# Supplementary material for: Security framework for quantum key distribution with imperfect sources
Source: arXiv:2305.05930 source file (2026-01-30)
Supplement: Supplementary file 1 [file supp.pdf]

## SUPPLEMENTARY INFORMATION

|                                                                                               |            |
|-----------------------------------------------------------------------------------------------|------------|
| <b>Supplementary Methods</b>                                                                  | <b>S3</b>  |
| SM1. Security proof for prepare-and-measure protocols                                         | S3         |
| A. Protocol description, assumptions, and security framework                                  | S3         |
| 1. Protocol description                                                                       | S3         |
| 2. Assumptions                                                                                | S4         |
| 3. Security framework                                                                         | S5         |
| B. Security proof for a particular three-state scenario                                       | S6         |
| 1. Constructing the loss-tolerant quantum coin state                                          | S6         |
| 2. Overview of the next steps in the security proof                                           | S7         |
| 3. Tag assignment                                                                             | S8         |
| 4. Coin Protocol                                                                              | S11        |
| C. Security proof for a particular BB84 scenario                                              | S14        |
| 1. Security analysis                                                                          | S14        |
| 2. Investigating how tight is our security proof                                              | S16        |
| 3. Reduction to the original quantum coin analysis when there are no qubit flaws              | S17        |
| D. General analysis for prepare-and-measure protocols                                         | S18        |
| E. General finite-key analysis for prepare-and-measure protocols                              | S22        |
| 1. Concentration inequalities                                                                 | S22        |
| 2. Analysis for a general prepare-and-measure protocol                                        | S23        |
| 3. Secret-key rate for a particular BB84 scenario                                             | S25        |
| SM2. Security proof for MDI-type protocols                                                    | S26        |
| A. Protocol description, assumptions and security framework                                   | S26        |
| 1. Protocol description                                                                       | S26        |
| 2. Assumptions                                                                                | S27        |
| 3. Security framework                                                                         | S27        |
| B. Constructing the reference and target states, and the Virtual Protocol with tag assignment | S28        |
| C. Coin protocol                                                                              | S30        |
| D. General finite-key analysis for MDI protocols                                              | S31        |
| SM3. Security analysis for non-IID sources                                                    | S32        |
| A. Independent but not identical pure states                                                  | S32        |
| B. Independent but not identical mixed states                                                 | S32        |
| C. Setting-independent pulse correlations                                                     | S33        |
| D. Setting-dependent pulse correlations                                                       | S33        |
| SM4. Security with WCP light sources                                                          | S35        |
| A. Coherent-light-based MDI protocol                                                          | S36        |
| 1. Protocol description                                                                       | S36        |
| 2. Security analysis                                                                          | S37        |
| 3. Finite-key analysis                                                                        | S42        |
| B. Decoy-state protocols                                                                      | S44        |
| 1. Ideal PR-WCP light sources                                                                 | S44        |
| 2. Realistic PR-WCP light sources                                                             | S45        |
| SM5. Why our security proof does not require the sequential assumption                        | S46        |
| A. Ensuring sequentiality by restricting the repetition rate                                  | S47        |
| SM6. Recipe for experimentalists                                                              | S48        |
| <b>Supplementary Equations</b>                                                                | <b>S50</b> |

|                                                                 |     |
|-----------------------------------------------------------------|-----|
| SE1. Proof of the quantum coin inequality                       | S50 |
| A. Prepare-and-measure scenario                                 | S50 |
| B. Measurement-device-independent scenario                      | S53 |
| SE2. Obtaining a bound on the coin imbalance parameter $\Delta$ | S53 |
| A. Three-state protocol                                         | S54 |
| 1. Numerical bound using SDP techniques                         | S54 |
| 2. Analytical bound with an additional assumption               | S55 |
| 3. Comparison between the numerical and analytical bounds       | S55 |
| B. Coherent-light-based MDI protocol                            | S55 |
| SE3. Channel model                                              | S57 |
| A. Prepare-and-measure protocol                                 | S57 |
| B. Coherent-light-based MDI protocol                            | S58 |
| SE4. High-level description of the code                         | S59 |
| <b>Supplementary Tables</b>                                     | S60 |
| <b>References</b>                                               | S62 |

## Supplementary Methods

In the Supplementary Methods, we present our security proof in detail. In Section SM1, we consider prepare-and-measure (P&M) protocols and in Section SM2, we consider measurement-device-independent (MDI) protocols. In Section SM3, we show how our security proof can be applied to scenarios in which the pulses emitted by the source are mixed and even correlated across different rounds, and in Section SM4, how it can be applied to scenarios in which the sources emit weak coherent pulses. In Section SM5, we present a key feature of our security proof, namely, why, unlike other analyses [S1, S2], it does not require the sequential assumption. Finally, in Section SM6, we present a simple step-by-step instruction list to apply our security proof to a practical QKD implementation. We remark that, for simplicity, throughout the Supplementary Information we denote the emitted quantum states by  $|\psi_j\rangle_B$  rather than  $|\psi_j(\epsilon)\rangle_B$ , the notation used in the Main Text.

### SM1. SECURITY PROOF FOR PREPARE-AND-MEASURE PROTOCOLS

#### A. Protocol description, assumptions, and security framework

##### 1. Protocol description

As explained in the Main Text, our security proof is applicable irrespective of whether Alice emits three or four different states  $\{|\psi_j\rangle_B\}_j$ . Without loss of generality, in the former (latter) case, we label these states as  $j \in \{0_Z, 1_Z, 0_X\}$  ( $j \in \{0_Z, 1_Z, 0_X, 1_X\}$ ). States such that  $j \in \{0_Z, 1_Z\}$  ( $j \notin \{0_Z, 1_Z\}$ ) are considered  $Z$ -basis ( $X$ -basis) states. For simplicity, the  $Z$ -basis states are assumed to be selected with probability  $p_{Z_A}/2$  each (see Section SE3 A in Supplementary Tables for a list of all probabilities). Also, in the three-state scenario, Alice selects the  $X$ -basis state  $j = 0_X$  with probability  $p_{X_A} := 1 - p_{Z_A}$ ; while in the four-state scenario, we assume that the  $X$ -basis states  $j \in \{0_X, 1_X\}$  are selected with probability  $p_{X_A}/2$  each.

---

#### Actual Protocol

1. **Quantum communication:** For each of the  $N$  rounds: (a) Alice probabilistically chooses a state  $\{|\psi_j\rangle_B\}_j$  and sends it to Bob through a quantum channel. (b) Bob chooses the positive operator-valued measure (POVM)  $\mathcal{Z}$  ( $\mathcal{X}$ ) with probability  $p_{Z_B}$  ( $p_{X_B}$ ), measures the incoming state and, if he obtains a detection (i.e., a bit value, rather than an inconclusive outcome), he announces this fact.
  2. **Basis and bit announcement:** Alice and Bob reveal their basis choices in the detected rounds. Then, they define the detected key rounds as the detected rounds in which both chose the  $Z$  basis, and their sifted keys as the bit outcomes of these rounds. Also, they evaluate its length  $N_{\text{key}}^{\text{det}}$ . Then, they define the detected test rounds as the detected rounds in which Bob used the  $X$  basis. For each of these rounds, Bob reveals his bit outcome, and Alice reveals her setting choice  $j$ .
  3. **Parameter estimation:** Alice and Bob quantify the number of events  $N_j^{\beta_X}$  for  $\beta \in \{0, 1\}$ , i.e., the number of instances in which Alice emitted the state  $|\psi_j\rangle_B$  and Bob obtained the measurement result  $\beta_X$ . Then, they use this information to obtain an upper bound on the phase-error rate  $e_{\text{ph}}$  of the sifted key.
  4. **Data post-processing:** Alice sends Bob syndrome information about her sifted key through an authenticated classical channel for him to correct his own sifted key. After, Alice and Bob perform error verification by computing a hash of their corrected keys using a random two-universal hash function and then check whether they are identical. If so, Alice and Bob perform privacy amplification by employing a random two-universal hash function to extract a secure key pair from the corrected keys. Otherwise, they abort the protocol.
- 

For simplicity, we assume that, in Step 4, Alice and Bob perform error correction for a predetermined bit-error rate, which is inferred from *a priori* knowledge of the channel. After, they perform error verification, learning whether or not the actual bit-error rate exceeded the predetermined one. Alternatively, Alice and Bob could sacrifice a small fraction of their sifted key to estimate its bit-error rate, and then select an appropriate error correcting code. This would require minor changes in the security proof, but its essence would remain the same. Also, we remark that during Step 1 of the Actual Protocol, Eve can perform the most general attack allowed by quantum mechanics on all of the transmitted signals at once. Indeed, our security proof does not rely on an independent and identically distributed (IID) assumption or on a sequential assumption. For more details on why this is the case, see Section SM5.

## 2. Assumptions

(A1) *Bounded fidelity to qubit states:* Alice's emitted states  $\{|\psi_j\rangle_B\}_j$  are  $\epsilon$ -close (in terms of fidelity) to some characterized qubit states  $\{|\phi_j\rangle_B\}_j$ , i.e., for all  $j$ ,

$$|\langle\phi_j|\psi_j\rangle_B|^2 \geq 1 - \epsilon, \quad (\text{S1})$$

where  $\epsilon$  is known<sup>1</sup>. For notational simplicity, we consider throughout the proof that the states emitted by Alice are pure and identical for all rounds. However, as explained in the Main Text and Methods, our security analysis can be trivially extended without any modifications to the scenario in which Alice's states are mixed and/or different for different rounds (see Eq. (1) in the Main Text). Moreover, with a simple modification to Eq. (S1) and to the post-processing step of the protocol, our analysis can be applied in the presence of setting-dependent pulse correlations i.e., when the state emitted in a given round depends on the setting choices made in previous rounds. For more information, see Section SM3.

**Claim.** As a consequence of Eq. (S1), we can assume that the emitted states are

$$|\psi_j\rangle_B = \sqrt{1 - \epsilon} |\phi_j\rangle_B + \sqrt{\epsilon} |\phi_j^\perp\rangle_B, \quad (\text{S2})$$

where  $|\phi_j^\perp\rangle_B$  is a state such that  $\langle\phi_j|\phi_j^\perp\rangle_B = 0$ , since this never underestimates the information available to Eve.

*Proof of Claim.* Without loss of generality, Eq. (S1) implies that the emitted states can be expressed as

$$|\psi_j\rangle_B = e^{i\varphi_j} (\sqrt{1 - \epsilon_j} |\phi_j\rangle_B + \sqrt{\epsilon_j} |\phi_j^\perp\rangle_B), \quad (\text{S3})$$

where  $\epsilon_j \leq \epsilon$  and  $\varphi_j \in [0, 2\pi)$ . However, since the global phases  $\varphi_j$  have no physical meaning, we can take  $\varphi_j = 0$  and write Eq. (S3) as

$$|\psi_j\rangle_B = \sqrt{1 - \epsilon_j} |\phi_j\rangle_B + \sqrt{\epsilon_j} |\phi_j^\perp\rangle_B. \quad (\text{S4})$$

Now, we show that, in Eq. (S4), we can simply consider that  $\epsilon_j = \epsilon$ . For this, suppose that instead of preparing  $\{|\psi_j\rangle_B\}_j$  in Eq. (S4), Alice first generates the states  $\{|\psi_j\rangle_{BF}\}_j$ :

$$|\psi_j\rangle_{BF} = |\psi_j\rangle_B \otimes \left[ \frac{\sqrt{1 - \epsilon}}{\sqrt{1 - \epsilon_j}} |0\rangle_F + \sqrt{1 - \frac{1 - \epsilon}{1 - \epsilon_j}} |1\rangle_F \right], \quad (\text{S5})$$

where  $\{|0\rangle_F, |1\rangle_F\}$  forms an orthonormal basis, and then emits system  $B$ . In both scenarios, the states that Eve observes are the same, and therefore they are equivalent. We can then rewrite Eq. (S5) as

$$|\psi_j\rangle_{BF} = \sqrt{1 - \epsilon} |\phi_j\rangle_{BF} + \sqrt{\epsilon} |\phi_j^\perp\rangle_{BF}, \quad (\text{S6})$$

where we have defined  $|\phi_j\rangle_{BF} := |\phi_j\rangle_B |0\rangle_F$  and  $\langle\phi_j|\phi_j^\perp\rangle_{BF} = 0$ . If we assume that Eve also has access to the fictitious system  $F$ , which never underestimates her side information, and rename systems  $BF$  as simply  $B$ , we obtain Eq. (S2), as required. The advantage of Eq. (S2) with respect to Eq. (S4) is that, in the former, the coefficient of the qubit state  $|\phi_j\rangle_B$  is known exactly, which is needed to run the semidefinite program (SDP) in Section SE2.  $\square$

(A2) *Basis-independent detection efficiency:* Bob's POVMs can be expressed as  $\mathcal{Z} := \{\hat{m}_{0_Z}, \hat{m}_{1_Z}, \hat{m}_f\}$  and  $\mathcal{X} := \{\hat{m}_{0_X}, \hat{m}_{1_X}, \hat{m}_f\}$ , where  $\hat{m}_f$  is associated with an inconclusive outcome. That is, the probability that Bob obtains a successful detection is independent of his basis choice, regardless of the state that arrives to his measurement device. For later convenience, we define  $\hat{m}_{\text{det}} = \hat{\mathbb{I}} - \hat{m}_f$ . Also, we assume that there are no side channels on Bob's devices. We remark that, due to the feasibility of attacks that can control the behavior of the detectors [S3–S6], no existing security analysis can achieve information-theoretic security against general detector side channels, and in fact achieving this at the security-proof level may be an unrealistic goal. Fortunately, this issue can be avoided by considering an MDI-type protocol [S7], for which our analysis can be applied to close vulnerabilities and side channels for both Alice and Bob's sources (see Section SM2).

<sup>1</sup> For simplicity, we have considered that  $\epsilon$  is independent of  $j$ , but our security proof can be equally applied when its value is different for different  $j$ . Also, as explained in Methods, our security proof can be applied under the more general assumption that  $|\langle\phi_j|\psi_j\rangle_B|^2 \geq 1 - \epsilon$ , where  $\{|\phi_j\rangle_B\}_j$  any characterized states, not necessarily qubits.

### 3. Security framework

The sifted key is generated from the detected key rounds, i.e., the detected rounds in which both Alice and Bob selected the  $Z$  basis. Note that, in these rounds, instead of emitting  $\{|\psi_{0Z}\rangle_B, |\psi_{1Z}\rangle_B\}$ , Alice could have generated the entangled state

$$|\Psi_Z\rangle_{AB} = \frac{1}{\sqrt{2}}(|0_Z\rangle_A |\psi_{0Z}\rangle_B + e^{i\omega} |1_Z\rangle_A |\psi_{1Z}\rangle_B), \quad (\text{S7})$$

where  $\omega = [0, 2\pi)$  can be freely chosen, and then measured the ancillary system  $A$  in the  $Z$  basis. Due to Assumption (A2), the amount of privacy amplification that needs to be applied to the sifted key to turn it into a secret key can be directly related to the error rate that Alice and Bob would have observed if, in these rounds, Alice had measured system  $A$  in the  $X$  basis and Bob had used the  $\mathcal{X}$  POVM, i.e., the phase-error rate  $e_{\text{ph}}$ . For this estimation, it is useful to rewrite Eq. (S7) as

$$|\Psi_Z\rangle_{AB} = \sqrt{q_{\text{vir0}}^\psi} |0_X\rangle_A |\psi_{\text{vir0}}\rangle_B + e^{i\omega} \sqrt{q_{\text{vir1}}^\psi} |1_X\rangle_A |\psi_{\text{vir1}}\rangle_B, \quad (\text{S8})$$

where

$$\begin{aligned} |\psi_{\text{vir0}}\rangle_B &= \frac{1}{2\sqrt{q_{\text{vir0}}^\psi}} (|\psi_{0Z}\rangle_B + e^{i\omega} |\psi_{1Z}\rangle_B), \\ |\psi_{\text{vir1}}\rangle_B &= \frac{1}{2\sqrt{q_{\text{vir1}}^\psi}} (|\psi_{0Z}\rangle_B - e^{i\omega} |\psi_{1Z}\rangle_B), \end{aligned} \quad (\text{S9})$$

with

$$\begin{aligned} q_{\text{vir0}}^\psi &= \frac{1}{4} \| |\psi_{0Z}\rangle_B + e^{i\omega} |\psi_{1Z}\rangle_B \|^2 = \frac{1}{2} (1 + \text{Re } e^{i\omega} \langle \psi_{0Z} | \psi_{1Z} \rangle_B), \\ q_{\text{vir1}}^\psi &= \frac{1}{4} \| |\psi_{0Z}\rangle_B - e^{i\omega} |\psi_{1Z}\rangle_B \|^2 = \frac{1}{2} (1 - \text{Re} \{ e^{i\omega} \} \langle \psi_{0Z} | \psi_{1Z} \rangle_B). \end{aligned} \quad (\text{S10})$$

Thus, the scenario described above is equivalent to a protocol in which, in the key rounds, Alice emits the *virtual* states  $|\psi_{\text{vir0}}\rangle_B$  ( $|\psi_{\text{vir1}}\rangle_B$ ) with probability  $q_{\text{vir0}}^\psi$  ( $q_{\text{vir1}}^\psi$ ), and Bob uses the  $\mathcal{X}$  POVM; we refer to this scenario as the Virtual Protocol (see full description below). We remark that, for clarity, throughout the Supplementary Information we use  $q_{\text{vir0}}^\psi$  ( $q_{\text{vir1}}^\psi$ ) to denote the probability  $1 - q_\epsilon$  ( $q_\epsilon$ ), the notation used in the Main Text.

In this Virtual Protocol, the phase-error rate can be expressed as  $e_{\text{ph}} := N_{\text{ph}}/N_{\text{key}}^{\text{det}}$ , where  $N_{\text{ph}} := N_{\text{vir0}}^{1X} + N_{\text{vir1}}^{0X}$  is the number of phase errors, and  $N_{\text{vir}\alpha}^{\beta X}$  is the number of events in which Alice emits  $|\psi_{\text{vir}\alpha}\rangle_B$  and Bob obtains the measurement result  $\beta_X$ , with  $\alpha, \beta \in \{0, 1\}$  (see Table S1 in Supplementary Tables for a list of all random variables). The objective of our security analysis is then to find a bound of the form

$$N_{\text{ph}} \leq f(\{N_j^{\beta X}\}_{j,\beta}, N_{\text{key}}^{\text{det}}) =: N_{\text{ph}}^{\text{U}}, \quad (\text{S11})$$

with a failure probability approaching zero exponentially fast as the number of detected rounds increases, and consequently be able to upper bound the phase-error rate as  $e_{\text{ph}}^{\text{U}} := N_{\text{ph}}^{\text{U}}/N_{\text{key}}^{\text{det}}$ .

---

#### Virtual Protocol

1. **Quantum communication:** For each of the  $N$  rounds: (a) With probability  $p_{ZA}p_{ZB}$ , the round is a key round. If so, Alice emits  $|\psi_{\text{vir0}}\rangle_B$  ( $|\psi_{\text{vir1}}\rangle_B$ ) with probability  $q_{\text{vir0}}^\psi$  ( $q_{\text{vir1}}^\psi$ ), and Bob uses the  $\mathcal{X}$  POVM to measure the incoming signal. (b) With probability  $p_{XB}$ , the round is a test round. If so, Alice emits  $\{|\psi_j\rangle_B\}_j$  with the same probabilities as in the Actual Protocol and Bob uses the  $\mathcal{X}$  POVM to measure the incoming signal. (c) With probability  $p_{XA}p_{ZB}$ , Alice emits some state  $|\psi_j\rangle_B$  such that  $j \notin \{0_Z, 1_Z\}$  and Bob measures the incoming signal using the  $Z$  POVM. As in the Actual Protocol (see Section SM1 A 1), whenever Bob obtains a successful detection, he announces it.
  2. **Basis and bit announcement:** Alice and Bob reveal their basis choices in the detected rounds. In particular, for the key rounds, Bob announces the  $Z$  basis even though he uses the  $\mathcal{X}$  POVM. This ensures that the announcements in the Virtual Protocol match those in the Actual Protocol. For the test rounds, Bob reveals his bit outcome, and Alice reveals her setting choice  $j$ .
-

Note that, from Eve's perspective, the Virtual Protocol is completely equivalent to Steps 1 and 2 in the Actual Protocol. This is because all quantum and classical information available to her is identical in both protocols<sup>2</sup>. Also, note that the Virtual Protocol is merely a mathematical tool that is used to prove security, and there is no need to implement it in reality.

### B. Security proof for a particular three-state scenario

As explained in the Main Text, our approach to obtain  $e_{\text{ph}}^{\text{U}}$  relies on the construction of a loss-tolerant quantum coin state. The exact form of this quantum coin state, and the resulting phase-error rate bound, depends on the form of the states  $\{|\phi_j\rangle_B\}_j$ . In this Section, we explain all the ideas in our security proof in detail by applying it to a particular three-state scenario in which these states are

$$|\phi_j\rangle_B = \cos(\theta_j) |0_Z\rangle_B + \sin(\theta_j) |1_Z\rangle_B, \quad (\text{S12})$$

for  $j \in \{0_Z, 1_Z, 0_X\}$ . Here,  $\{|0_Z\rangle_B, |1_Z\rangle_B\}$  forms a qubit basis, and

$$\theta_{0_Z} = 0, \quad \theta_{1_Z} = \kappa\pi/2, \quad \theta_{0_X} = \kappa\pi/4, \quad (\text{S13})$$

with  $\kappa = 1 + \delta/\pi$ , and where  $\delta \in [0, \pi)$  quantifies the magnitude of the qubit flaws. Also, for simplicity, in this Section, we assume the asymptotic regime. In Section SM1 D, we present a general analysis that is valid for any  $\{|\phi_j\rangle_B\}_j$  and in Section SM1 E, we extend it to the finite-key regime. However, we recommend reading this Section first, as the ideas behind our security proof are explained in much more detail here.

#### 1. Constructing the loss-tolerant quantum coin state

To construct the quantum coin state, we need to appropriately define the target and reference states. For this, we first consider the scenario  $\epsilon = 0$  and employ the loss-tolerant (LT) analysis [S14] to find relationships between the virtual and qubit states. For the states in Eq. (S12), these are [S15]

$$|\phi_{\text{vir}0}\rangle\langle\phi_{\text{vir}0}|_B = |\phi_{0_X}\rangle\langle\phi_{0_X}|_B, \quad (\text{S14})$$

$$c_2 |\phi_{0_X}\rangle\langle\phi_{0_X}|_B + |\phi_{\text{vir}1}\rangle\langle\phi_{\text{vir}1}|_B = c_1 |\phi_{0_Z}\rangle\langle\phi_{0_Z}|_B + c_1 |\phi_{1_Z}\rangle\langle\phi_{1_Z}|_B, \quad (\text{S15})$$

where

$$\begin{aligned} c_1 &:= \frac{1}{2 \sin^2(\kappa\pi/4)} \in (1/2, 1], \\ c_2 &:= 2c_1 - 1 \in (0, 1], \end{aligned} \quad (\text{S16})$$

and

$$\begin{aligned} |\phi_{\text{vir}0}\rangle_B &= \frac{1}{2\sqrt{q_{\text{vir}0}^\phi}} (|\phi_{0_Z}\rangle_B + |\phi_{1_Z}\rangle_B), \\ |\phi_{\text{vir}1}\rangle_B &= \frac{1}{2\sqrt{q_{\text{vir}1}^\phi}} (|\phi_{0_Z}\rangle_B - |\phi_{1_Z}\rangle_B), \end{aligned} \quad (\text{S17})$$

with

$$\begin{aligned} q_{\text{vir}0}^\phi &= \frac{1}{2} (1 + \text{Re} \langle \phi_{0_Z} | \phi_{1_Z} \rangle_B) = \frac{1}{2c_1}, \\ q_{\text{vir}1}^\phi &= \frac{1}{2} (1 - \text{Re} \langle \phi_{0_Z} | \phi_{1_Z} \rangle_B) = \frac{2c_1 - 1}{2c_1}. \end{aligned} \quad (\text{S18})$$

---

<sup>2</sup> Although the Virtual Protocol cannot output the information that is available to Eve in Step 4 of the Actual Protocol, the parameter estimation (i.e., the phase-error rate estimation) established in the Virtual Protocol can be directly used to determine the amount of privacy amplification required in the Actual Protocol [S8–S13].

Note that Eqs. (S17) and (S18) are analogous to Eqs. (S9) and (S10) after taking  $\omega = 0$  and substituting the actual  $Z$  basis states  $|\psi_{0z}\rangle_B$  and  $|\psi_{1z}\rangle_B$  by their respective qubit components  $|\phi_{0z}\rangle_B$  and  $|\phi_{1z}\rangle_B$ . We remark that, for clarity, throughout the Supplementary Information we use  $q_{\text{vir}0}^\phi$  ( $q_{\text{vir}1}^\phi$ ) to denote the probability  $1 - q_0$  ( $q_0$ ), the notation used in the Main Text.

When  $\epsilon \gtrsim 0$ , namely, in the presence of side channels, the equalities in Eqs. (S14) and (S15) do not hold exactly, but still hold approximately, i.e.,

$$|\psi_{\text{vir}0}\rangle\langle\psi_{\text{vir}0}|_B \approx |\psi_{0x}\rangle\langle\psi_{0x}|_B, \quad (\text{S19})$$

$$c_2 |\psi_{0x}\rangle\langle\psi_{0x}|_B + |\psi_{\text{vir}1}\rangle\langle\psi_{\text{vir}1}|_B \approx c_1 |\psi_{0z}\rangle\langle\psi_{0z}|_B + c_1 |\psi_{1z}\rangle\langle\psi_{1z}|_B. \quad (\text{S20})$$

Taking advantage of this fact, we define  $|\Psi_{\text{Tar}}\rangle_{DAB}$  and  $|\Psi_{\text{Ref}}\rangle_{DAB}$  in the following way

$$|\Psi_{\text{Tar}}\rangle_{DAB} = \frac{1}{\sqrt{1 + c_2 q_{\text{vir}1}^\phi}} \left[ \sqrt{q_{\text{vir}0}^\psi} |0\rangle_D |0\rangle_A |\psi_{\text{vir}0}\rangle_B + |1\rangle_D \left( \sqrt{c_2 q_{\text{vir}1}^\phi} |0'\rangle_A |\psi_{0x}\rangle_B + \sqrt{q_{\text{vir}1}^\psi} |1'\rangle_A |\psi_{\text{vir}1}\rangle_B \right) \right], \quad (\text{S21})$$

$$|\Psi_{\text{Ref}}\rangle_{DAB} = \frac{1}{\sqrt{1 + c_2 q_{\text{vir}1}^\phi}} \left[ \sqrt{q_{\text{vir}0}^\phi} |0\rangle_D |0\rangle_A |\psi_{0x}\rangle_B + \sqrt{c_1 q_{\text{vir}1}^\phi} |1\rangle_D (|0\rangle_A |\psi_{0z}\rangle_B + |1\rangle_A |\psi_{1z}\rangle_B) \right]. \quad (\text{S22})$$

In Eq. (S21), the orthonormal basis  $\{|0'\rangle_A, |1'\rangle_A\}$  has been chosen such that

$$\sqrt{c_2} |0'\rangle_A |\phi_{0x}\rangle_B + |1'\rangle_A |\phi_{\text{vir}1}\rangle_B = \sqrt{c_1} (|0\rangle_A |\phi_{0z}\rangle_B + |1\rangle_A |\phi_{1z}\rangle_B), \quad (\text{S23})$$

which must exist due to the equality in Eq. (S15) and Uhlmann's theorem, and can be calculated to be

$$\begin{aligned} |0'\rangle_A &= \frac{1}{\sqrt{2}}(|0\rangle_A + |1\rangle_A), \\ |1'\rangle_A &= \frac{1}{\sqrt{2}}(|0\rangle_A - |1\rangle_A). \end{aligned} \quad (\text{S24})$$

Note that  $|\Psi_{\text{Tar}}\rangle_{DAB} = |\Psi_{\text{Ref}}\rangle_{DAB}$  when  $\epsilon = 0$ , which ensures the robustness of our phase-error rate bound against qubit flaws; and that, in Eq. (S21), the coefficient of the state  $|\psi_{\text{vir}0}\rangle_B$  ( $|\psi_{\text{vir}1}\rangle_B$ ) is proportional to  $\sqrt{q_{\text{vir}0}^\psi}$  ( $\sqrt{q_{\text{vir}1}^\psi}$ ). Therefore, the target and reference states in Eq. (S21) and Eq. (S22) fulfill the requirements described in Methods for the definition of these states. Our particular choice in Eqs. (S21) and (S22) uses  $q_{\text{vir}\alpha}^\phi$  rather than  $q_{\text{vir}\alpha}^\psi$  everywhere except in the coefficients of the virtual states. This is advantageous because it will lead to a phase-error rate bound that depends on  $q_{\text{vir}\alpha}^\phi$ , which is known exactly, rather than  $q_{\text{vir}\alpha}^\psi$ , which is not (see Eq. (S46) below). This avoids having to use numerical optimization to find the worst-case scenario for  $q_{\text{vir}\alpha}^\psi$  in this expression. Finally, we define the loss-tolerant quantum coin state as (see the Main Text for more details)

$$|\Psi_{\text{coin}}\rangle_{CDAB} = \frac{1}{\sqrt{2}} (|0z\rangle_C |\Psi_{\text{Tar}}\rangle_{DAB} + |1z\rangle_C |\Psi_{\text{Ref}}\rangle_{DAB}), \quad (\text{S25})$$

where system  $C$  is held by Alice, and therefore inaccessible to Eve.

## 2. Overview of the next steps in the security proof

Let us assume that Alice generates many copies of Eq. (S25), sends all systems  $B$  to Bob through the Eve-controlled quantum channel, and then probabilistically decides whether to measure each coin system  $C$  in the  $Z$  basis or  $X$  basis. Also, Alice and Bob perform a joint POVM containing the element  $\hat{m}_{\text{err}} = |0\rangle\langle 0|_D \otimes \hat{m}_{1x} + |1\rangle\langle 1|_D \otimes \hat{m}_{0x}$ . Let  $N_{ZC=0}^{\text{err}}$  ( $N_{ZC=1}^{\text{err}}$ ) be the number of events in which Alice chooses the  $Z$  basis to measure the coin system  $C$ , obtains the result  $Z_C = 0$  ( $Z_C = 1$ ), and Alice and Bob obtain the outcome associated to  $\hat{m}_{\text{err}}$ . Note that  $N_{ZC=0}^{\text{err}}$  contains events in which Alice emits  $|\psi_{\text{vir}0}\rangle_B$  ( $|\psi_{\text{vir}1}\rangle_B$ ) and Bob obtains measurement outcome  $1_x$  ( $0_x$ ), i.e., phase errors; and that both  $N_{ZC=0}^{\text{err}}$  and  $N_{ZC=1}^{\text{err}}$  contain events in which Alice emits some actual state  $|\psi_j\rangle_B$  and Bob obtains a measurement outcome  $\beta_x$ , whose detection statistics can be observed in the Actual Protocol. These facts allow us to use the quantum coin idea to obtain a bound on the number of phase errors in the Virtual Protocol. More precisely, using the quantum coin inequality (see Section SE1 for more details), we can bound the deviation between  $N_{ZC=0}^{\text{err}}$  and  $N_{ZC=1}^{\text{err}}$

by a function of  $N_{X_C=1}$ , the overall number of events, detected or not, in which Alice obtained  $X_C = 1$ . In turn,  $N_{X_C=1}$  can be estimated by bounding the *a priori* probability that Alice obtains  $X_C = 1$  in her measurement of the quantum coin, as discussed in the Main Text.

However, to use the quantum coin idea, we first need to deal with the fact that the generation of the quantum coin state in Eq. (S25) is not directly equivalent to Alice’s state preparation in the Virtual Protocol, and therefore the quantum coin inequality is not directly applicable to the latter scenario. This is because the probability that Alice emits a particular state in the Virtual Protocol differs from the probability that Alice “emits” this state when she generates the quantum coin. For example, the probability that Alice emits the state  $|\psi_{0_Z}\rangle_B$  in the Virtual Protocol is  $p_{Z_A}p_{X_B}/2$ , while the probability that Alice “emits”  $|\psi_{0_Z}\rangle_B$  when she generates the quantum coin is  $q_{\text{vir1}}^\phi c_1/(2 + 2c_2q_{\text{vir1}}^\phi)$ . In general, it is not possible to select  $p_{Z_A}$  and  $p_{Z_B}$  such that these probabilities coincide for all states. To address this, we consider a slight modification to the Virtual Protocol. Namely, we consider that, after the quantum communication step, Alice probabilistically assigns tags to her emissions, in such a way that emissions that receive a tag can be regarded as equivalent to those originating from the quantum coin state in Eq. (S25). This allows us to draw an equivalence between the Virtual Protocol and a scenario in which Alice sometimes generates this quantum coin state, which we denote as the Coin Protocol. More specifically, tagged rounds in the former scenario correspond to coin rounds (i.e., rounds in which the quantum coin state is generated) in the latter, see Fig. S1. Thanks to this correspondence, we are able to apply the quantum coin inequality described above to obtain a bound on the number of phase errors within the tagged rounds. Finally, by using the fact that Alice’s tag assignment is independent between rounds, and is independent of Bob’s measurement outcomes (because it does not affect the emitted quantum state), we combine this result with known random sampling inequalities to obtain a bound on the total number of phase errors. We note that, since the outcomes of the tag assignment step are statistically estimated, Alice does not actually need to perform this tag assignment step in the Actual Protocol; the mere fact that she could have done so is enough for the idea to work.

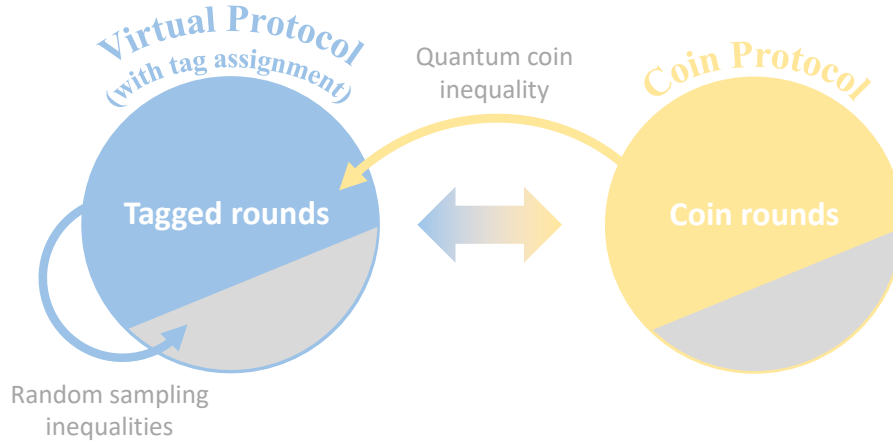

Figure S1. Overview of the phase-error rate estimation. After adding a fictitious tag assignment step to the Virtual Protocol, the tagged rounds can be seen as equivalent to the generation of the quantum coin state  $|\Psi_{\text{coin}}\rangle_{CDAB}$  in Eq. (S25). This allows us to use the quantum coin inequality to derive a bound on the number of phase errors within the tagged rounds. Then, we obtain a bound on the total number of phase errors by combining this result with random sampling inequalities.

### 3. Tag assignment

As explained in Section SM1 B 2, to find an equivalence between the Virtual Protocol and the Coin Protocol, we consider the addition of a fictitious tag assignment step to the former, such that tagged emissions can be regarded as equivalent to those originating from the loss-tolerant quantum coin state in Eq. (S25). Let  $l \in \{\text{vir0}, \text{vir1}, 0_Z, 1_Z, 0_X, 0_X^*\}$  denote Alice and Bob’s joint selection in Step 1 of the Virtual Protocol, where  $l = 0_X$  ( $0_X^*$ ) denotes an event in which Alice emits  $|\psi_{0_X}\rangle_B$  and Bob chooses the  $X$  ( $Z$ ) basis, and the rest of the events are self-descriptive. The probability  $p_l$  associated to each event in the Virtual Protocol is

$$\begin{aligned}
p_{\text{vir}0} &= q_{\text{vir}0}^\psi p_{Z_A} p_{Z_B}, \\
p_{\text{vir}1} &= q_{\text{vir}1}^\psi p_{Z_A} p_{Z_B}, \\
p_{0_Z} &= p_{1_Z} = \frac{1}{2} p_{Z_A} p_{X_B}, \\
p_{0_X} &= p_{X_A} p_{X_B}, \\
p_{0_X^*} &= p_{X_A} p_{Z_B}.
\end{aligned} \tag{S26}$$

The events  $l = 0_X^*$  are irrelevant for the analysis, because Bob's  $Z$ -basis measurement results do not help to estimate the phase-error rate, and in the following we assume  $l \in \{\text{vir}0, \text{vir}1, 0_Z, 1_Z, 0_X\}$ . We can define the additional tag assignment step, which is performed after Step 1 of the Virtual Protocol, as:

---

**1.5. Tag assignment:** For each event  $l \in \{\text{vir}0, \text{vir}1, 0_Z, 1_Z, 0_X\}$ , Alice assigns it a single tag  $t \in \{\text{TAR}, \text{REF}\}$  with probability  $p_{t|l}$ , or no tag with probability  $1 - \sum_t p_{t|l}$ . Then, for the tagged events, Alice marks (i.e., takes note of) each emission as  $Z_C$  ( $X_C$ ) with probability  $p_{Z_C}$  ( $p_{X_C} = 1 - p_{Z_C}$ ).

---

The conditional tag assignment probabilities  $\{p_{t|l}\}$  should be chosen carefully, such that an emission with a tag **TAR** (**REF**) is equivalent to that originating from the state  $|\Psi_{\text{TAR}}\rangle_{DAB}$  ( $|\Psi_{\text{REF}}\rangle_{DAB}$ ). Also, since the coefficients associated with  $|\Psi_{\text{TAR}}\rangle_{DAB}$  and  $|\Psi_{\text{REF}}\rangle_{DAB}$  in Eq. (S25) are identical, the overall probability of assigning both tags must also be identical, i.e.,  $p_{\text{TAR}} = p_{\text{REF}}$ . By doing so, an emission with a tag **TAR** or **REF** can be regarded as equivalent to that originating from the state  $|\Psi_{\text{coin}}\rangle_{CDAB}$ . In addition, Alice probabilistically marks each tagged emission as  $Z_C$  or  $X_C$ . These correspond to rounds in which, in the Coin Protocol, Alice measures the quantum coin system  $C$  in the  $Z_C$  or  $X_C$  basis, respectively. In Fig. S2, we depict the Virtual Protocol before and after the tag assignment step. For the latter, we have reordered emissions according to their tag  $t$  and mark ( $Z_C$  or  $X_C$ ), which helps represent its equivalence with the Coin Protocol, shown on the right.

Let us rewrite the states  $|\Psi_{\text{TAR}}\rangle_{DAB}$  and  $|\Psi_{\text{REF}}\rangle_{DAB}$  in Eqs. (S21) and (S22) as

$$\begin{aligned}
|\Psi_{\text{TAR}}\rangle_{DAB} &= \sqrt{p_{\text{vir}0|\text{TAR}}} |0\rangle_D |0\rangle_A |\psi_{\text{vir}0}\rangle_B + |1\rangle_D (\sqrt{p_{0_X|\text{TAR}}} |0'\rangle_A |\psi_{0_X}\rangle_B + \sqrt{p_{\text{vir}1|\text{TAR}}} |1'\rangle_A |\psi_{\text{vir}1}\rangle_B), \\
|\Psi_{\text{REF}}\rangle_{DAB} &= \sqrt{p_{0_X|\text{REF}}} |0\rangle_D |0\rangle_A |\psi_{0_X}\rangle_B + |1\rangle_D (\sqrt{p_{0_Z|\text{REF}}} |0\rangle_A |\psi_{0_Z}\rangle_B + \sqrt{p_{1_Z|\text{REF}}} |1\rangle_A |\psi_{1_Z}\rangle_B),
\end{aligned} \tag{S27}$$

where

$$\begin{aligned}
p_{\text{vir}0|\text{TAR}} &= \frac{q_{\text{vir}0}^\psi}{1 + c_2 q_{\text{vir}1}^\phi}, \\
p_{0_X|\text{TAR}} &= \frac{c_2 q_{\text{vir}1}^\phi}{1 + c_2 q_{\text{vir}1}^\phi}, \\
p_{\text{vir}1|\text{TAR}} &= \frac{q_{\text{vir}1}^\psi}{1 + c_2 q_{\text{vir}1}^\phi}, \\
p_{0_X|\text{REF}} &= \frac{q_{\text{vir}0}^\phi}{1 + c_2 q_{\text{vir}1}^\phi}, \\
p_{0_Z|\text{REF}} &= p_{1_Z|\text{REF}} = \frac{c_1 q_{\text{vir}1}^\phi}{1 + c_2 q_{\text{vir}1}^\phi}.
\end{aligned} \tag{S28}$$

The tag assignment probabilities  $p_{t|l}$  should be chosen appropriately such that the probability that an emission with tag  $t$  originated from event  $l$ ,  $p_{l|t}$ , matches Eq. (S28). By Bayes' Theorem, we can express

$$p_{t|l} = \frac{p_t p_{l|t}}{p_l}, \tag{S29}$$

where  $p_l$  is the probability of event  $l$  and  $p_t$  is the overall probability to assign tag  $t$ . Note that the sets  $\{p_l\}$  and  $\{p_{l|t}\}$  are fixed and given by Eqs. (S26) and (S28), respectively. Therefore, the conditional tag assignment probabilities  $\{p_{t|l}\}$  become fixed once we fix  $p_{\text{TAR}}$  and  $p_{\text{REF}}$ , which should be such that  $p_{\text{TAR}} = p_{\text{REF}}$ , as explained above. Taking the

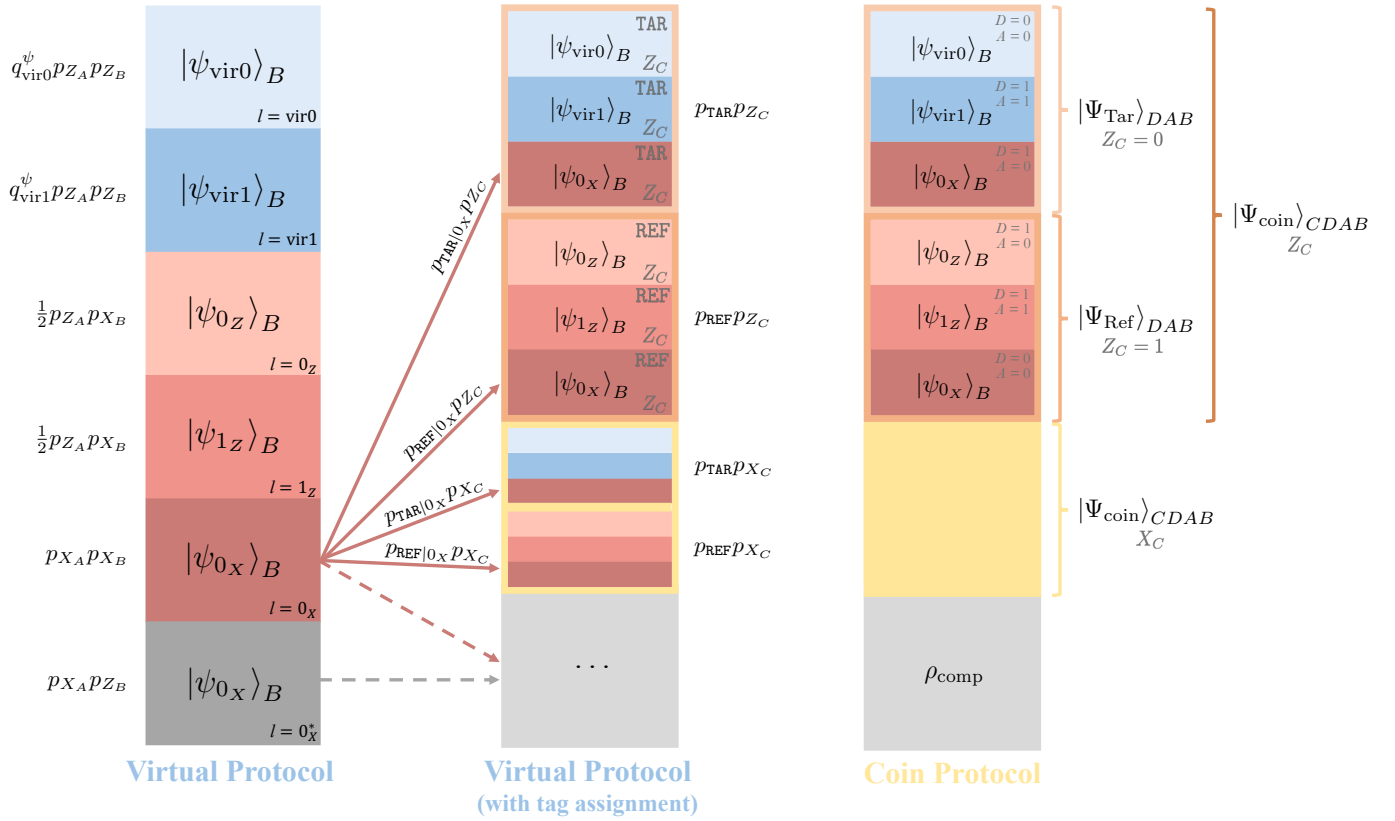

Figure S2. Equivalence between the Virtual Protocol and the Coin Protocol, after adding a fictitious tag assignment step to the former. As an example, this assignment is illustrated for the events  $l = 0_x$  using arrows, which are either tagged as  $t \in \{\text{TAR}, \text{REF}\}$  and marked as  $Z_C$  ( $X_C$ ) with probability  $p_{t|0_x p_{Z_C}}$  ( $p_{t|0_x p_{X_C}}$ ) (solid lines) or receive no tag (dashed line). The emissions with a tag **TAR** (**REF**) and marked with  $Z_C$ , which are enclosed by an orange square, are equivalent to those originating from the state  $|\Psi_{\text{Tar}}\rangle_{DAB}$  ( $|\Psi_{\text{Ref}}\rangle_{DAB}$ ). Also, when considered together, the two orange squares in the Virtual Protocol with tag assignment are equivalent to the generation of the quantum coin state  $|\Psi_{\text{coin}}\rangle_{CDAB}$ ; the same is true for the two yellow squares. Note that, in the  $Z_C$  rounds, Alice and Bob learn the same information in both protocols, while in the  $X_C$  rounds, they learn different information. The untagged rounds, and their equivalent compensation rounds, are marked in light gray.

sum over  $t \in \{\text{TAR}, \text{REF}\}$  on both sides of Eq. (S29) and using the fact that  $p_{\text{TAR}|l} + p_{\text{REF}|l} \leq 1$ , we derive the following constraints,

$$p_{\text{TAR}} p_{l|\text{TAR}} + p_{\text{REF}} p_{l|\text{REF}} \leq p_l, \quad \forall l. \quad (\text{S30})$$

The selected value of  $p_{\text{TAR}} = p_{\text{REF}}$  should be consistent with the above inequalities, i.e.,

$$p_{\text{TAR}} = p_{\text{REF}} \leq \min_l \frac{p_l}{p_{l|\text{TAR}} + p_{l|\text{REF}}}. \quad (\text{S31})$$

Substituting Eq. (S26) and Eq. (S28) into Eq. (S31) and simplifying, we obtain

$$p_{\text{TAR}} = p_{\text{REF}} \leq (1 + c_2 q_{\text{vir1}}^\phi) \min \left\{ p_{Z_A p_{Z_B}}, \frac{p_{X_A p_{X_B}}}{1 - (1 - c_2) q_{\text{vir1}}^\phi}, \frac{p_{Z_A p_{X_B}}}{2 c_1 q_{\text{vir1}}^\phi} \right\}, \quad (\text{S32})$$

and we can simply select  $p_{\text{TAR}}$  as the right-hand side of Eq. (S32). Also, substituting Eq. (S28) into Eq. (S29) and using the fact that  $p_{\text{TAR}} = p_{\text{REF}}$ , we obtain

$$\begin{aligned}
p_{\text{TAR}|\text{vir}} &:= p_{\text{TAR}|\text{vir}0} = p_{\text{TAR}|\text{vir}1} = \frac{p_{\text{TAR}}}{p_{Z_A} p_{Z_B} (1 + c_2 q_{\text{vir}1}^\phi)}, \\
p_{\text{TAR}|0_X} &= \frac{p_{\text{TAR}} c_2 q_{\text{vir}1}^\phi}{p_{X_A} p_{X_B} (1 + c_2 q_{\text{vir}1}^\phi)}, \\
p_{\text{REF}|0_X} &= \frac{p_{\text{TAR}} q_{\text{vir}0}^\phi}{p_{X_A} p_{X_B} (1 + c_2 q_{\text{vir}1}^\phi)}, \\
p_{\text{REF}|0_Z} = p_{\text{REF}|1_Z} &= \frac{2 p_{\text{TAR}} c_1 q_{\text{vir}1}^\phi}{p_{Z_A} p_{X_B} (1 + c_2 q_{\text{vir}1}^\phi)}.
\end{aligned} \tag{S33}$$

Note that these probabilities do not depend on  $q_{\text{vir}\alpha}^\psi$ , and therefore their exact value is known. This is a consequence of our choice of target and reference states in Eqs. (S21) and (S22).

### Random sampling relationships

Let  $N_l^{\beta_X}$  be the number of events  $l$  in which Bob obtained the measurement result  $\beta_X \in \{0_X, 1_X\}$ , and let  $N_{l,t,Z_C}^{\beta_X}$  be the number of events  $l$  with tag  $t$  marked as  $Z_C$  in which Bob obtained  $\beta_X$ . The probability that a given event  $l$  is assigned a tag  $t$  must be independent of Bob's measurement result for that round, since the tag assignment does not change the emitted quantum state, and Eve has no tag information. The same is true for the probability that the event is marked as  $Z_C$ . Therefore,  $N_{l,t,Z_C}^{\beta_X}$  is a random sample of a population of  $N_l^{\beta_X}$  events, where each event is selected with probability  $p_{Z_C} p_{t|l}$ . By the Chernoff bound [S16],

$$N_{l,t,Z_C}^{\beta_X} \simeq p_{Z_C} p_{t|l} N_l^{\beta_X}, \tag{S34}$$

where the symbol “ $\simeq$ ” denotes that the ratio between the left- and right-hand sides approaches one as  $N \rightarrow \infty$  (see Section SM1E for the analysis with a finite  $N$ ). Similarly, if we denote  $N_l^{\text{det}} = N_l^{0_X} + N_l^{1_X}$  and  $N_{l,t,Z_C}^{\text{det}} = N_{l,t,Z_C}^{0_X} + N_{l,t,Z_C}^{1_X}$ , we have that

$$N_{l,t,Z_C}^{\text{det}} \simeq p_{Z_C} p_{t|l} N_l^{\text{det}}. \tag{S35}$$

### 4. Coin Protocol

We are now ready to provide a full definition for the Coin Protocol. We remark that, in addition to coin rounds, this scenario also contains rounds in which the quantum coin state is not generated, which correspond to the untagged rounds in the Virtual Protocol with tag assignment. In these rounds, which we denote as compensation rounds, Alice prepares a state  $\rho_{\text{comp}}$  that is equivalent to the average state emitted in an untagged round, see Fig. S2. This ensures the overall equivalence between the Coin Protocol and the Virtual Protocol with tag assignment.

---

#### Coin Protocol

1. **State preparation:** (a) With probability  $p_C := p_{\text{TAR}} + p_{\text{REF}} = 2p_{\text{TAR}}$ , the round is a coin round. Alice prepares  $|\Psi_{\text{coin}}\rangle_{C D A B}$ , and sends system  $B$  through a quantum channel. (b) With probability  $1 - p_C$ , the round is a compensation round. Alice prepares  $\rho_{\text{comp}}$  and sends it through the quantum channel.
2. **Detection:** For each round, Bob performs the POVM  $\{\hat{m}_{0_X}, \hat{m}_{1_X}, \hat{m}_f\}$ . If he obtains a successful detection, which is associated to the outcome  $\hat{m}_{\text{det}} := \hat{\mathbb{I}} - \hat{m}_f$ , he announces this information.
3. **Coin measurement:** For each coin round, Alice chooses the basis  $Z_C$  ( $X_C$ ) with probability  $p_{Z_C}$  ( $p_{X_C}$ ), and measures system  $C$  in the chosen basis. Let  $N_{Z_C=0}^{\text{det}}$  ( $N_{Z_C=1}^{\text{det}}$ ) be the number of detected rounds in which Alice chose  $Z_C$  and obtained the outcome  $Z_C = 0$  ( $Z_C = 1$ ).
4. **Ancilla measurement:** For each detected coin round in which Alice chose  $Z_C$ , she measures system  $D$  in the basis  $\{|0\rangle_D, |1\rangle_D\}$ , whose measurement outcome we denote by  $D = d$  for  $d \in \{0, 1\}$ . Note that the outcome of this measurement, together with the outcome of Bob's measurement in Step 2, associates each of these rounds to one of  $\{\hat{m}_{\text{err}}, \hat{\mathbb{I}} - \hat{m}_{\text{err}}\}$ , where  $\hat{m}_{\text{err}} = |0\rangle\langle 0|_D \otimes \hat{m}_{1_X} + |1\rangle\langle 1|_D \otimes \hat{m}_{0_X}$ . Then, if she obtained  $D = 0$ , or if she obtained  $D = 1$  and  $Z_C = 1$ , she measures system  $A$  in the  $\{|0\rangle_A, |1\rangle_A\}$  basis; if she

obtained  $D = 1$  and  $Z_C = 0$ , she measures system  $A$  in the  $\{|0'\rangle_A, |1'\rangle_A\}$  basis. In either case, we denote the outcome of this measurement as  $A = a$ , with  $a \in \{0, 1\}$ . Also, let  $N_{Z_C=z, D=d, A=a}^{\beta_X}$  be the number of rounds in which Alice obtained  $Z_C = z, D = d, A = a$  and Bob obtained the outcome associated to  $\hat{m}_{\beta_X}$ , and let  $N_{Z_C=z, D=d, A=a}^{\det} = N_{Z_C=z, D=d, A=a}^{0_X} + N_{Z_C=z, D=d, A=a}^{1_X}$ .

Note that, in the coin rounds in which Alice chooses  $Z_C$ , Alice and Bob learn the same information as in the tagged rounds marked as  $Z_C$  in the Virtual Protocol with tag assignment. This allows us to draw an equivalence between the random variables associated to these rounds in the two scenarios. For example, in the Coin Protocol in Fig. S2, if Alice obtains  $Z_C = 0, d = 0$  and  $a = 0$ , she has learned that she emitted  $|\psi_{\text{vir}0}\rangle_B$ . The number of these events in which Bob obtains a measurement outcome of, say,  $1_X$ ,  $N_{Z_C=0, d=0, a=0}^{1_X}$ , is equivalent to the number of events in which, in the Virtual Protocol with tag assignment, Alice emits  $|\psi_{\text{vir}0}\rangle_B$ , assigns it a tag  $t = \text{TAR}$ , marks it as  $Z_C$ , and Bob obtains the outcome  $1_X$ ,  $N_{\text{vir}0, \text{TAR}, Z_C}^{1_X}$ . We represent this equivalence as  $N_{Z_C=0, d=0, a=0}^{1_X} \equiv N_{\text{vir}0, \text{TAR}, Z_C}^{1_X}$ . Moreover, in the Coin Protocol, due to the form of the operator  $\hat{m}_{\text{err}}$  and Eqs. (S21), (S22) and (S25), we have relationships of the form  $N_{Z_C=0}^{\text{err}} = N_{Z_C=0, d=0, a=0}^{1_X} + N_{Z_C=0, d=1, a=1}^{0_X} + N_{Z_C=0, d=1, a=0}^{0_X}$ , and so on. Putting it all together, we have that

$$\begin{aligned} N_{Z_C=0}^{\text{err}} &= N_{Z_C=0, d=0, a=0}^{1_X} + N_{Z_C=0, d=1, a=1}^{0_X} + N_{Z_C=0, d=1, a=0}^{0_X} \equiv N_{\text{vir}0, \text{TAR}, Z_C}^{1_X} + N_{\text{vir}1, \text{TAR}, Z_C}^{0_X} + N_{0_X, \text{TAR}, Z_C}^{0_X}, \\ N_{Z_C=1}^{\text{err}} &= N_{Z_C=1, d=0, a=0}^{1_X} + N_{Z_C=1, d=1, a=0}^{0_X} + N_{Z_C=1, d=1, a=1}^{0_X} \equiv N_{0_X, \text{REF}, Z_C}^{1_X} + N_{0_Z, \text{REF}, Z_C}^{0_X} + N_{1_Z, \text{REF}, Z_C}^{0_X}, \\ N_{Z_C=0}^{\det} &= N_{Z_C=0, d=0, a=0}^{\det} + N_{Z_C=0, d=1, a=1}^{\det} + N_{Z_C=0, d=1, a=0}^{\det} \equiv N_{\text{vir}0, \text{TAR}, Z_C}^{\det} + N_{\text{vir}1, \text{TAR}, Z_C}^{\det} + N_{0_X, \text{TAR}, Z_C}^{\det}, \\ N_{Z_C=1}^{\det} &= N_{Z_C=1, d=0, a=0}^{\det} + N_{Z_C=1, d=1, a=0}^{\det} + N_{Z_C=1, d=1, a=1}^{\det} \equiv N_{0_X, \text{REF}, Z_C}^{\det} + N_{0_Z, \text{REF}, Z_C}^{\det} + N_{1_Z, \text{REF}, Z_C}^{\det}. \end{aligned} \quad (\text{S36})$$

Substituting the random sampling relations in Eqs. (S34) and (S35) into Eq. (S36), we obtain

$$\begin{aligned} N_{Z_C=0}^{\text{err}} &\simeq p_{Z_C} (p_{\text{TAR}|\text{vir}0} N_{\text{vir}0}^{1_X} + p_{\text{TAR}|\text{vir}1} N_{\text{vir}1}^{0_X} + p_{\text{TAR}|0_X} N_{0_X}^{0_X}) \stackrel{(1)}{=} p_{Z_C} (p_{\text{TAR}|\text{vir}} N_{\text{ph}} + p_{\text{TAR}|0_X} N_{0_X}^{0_X}), \\ N_{Z_C=1}^{\text{err}} &\simeq p_{Z_C} (p_{\text{REF}|0_X} N_{0_X}^{1_X} + p_{\text{REF}|0_Z} N_{0_Z}^{0_X} + p_{\text{REF}|1_Z} N_{1_Z}^{0_X}), \\ N_{Z_C=0}^{\det} &\simeq p_{Z_C} (p_{\text{TAR}|\text{vir}0} N_{\text{vir}0}^{\det} + p_{\text{TAR}|\text{vir}1} N_{\text{vir}1}^{\det} + p_{\text{TAR}|0_X} N_{0_X}^{\det}) \stackrel{(2)}{=} p_{Z_C} (p_{\text{TAR}|\text{vir}} N_{\text{key}}^{\det} + p_{\text{TAR}|0_X} N_{0_X}^{\det}), \\ N_{Z_C=1}^{\det} &\simeq p_{Z_C} (p_{\text{REF}|0_X} N_{0_X}^{\det} + p_{\text{REF}|0_Z} N_{0_Z}^{\det} + p_{\text{REF}|1_Z} N_{1_Z}^{\det}). \end{aligned} \quad (\text{S37})$$

In the equalities marked by (1) and (2), we have used  $p_{\text{TAR}|\text{vir}} := p_{\text{TAR}|\text{vir}0} = p_{\text{TAR}|\text{vir}1}$ ; in the equality marked by (1), we have used  $N_{\text{ph}} := N_{\text{vir}0}^{1_X} + N_{\text{vir}1}^{0_X}$ ; and in the equality marked by (2), we have used the fact that  $N_{\text{vir}0}^{\det} + N_{\text{vir}1}^{\det}$  equals the length of the sifted key,  $N_{\text{key}}^{\det}$ .

As explained in Section SM1B2, using the quantum coin idea, we can find a statistical relationship — the quantum coin inequality — between the random variables  $\{N_{Z_C=0}^{\text{err}}, N_{Z_C=1}^{\text{err}}, N_{Z_C=0}^{\det}, N_{Z_C=1}^{\det}, N_{X_C=1}\}$ . Namely, in Section SE1, we show that,

$$N_{Z_C=0}^{\text{err}} \lesssim N_{Z_C=0}^{\det} G_+ \left( \frac{N_{Z_C=1}^{\text{err}}}{N_{Z_C=1}^{\det}}, 1 - \frac{2p_{Z_C} N_{X_C=1}}{p_{X_C} (N_{Z_C=0}^{\det} + N_{Z_C=1}^{\det})} \right), \quad (\text{S38})$$

where the symbol  $\lesssim$  means that, in the limit  $N \rightarrow \infty$ , the ratio between the left and right-hand sides is less or equal to one; and where

$$G_+(y, z) = \begin{cases} y + (1-z)(1-2y) + 2\sqrt{z(1-z)y(1-y)} & \text{if } 0 \leq y < z^2 \leq 1, \\ 1 & \text{otherwise.} \end{cases} \quad (\text{S39})$$

Moreover, note that the event “Alice generates the quantum coin, chooses the  $X_C$  basis and obtains the result  $X_C = 1$ ” is independently and identically distributed for the  $N$  rounds of the Coin Protocol, because Alice’s measurement on each coin system  $C$  commutes with any other measurement in any other system. Therefore, using the Chernoff bound, we have that

$$N_{X_C=1} \simeq N p_C p_{X_C} \frac{1 - \text{Re} \langle \Psi_{\text{Ref}} | \Psi_{\text{Tar}} \rangle_{DAB}}{2}. \quad (\text{S40})$$

In Section SE2, we show how to obtain a bound

$$1 - \text{Re} \langle \Psi_{\text{Ref}} | \Psi_{\text{Tar}} \rangle_{DAB} \leq \Delta, \quad (\text{S41})$$

numerically using SDP techniques, and analytically with an additional assumption on the form of the states  $\{|\psi_j\rangle_B\}_j$ . Combining Eqs. (S40) and (S41), we arrive at

$$N_{X_C=1} \lesssim \frac{N p_C p_{X_C} \Delta}{2} =: N_{X_C=1}^U. \quad (\text{S42})$$

Substituting Eq. (S42) into Eq. (S38), and using  $p_C := p_{\text{TAR}} + p_{\text{REF}} = 2p_{\text{TAR}}$ , we obtain

$$N_{Z_C=0}^{\text{err}} \lesssim N_{Z_C=0}^{\text{det}} G_+ \left( \frac{N_{Z_C=1}^{\text{err}}}{N_{Z_C=1}^{\text{det}}}, 1 - \frac{2p_{Z_C} p_{\text{TAR}} N \Delta}{N_{Z_C=0}^{\text{det}} + N_{Z_C=1}^{\text{det}}} \right). \quad (\text{S43})$$

Finally, substituting Eqs. (S33) and (S37) into Eq. (S43), and taking into account that  $N_l^{\text{det}} = N_l^{0x} + N_l^{1x}$  for  $l \in \{0_Z, 1_Z, 0_X\}$ , we obtain a bound of the form

$$N_{\text{ph}} \lesssim f(N_{0_Z}^{0x}, N_{0_Z}^{1x}, N_{1_Z}^{0x}, N_{1_Z}^{1x}, N_{0_X}^{0x}, N_{0_X}^{1x}, N_{\text{key}}^{\text{det}}) =: N_{\text{ph}}^U, \quad (\text{S44})$$

and, as desired, the bound on the phase-error rate is given by

$$e_{\text{ph}} \lesssim \frac{N_{\text{ph}}^U}{N_{\text{key}}^{\text{det}}} =: e_{\text{ph}}^U. \quad (\text{S45})$$

Note that, in the Coin Protocol defined in this Section, Alice and Bob do not make any basis and bit announcements. Therefore, strictly speaking, the Coin Protocol is only equivalent to the Virtual Protocol *before* the basis and bit announcement step of the latter. In other words, we have proven that Eq. (S45) holds *before* this basis and bit announcement step. However, note that  $e_{\text{ph}}^U$  is a function of the random variables  $\{N_{0_Z}^{0x}, N_{0_Z}^{1x}, N_{1_Z}^{0x}, N_{1_Z}^{1x}, N_{0_X}^{0x}, N_{0_X}^{1x}, N_{\text{key}}^{\text{det}}\}$ , whose distribution depends only on Eve's attack, which she can no longer modify after Bob has finished all his measurements in the quantum communication phase of the protocol. Thus, if Eq. (S45) holds *before* the basis and bit announcement step, it must also hold *after* this step, which concludes the proof.

Because of the above, a corollary of our result is that, in security proofs based on the quantum coin idea, including our proof, one can extract key from both the instances in which Alice selects  $Z_C$  and the instances in which she selects  $X_C$ . In fact, in the Actual Protocol, Alice does not even need to decide which instances belong to  $Z_C$  or  $X_C$ . This decision only needs to be made in the fictitious tag assignment step, allowing us to obtain a statistical statement for the rounds marked as  $Z_C$ , and then extending it to the rest of rounds via random sampling arguments. A key reason why this is allowed is that, in the Coin Protocol, Alice does not make any postselection or perform any operation that depends on the outcome of her  $X_C$  measurements. Moreover, our statistical bound on the number of phase errors does not depend on these outcomes, since the random variable  $N_{X_C=1}$  is replaced by its upper bound  $N_{X_C=1}^U$ , where both  $N_{X_C=1}^U$  and the failure probability of the bound  $\Pr[N_{X_C=1} > N_{X_C=1}^U]$  are constants that can be calculated and set before running the protocol. Therefore, the estimation remains valid even if, in the rounds marked as  $X_C$ , Alice does not actually perform the  $X_C$  measurement, or even if she performs the  $Z_C$  measurement instead. Moreover, since her measurement on the rounds marked as  $X_C$  does not change the reduced density operator on the rounds marked as  $Z_C$ , and the rounds marked as  $Z_C$  and  $X_C$  are identical, the statistical statement obtained for the rounds marked as  $Z_C$  can be extended to the rounds marked as  $X_C$  via the random sampling argument. This is another improvement over previous security proofs based on the quantum coin idea, in which, in the actual protocol, Alice actually needed to probabilistically mark each detected round as either  $Z_C$  or  $X_C$  and discard those marked as  $X_C$  [S17–S19].

Throughout this Section, for simplicity, we have assumed the asymptotic regime ( $N \rightarrow \infty$ ), in which the phase-error rate bound can be expressed as

$$e_{\text{ph}}^U \simeq \left( 1 + \frac{c_2 q_{\text{vir1}}^\phi Y_{0_X}}{Y_Z} \right) G_+ \left( \frac{q_{\text{vir0}}^\phi Y_{0_X}^{1x} + c_1 q_{\text{vir1}}^\phi (Y_{0_Z}^{0x} + Y_{1_Z}^{0x})}{q_{\text{vir0}}^\phi Y_{0_X} + c_1 q_{\text{vir1}}^\phi Y_Z}, 1 - \frac{2\Delta(1 + c_2 q_{\text{vir1}}^\phi)}{Y_Z + q_{\text{vir0}}^\phi Y_{0_X} + q_{\text{vir1}}^\phi (c_2 Y_{0_X} + c_1 Y_Z)} \right) - \frac{c_2 q_{\text{vir1}}^\phi Y_{0_X}^{0x}}{Y_Z}, \quad (\text{S46})$$

where we have used that  $N_j^{\beta x} \simeq N p_j Y_j^{\beta x}$  and  $N_{\text{key}}^{\text{det}} \simeq N p_{Z_A} p_{Z_B} Y_Z$ , with  $p_j$  for  $j \in \{0_Z, 1_Z, 0_X\}$  defined in Eq. (S26),  $Y_j^{\beta x}$  is the observed rate at which Bob obtains  $\beta x$  conditioned on Alice selecting the setting  $j$ , and  $Y_Z$  is the rate at which Bob obtains a detection event conditioned on Alice choosing the  $Z$  basis. Also, in Eq. (S46), we have used the fact that  $Y_Z = Y_Z^{0x} + Y_Z^{1x} = Y_Z^{0x} + Y_Z^{1x}$  (see Assumption A2). Using  $e_{\text{ph}}^U$ , we can finally obtain a lower bound on the asymptotic secret-key rate:

$$R \geq p_{Z_A} p_{Z_B} Y_Z [1 - h(e_{\text{ph}}^U) - fh(e_Z)], \quad (\text{S47})$$

where  $h(x) = -x \log_2 x - (1-x) \log_2 (1-x)$  is the binary entropy function,  $f$  is the error correction inefficiency and  $e_Z$  is the bit-error rate. We remark that it is straightforward to apply our analysis in the finite-key regime by taking into account the deviation terms and failure probabilities associated to the concentration inequalities employed in the analysis. In Section SM1 E, we explicitly show how to derive a bound on the phase-error rate that takes into account finite-key effects and how to calculate the secret-key length.

### C. Security proof for a particular BB84 scenario

#### 1. Security analysis

Here, we apply our security proof to the BB84 scenario considered in the Main Text. This scenario only differs from the one in the previous section in that Alice sends an additional state  $|\psi_{1x}\rangle_B$  whose qubit component  $|\phi_{1x}\rangle_B$  is given by Eq. (S12) with  $\theta_{1x} = 3\kappa\pi/4$ .

Similarly to Section SM1 B 1, we can use the LT analysis to obtain the following expressions

$$|\phi_{\text{vir}0}\rangle\langle\phi_{\text{vir}0}|_B = |\phi_{0x}\rangle\langle\phi_{0x}|_B, \quad (\text{S48})$$

$$c_1 |\phi_{0z}\rangle\langle\phi_{0z}|_B + |\phi_{\text{vir}1}\rangle\langle\phi_{\text{vir}1}|_B = c_2 |\phi_{1z}\rangle\langle\phi_{1z}|_B + c_3 |\phi_{1x}\rangle\langle\phi_{1x}|_B, \quad (\text{S49})$$

where

$$\begin{aligned} c_1 &:= \frac{\cos(\kappa\pi/2)}{\cos(\kappa\pi) - \cos(\kappa\pi/2)}, \\ c_2 &:= \frac{\cos(\kappa\pi/2)}{\cos(\kappa\pi/2) - 1}, \\ c_3 &:= \frac{1 + \cos(\kappa\pi/2)}{\cos(\kappa\pi/2) - \cos(\kappa\pi)}. \end{aligned} \quad (\text{S50})$$

We remark that, for this scenario, Eqs. (S48) and (S49) are just one of the possible ways to write the virtual states as a linear function of qubit states. Indeed, to find these expressions, we have to solve two systems of three linear equations with four unknowns, which have infinitely many solutions. This is in contrast with the three-state scenario considered in Section SM1 B, whose two systems of three linear equations have three unknowns and thus have a unique solution each. Here, we select the solution given by Eqs. (S48) and (S49) because it provides the tightest bound on the phase-error rate [S20]. When  $\epsilon \gtrsim 0$ , these equations do not hold exactly, but still hold approximately, i.e.,

$$|\psi_{\text{vir}0}\rangle\langle\psi_{\text{vir}0}|_B \approx |\psi_{0x}\rangle\langle\psi_{0x}|_B, \quad (\text{S51})$$

$$c_1 |\psi_{0z}\rangle\langle\psi_{0z}|_B + |\psi_{\text{vir}1}\rangle\langle\psi_{\text{vir}1}|_B \approx c_2 |\psi_{1z}\rangle\langle\psi_{1z}|_B + c_3 |\psi_{1x}\rangle\langle\psi_{1x}|_B. \quad (\text{S52})$$

Taking into account the relationships in Eqs. (S51) and (S52), we define the following target and reference states

$$|\Psi_{\text{Tar}}\rangle_{DAB} = \frac{1}{\sqrt{1 + c_1 q_{\text{vir}1}^\phi}} \left[ \sqrt{q_{\text{vir}0}^\psi} |0\rangle_D |0\rangle_A |\psi_{\text{vir}0}\rangle_B + |1\rangle_D \left( \sqrt{c_1 q_{\text{vir}1}^\phi} |0'\rangle_A |\psi_{0z}\rangle_B + \sqrt{q_{\text{vir}1}^\psi} |1'\rangle_A |\psi_{\text{vir}1}\rangle_B \right) \right], \quad (\text{S53})$$

$$|\Psi_{\text{Ref}}\rangle_{DAB} = \frac{1}{\sqrt{1 + c_1 q_{\text{vir}1}^\phi}} \left[ \sqrt{q_{\text{vir}0}^\phi} |0\rangle_D |0\rangle_A |\psi_{0x}\rangle_B + \sqrt{q_{\text{vir}1}^\phi} |1\rangle_D (\sqrt{c_2} |0\rangle_A |\psi_{1z}\rangle_B + \sqrt{c_3} |1\rangle_A |\psi_{1x}\rangle_B) \right], \quad (\text{S54})$$

where  $q_{\text{vir}\alpha}^\phi$  and  $q_{\text{vir}\alpha}^\psi$  are defined in Eq. (S18) and Eq. (S10), respectively. In Eq. (S54), the orthonormal basis  $\{|0'\rangle_A, |1'\rangle_A\}$  has been chosen such that

$$\sqrt{c_1} |0'\rangle_A |\phi_{0z}\rangle_B + |1'\rangle_A |\phi_{\text{vir}1}\rangle_B = \sqrt{c_2} |0\rangle_A |\phi_{1z}\rangle_B + \sqrt{c_3} |1\rangle_A |\phi_{1x}\rangle_B, \quad (\text{S55})$$

which must exist due to Eq. (S49), and can be calculated to be

$$\begin{aligned} |0'\rangle_A &= \sqrt{\frac{\cos(\kappa\pi) - \cos(\kappa\pi/2)}{\cos(\kappa\pi/2) - 1}} |0\rangle_A - \sqrt{-2 \cos(\kappa\pi/2)} |1\rangle_A, \\ |1'\rangle_A &= -\sqrt{-2 \cos(\kappa\pi/2)} |0\rangle_A - \sqrt{\frac{\cos(\kappa\pi) - \cos(\kappa\pi/2)}{\cos(\kappa\pi/2) - 1}} |1\rangle_A. \end{aligned} \quad (\text{S56})$$

Note that the definitions in Eqs. (S53) and (S54) are slightly different from those in Eqs. (9) and (10) of the Main Text, i.e., the coefficients associated with the actual states depend on  $q_{\text{vir}\alpha}^\phi$  rather than on  $q_{\text{vir}\alpha}^\psi$ . As explained in Methods, one can make different choices of target and reference states given that they satisfy the required conditions. The states in Eqs. (S53) and (S54) do so because: (1)  $|\Psi_{\text{Tar}}\rangle_{DAB} = |\Psi_{\text{Ref}}\rangle_{DAB}$  when  $\epsilon = 0$  due to our choice in Eq. (S56), and (2) the coefficient of the state  $|\psi_{\text{vir}0}\rangle_B$  ( $|\psi_{\text{vir}1}\rangle_B$ ) is proportional to  $\sqrt{q_{\text{vir}0}^\psi}$  ( $\sqrt{q_{\text{vir}1}^\psi}$ ). The advantage of Eqs. (S53) and (S54) over Eqs. (9) and (10) is that our final bound on  $e_{\text{ph}}$  is independent of  $q_{\text{vir}\alpha}^\psi$  (see Eq. (S63) below), and therefore no numerical optimization is needed. Using Eqs. (S53) and (S54), we can then define the loss-tolerant quantum coin state as

$$|\Psi_{\text{coin}}\rangle_{CDAB} = \frac{1}{\sqrt{2}}(|0_Z\rangle_C |\Psi_{\text{Tar}}\rangle_{DAB} + |1_Z\rangle_C |\Psi_{\text{Ref}}\rangle_{DAB}). \quad (\text{S57})$$

The rest of the analysis is essentially the same as for the three-state protocol. First, as in Section SM1 B 3, we add a fictitious tag assignment to the Virtual Protocol, such that the tagged rounds can be regarded as equivalent to generating the quantum coin state in Eq. (S57). The only difference is the definition of  $l$ , which for the BB84 protocol is  $l \in \{\text{vir}0, \text{vir}1, 0_Z, 1_Z, 0_X, 1_X\}$ . Then, as in Section SM1 B 4, we consider a Coin Protocol and obtain that, in the limit  $N \rightarrow \infty$ ,

$$\begin{aligned} N_{ZC=0}^{\text{err}} &\simeq p_{ZC}(p_{\text{Tar}|\text{vir}}N_{\text{ph}} + p_{\text{Tar}|0_Z}N_{0_Z}^{0_X}), \\ N_{ZC=1}^{\text{err}} &\simeq p_{ZC}(p_{\text{Ref}|0_X}N_{0_X}^{1_X} + p_{\text{Ref}|1_Z}N_{1_Z}^{0_X} + p_{\text{Ref}|1_X}N_{1_X}^{0_X}), \\ N_{ZC=0}^{\text{det}} &\simeq p_{ZC}(p_{\text{Tar}|\text{vir}}N_{\text{key}}^{\text{det}} + p_{\text{Tar}|0_Z}N_{0_Z}^{\text{det}}), \\ N_{ZC=1}^{\text{det}} &\simeq p_{ZC}(p_{\text{Ref}|0_X}N_{0_X}^{\text{det}} + p_{\text{Ref}|1_Z}N_{1_Z}^{\text{det}} + p_{\text{Ref}|1_X}N_{1_X}^{\text{det}}), \end{aligned} \quad (\text{S58})$$

where

$$\begin{aligned} p_{\text{Tar}|\text{vir}} &:= p_{\text{Tar}|\text{vir}0} = p_{\text{Tar}|\text{vir}1} = \frac{p_{\text{Tar}}}{p_{Z_A}p_{Z_B}(1 + c_1q_{\text{vir}1}^\phi)}, \\ p_{\text{Tar}|0_Z} &= \frac{2p_{\text{Tar}}c_1q_{\text{vir}1}^\phi}{p_{Z_A}p_{X_B}(1 + c_1q_{\text{vir}1}^\phi)}, \\ p_{\text{Ref}|0_X} &= \frac{2p_{\text{Tar}}q_{\text{vir}0}^\phi}{p_{X_A}p_{X_B}(1 + c_1q_{\text{vir}1}^\phi)}, \\ p_{\text{Ref}|1_Z} &= \frac{2p_{\text{Tar}}c_2q_{\text{vir}1}^\phi}{p_{Z_A}p_{X_B}(1 + c_1q_{\text{vir}1}^\phi)}, \\ p_{\text{Ref}|1_X} &= \frac{2p_{\text{Tar}}c_3q_{\text{vir}1}^\phi}{p_{X_A}p_{X_B}(1 + c_1q_{\text{vir}1}^\phi)}, \end{aligned} \quad (\text{S59})$$

and

$$p_{\text{Tar}} \leq (1 + c_1q_{\text{vir}1}^\phi) \min \left\{ p_{Z_A}p_{Z_B}, \frac{p_{Z_A}p_{X_B}}{2c_1q_{\text{vir}1}^\phi}, \frac{p_{Z_A}p_{X_B}}{2c_2q_{\text{vir}1}^\phi}, \frac{p_{X_A}p_{X_B}}{2q_{\text{vir}0}^\phi}, \frac{p_{X_A}p_{X_B}}{2c_3q_{\text{vir}1}^\phi} \right\}. \quad (\text{S60})$$

Finally, using the quantum coin inequality (see Section SE1 for more details), we have that

$$N_{ZC=0}^{\text{err}} \lesssim N_{ZC=0}^{\text{det}} G_+ \left( \frac{N_{ZC=1}^{\text{err}}}{N_{ZC=1}^{\text{det}}}, 1 - \frac{2p_{ZC}p_{\text{Tar}}N\Delta}{N_{ZC=0}^{\text{det}} + N_{ZC=1}^{\text{det}}} \right), \quad (\text{S61})$$

where  $\Delta \geq 1 - \text{Re} \langle \Psi_{\text{Ref}} | \Psi_{\text{Tar}} \rangle_{DAB}$ . As before, we can obtain  $\Delta$  by using SDP techniques, as described in Section SE2. Then, by substituting Eqs. (S58) and (S59) into Eq. (S61), and by taking into account that  $N_l^{\text{det}} = N_l^{0_X} + N_l^{1_X}$  for  $l \in \{0_Z, 1_Z, 0_X, 1_X\}$ , we obtain a bound of the form

$$N_{\text{ph}} \lesssim f(N_{0_Z}^{0_X}, N_{0_Z}^{1_X}, N_{1_Z}^{0_X}, N_{1_Z}^{1_X}, N_{0_X}^{0_X}, N_{0_X}^{1_X}, N_{1_X}^{0_X}, N_{1_X}^{1_X}, N_{\text{key}}^{\text{det}}) =: N_{\text{ph}}^{\text{U}}, \quad (\text{S62})$$

as desired. Our bound on the phase-error rate is then  $e_{\text{ph}}^{\text{U}} \simeq N_{\text{ph}}^{\text{U}}/N_{\text{key}}^{\text{det}}$ , and in the asymptotic regime, it can be expressed as

$$e_{\text{ph}}^{\text{U}} \simeq \left(1 + \frac{c_1 q_{\text{vir1}}^{\phi} Y_{0z}}{Y_Z}\right) G_+ \left( \frac{q_{\text{vir0}}^{\phi} Y_{0x}^{1x} + q_{\text{vir1}}^{\phi} (c_2 Y_{1z}^{0x} + c_3 Y_{1x}^{0x})}{q_{\text{vir0}}^{\phi} Y_{0x} + q_{\text{vir1}}^{\phi} (c_2 Y_{1z} + c_3 Y_{1x})}, 1 - \frac{2\Delta(1 + c_1 q_{\text{vir1}}^{\phi})}{Y_Z + q_{\text{vir0}}^{\phi} Y_{0x} + q_{\text{vir1}}^{\phi} (c_1 Y_{0z} + c_2 Y_{1z} + c_3 Y_{1x})} \right) - \frac{c_1 q_{\text{vir1}}^{\phi} Y_{0z}^{0x}}{Y_Z}. \quad (\text{S63})$$

Finally, by substituting Eq. (S63) into Eq. (S47) we obtain the secret-key rate of the protocol. We remark that this analysis can be extended to the finite-key regime using the procedure in Section SM1 E below.

## 2. Investigating how tight is our security proof

The analysis for the BB84 protocol presented in the previous section was used to plot Fig. 1 in the Main Text. As one can see in that figure, to achieve non-zero key rates at reasonable distances, one needs to guarantee that  $\epsilon$  is fairly small. However, here, we highlight that this is, for the most part, a fundamental limitation of QKD protocols, rather than a specific drawback of our analysis. More specifically, here we show that, if the only information available about the emitted states  $\{|\psi_j\rangle_B\}_j$  is that their overlap with some other states  $\{|\phi_j\rangle_B\}_j$  is bounded by a certain threshold, i.e.,  $|\langle\phi_j|\psi_j\rangle_B|^2 \geq 1 - \epsilon$ , no security proof can achieve any key rate when the detection rate  $\eta$  is such that  $\eta \leq \epsilon$ , which is not so far off from what our security proof achieves.

Remember that the emitted states can be expressed as in Eq. (S2), where the only information known about the side-channel states  $\{|\phi_j^\perp\rangle_B\}_j$  is that  $\langle\phi_j^\perp|\phi_j\rangle_B = 0$  for all  $j$ . This implies that the side-channel states might be in a high-dimensional space and completely distinguishable for different  $j$ , enabling very powerful attacks by Eve based on unambiguous state discrimination [S21]. To define a simple attack of this type, let us assume for simplicity that  $\langle\phi_k^\perp|\phi_j\rangle_B = 0$  and  $\langle\phi_k^\perp|\phi_j^\perp\rangle_B = 0$  for all  $j \neq k$ , and consider that, in each protocol round, Eve applies the POVM  $\{\hat{E}_{0z}, \hat{E}_{1z}, \hat{E}_{0x}, \hat{E}_{1x}, \hat{E}_{\text{inc}}\}$ , where  $\hat{E}_j = |\phi_j^\perp\rangle\langle\phi_j^\perp|_B$  and  $\hat{E}_{\text{inc}} = \mathbb{I} - \sum_j \hat{E}_j$ . By doing so, Eve will either unambiguously discriminate Alice's setting choice  $j$  with probability  $\epsilon$  or obtain an inconclusive result with probability  $1 - \epsilon$ . Then, if she gets a conclusive result, she resends the identified state to Bob; otherwise, she sends a vacuum state. This attack allows Eve to learn Alice's setting choices for all detected rounds without introducing any errors, and results in an observed detection rate  $\eta = \epsilon$ . This implies that, if the observed  $\eta$  is such that  $\eta \leq \epsilon$ , distilling a secret key is impossible, which can be used as a crude upper bound on the maximum distance at which any security proof could achieve a non-zero key rate, as illustrated by the dashed lines in Fig. S3. When  $\epsilon = 10^{-3}$ , it is impossible to obtain any key after 143 km, less than half the maximum distance that the standard BB84 protocol can achieve for  $\epsilon = 0$ , which is not so far off from the 100 km achievable using our security proof. We remark that this crude upper bound does not use any information about Bob's measurement results other than his overall detection rate, and a tighter bound may be obtained by taking into account his detailed observed statistics, including the observed bit-error rate.

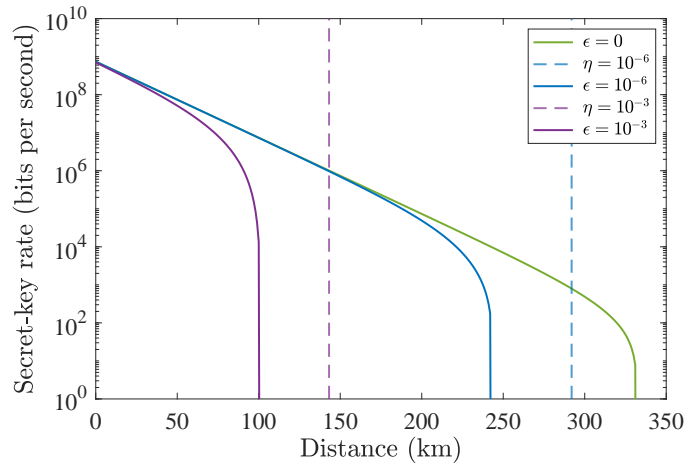

Figure S3. Asymptotic secret-key rate achievable when using our analysis for different values of  $\epsilon$ , under the assumption that  $\langle\phi_k^\perp|\phi_j\rangle_B = 0$  and  $\langle\phi_k^\perp|\phi_j^\perp\rangle_B = 0$  for  $j \neq k$  (solid lines), compared with a crude upper bound on the maximum distance at which a non-zero secret-key rate could be generated (dashed lines).

Hence, to achieve non-zero key rates at reasonable distances, there are only two possible experimental avenues: (1) ensuring that the overall magnitude of the side channels  $\epsilon$  is low enough, or (2) obtaining a (full or partial) characterization of the side-channel states  $\{|\phi_j^\perp\rangle\}_j$  (this could guarantee, for example, that  $\langle\phi_k^\perp|\phi_j^\perp\rangle_B \neq 0$ , thus ruling out the specific attack we have considered above). As we have argued in Methods, obtaining a characterization of the side-channel states appears to be significantly harder than simply obtaining a bound on  $\epsilon$ , and for this reason, when evaluating the performance of our security proof, we have assumed that no information is known about them. If some information is known, however, one could incorporate it into the SDP used to bound the inner product between the states  $|\Psi_{\text{Tar}}\rangle_{DAB}$  and  $|\Psi_{\text{Ref}}\rangle_{DAB}$  (see Section SE2), potentially resulting in a significant secret-key rate increase<sup>3</sup>. This highlights the flexibility and potential of our security proof to achieve good performances regardless of the information that is experimentally available.

### 3. Reduction to the original quantum coin analysis when there are no qubit flaws

Here, we show that our security proof reduces to the original quantum coin analysis when there are no qubit flaws (i.e., when  $\delta = 0$ ). In this case, we have that  $q_{\text{vir}0}^\phi = q_{\text{vir}1}^\phi = 1/2$  (see Eq. (S18)) and the coefficients in Eq. (S50) satisfy  $c_1 = c_2 = 0$  and  $c_3 = 1$ . Substituting these in Eq. (S63), we obtain

$$e_{\text{ph}}^U \simeq G_+ \left( \frac{Y_{0x}^{1x} + Y_{1x}^{0x}}{Y_{0x} + Y_{1x}}, 1 - \frac{2\Delta}{Y_Z + \frac{1}{2}(Y_{0x} + Y_{1x})} \right) = G_+ \left( e_X, 1 - \frac{2\Delta}{Y_Z + Y_X} \right) = G_+(e_X, 1 - 2\Delta'), \quad (\text{S64})$$

where in the second equality we have defined  $Y_X := (Y_{0x} + Y_{1x})/2$  and  $e_X := (Y_{0x}^{1x} + Y_{1x}^{0x})/(Y_{0x} + Y_{1x})$ ; and in the third equality we have defined  $\Delta' := \Delta/(Y_Z + Y_X)$ , with  $\Delta \geq 1 - \text{Re}\langle\Psi_X|\Psi_Z\rangle_{AB}$ . Equation (S64) is exactly the same phase-error rate bound as that of the original quantum coin analysis, see [S22]. Therefore, in Fig. 2 of the Main Text, the secret-key rate offered by the two analyses overlaps when  $\delta = 0$ .

To see why this is the case, let us substitute  $c_1 = c_2 = 0$ ,  $c_3 = 1$  and  $q_{\text{vir}0}^\phi = q_{\text{vir}1}^\phi = 1/2$  in Eqs. (S53) and (S54). Then, the target and reference states become

$$|\Psi_{\text{Tar}}\rangle_{DAB} = \sqrt{q_{\text{vir}0}^\psi} |0\rangle_D |0\rangle_A |\psi_{\text{vir}0}\rangle_B - \sqrt{q_{\text{vir}1}^\psi} |1\rangle_D |1\rangle_A |\psi_{\text{vir}1}\rangle_B, \quad (\text{S65})$$

$$|\Psi_{\text{Ref}}\rangle_{DAB} = \frac{1}{\sqrt{2}} [ |0\rangle_D |0\rangle_A |\psi_{0x}\rangle_B + |1\rangle_D |1\rangle_A |\psi_{1x}\rangle_B ], \quad (\text{S66})$$

where we have used the fact that  $|1'\rangle_A = -|1\rangle_A$  when  $\delta = 0$ . Then, by redefining  $|i\rangle_D |i\rangle_A$  as  $|i_X\rangle_A$  for  $i \in \{0, 1\}$  in Eqs. (S65) and (S66), where  $|i_X\rangle_A := (|0_Z\rangle + (-1)^i |1_Z\rangle)/\sqrt{2}$ , we obtain

$$|\Psi_{\text{Tar}}\rangle_{DAB} = \frac{1}{\sqrt{2}} (|0_Z\rangle_A |\psi_{0z}\rangle_B + |1_Z\rangle_A |\psi_{1z}\rangle_B) = |\Psi_Z\rangle_{AB}, \quad (\text{S67})$$

$$|\Psi_{\text{Ref}}\rangle_{DAB} = \frac{1}{\sqrt{2}} (|0_X\rangle_A |\psi_{0x}\rangle_B - |1_X\rangle_A |\psi_{1x}\rangle_B) = |\Psi_X\rangle_{AB}. \quad (\text{S68})$$

Note that Eqs. (S67) and (S68) are equivalent to the states  $|\Psi_Z(\epsilon)\rangle_{AB}$  and  $|\Psi_X(\epsilon)\rangle_{AB}$  in Eqs. (4) and (5) of the Main Text. Therefore, our quantum coin state is

$$|\Psi_{\text{coin}}\rangle_{CAB} = \frac{1}{\sqrt{2}} (|0_Z\rangle_C |\Psi_Z\rangle_{AB} + |1_Z\rangle_C |\Psi_X\rangle_{AB}), \quad (\text{S69})$$

which is identical to that in Eq. (6). Therefore, our security proof reduces to the original quantum coin analysis in the absence of qubit flaws.

<sup>3</sup> In fact, we remark that, in Fig. S3, we have computed the performance of our security analysis under the assumption that  $\langle\phi_k^\perp|\phi_j\rangle_B = 0$  and  $\langle\phi_k^\perp|\phi_j^\perp\rangle_B = 0$  for  $j \neq k$ , as this assumption is also made in the calculation of the upper bound; intuitively, this should not be very far off from the worst-case scenario, since it assumes that the side-channel states are orthogonal and thus completely distinguishable. Nevertheless, Fig. S3 already shows a slight but appreciable key-rate improvement with respect to the scenario considered in the Main Text, in which no such assumption is made.

### D. General analysis for prepare-and-measure protocols

Here, we present the general version of our analysis for P&M protocols, which can be applied irrespectively of whether Alice sends three or four states, and irrespectively of the form of the qubit components  $\{|\phi_j\rangle_B\}_j$ . The analyses presented in Sections SM1 B and SM1 C are special cases of this general approach. However, to understand the main ideas of the security proof, we recommend reading Sections SM1 B and SM1 C first. The starting point of our general analysis is the LT expressions

$$|\phi_{\text{vir}\alpha}\rangle\langle\phi_{\text{vir}\alpha}|_B + \sum_{j \in C_{\text{Tar}}^{(\alpha)}} c_j^{(\alpha)} |\phi_j\rangle\langle\phi_j|_B = \sum_{j \in C_{\text{Ref}}^{(\alpha)}} c_j^{(\alpha)} |\phi_j\rangle\langle\phi_j|_B, \quad (\text{S70})$$

where  $\alpha \in \{0, 1\}$ ,  $c_j^{(\alpha)} \geq 0$  for all  $j, \alpha$ , and  $|\phi_{\text{vir}\alpha}\rangle_B$  are the qubit analogues of Eq. (S9), defined as

$$\begin{aligned} |\phi_{\text{vir}0}\rangle_B &= \frac{1}{2\sqrt{q_{\text{vir}0}^\phi}} (|\phi_{0z}\rangle_B + e^{i\omega} |\phi_{1z}\rangle_B), \\ |\phi_{\text{vir}1}\rangle_B &= \frac{1}{2\sqrt{q_{\text{vir}1}^\phi}} (|\phi_{0z}\rangle_B - e^{i\omega} |\phi_{1z}\rangle_B), \end{aligned} \quad (\text{S71})$$

with

$$\begin{aligned} q_{\text{vir}0}^\phi &= \frac{1}{2} (1 + \text{Re } e^{i\omega} \langle\phi_{0z}|\phi_{1z}\rangle_B), \\ q_{\text{vir}1}^\phi &= \frac{1}{2} (1 - \text{Re } e^{i\omega} \langle\phi_{0z}|\phi_{1z}\rangle_B). \end{aligned} \quad (\text{S72})$$

These expressions can always be obtained, although the procedure varies slightly depending on the Bloch vectors of the states  $\{|\phi_j\rangle_B\}_j$ , and requires setting the parameter  $\omega$  appropriately:

*Case 1: The end points of the Bloch vectors of the states  $\{|\phi_j\rangle_B\}_j$  lie in the same plane, and this plane passes through the origin—.* Without loss of generality, we can assume that this plane is the XZ plane; if it is not, one should simply redefine the Bloch sphere such that it is. For this case, one should take  $\omega = 0$ , and follow the procedure detailed in Appendix B.1 of [S15] to obtain the LT formulas in Eq. (S70). Note that the specific scenarios considered in Section SM1 B and Section SM1 C fall under this Case. If the set  $\{|\phi_j\rangle_B\}_j$  contains three states (as in Section SM1 B), the LT formulas are unique, whereas if it contains four states (as in Section SM1 C), there are infinitely many expressions of the form in Eq. (S70). In general, choosing expressions with lower coefficients should result in a tighter analysis [S20].

*Case 2: The end points of the Bloch vectors of the states  $\{|\phi_j\rangle_B\}_j$  lie in the same plane, but this plane does not pass through the origin—.* In this case, one should choose the parameter  $\omega$  appropriately such that the end points of the Bloch vectors of the states  $|\phi_{\text{vir}0}\rangle_B$  and  $|\phi_{\text{vir}1}\rangle_B$  lie in the same plane as those of the states  $\{|\phi_j\rangle_B\}_j$ , as explained in Appendix B.2 of [S15]. By following the procedure detailed there, one can obtain the LT formulas in Eq. (S70). As in *Case 1*, when the set  $\{|\phi_j\rangle_B\}_j$  contains three states, these expressions are unique, and when it contains four states, there are infinitely many expressions to choose from.

*Case 3: The end points of the Bloch vectors of the states  $\{|\phi_j\rangle_B\}_j$  are not in the same plane (i.e., they form a pyramid)—.* This can only occur when the set  $\{|\phi_j\rangle_B\}_j$  contains four states. In this case, one can find unique expressions of the form in Eq. (S70) regardless of the value of  $\omega$ ; in general, one can simply choose  $\omega = 0$ . This is because, in this case, the Pauli operators  $\{\sigma_I, \sigma_Z, \sigma_X, \sigma_Y\}$  can be uniquely expressed as a linear combination of  $\{|\phi_j\rangle\langle\phi_j|_B\}_j$ , and any density operator in this qubit space, including the virtual states  $|\phi_{\text{vir}\alpha}\rangle\langle\phi_{\text{vir}\alpha}|_B$ , can be expressed uniquely as a linear combination of the Pauli operators. For more information, see [S14].

Once we have the expressions in Eq. (S70), we use them as a blueprint to construct the target and reference states

$|\Psi_{\text{Tar}}\rangle_{DAB}$  and  $|\Psi_{\text{Ref}}\rangle_{DAB}$ . First, we take purifications of the left- and right-hand sides of Eq. (S70),

$$|0\rangle_A |\phi_{\text{vir}\alpha}\rangle_B + \sum_{j \in \mathcal{C}_{\text{Tar}}^{(\alpha)}} \sqrt{c_j^{(\alpha)}} |k_j^{(\alpha)}\rangle_A |\phi_j\rangle_B, \quad (\text{S73})$$

$$\sum_{j \in \mathcal{C}_{\text{Ref}}^{(\alpha)}} \sqrt{c_j^{(\alpha)}} |k_j'^{(\alpha)}\rangle_A |\phi_j\rangle_B, \quad (\text{S74})$$

where  $\{|0\rangle_A\} \cup \{|k_j^{(\alpha)}\rangle_A\}_{j \in \mathcal{C}_{\text{Tar}}^{(\alpha)}}$  and  $\{|k_j'^{(\alpha)}\rangle_A\}_{j \in \mathcal{C}_{\text{Ref}}^{(\alpha)}}$  are orthonormal bases chosen appropriately such that Eqs. (S73) and (S74) are identical; these bases always exist due to the equality in Eq. (S70). Then, making use of Eqs. (S73) and (S74), we define the normalized states

$$|\Phi_{\text{Tar}}\rangle_{DAB} = 1/\sqrt{C} \left[ \sum_{\alpha \in \{0,1\}} \sqrt{q_{\text{vir}\alpha}^\phi} |\alpha\rangle_D \left( |0\rangle_A |\phi_{\text{vir}\alpha}\rangle_B + \sum_{j \in \mathcal{C}_{\text{Tar}}^{(\alpha)}} \sqrt{c_j^{(\alpha)}} |k_j^{(\alpha)}\rangle_A |\phi_j\rangle_B \right) \right], \quad (\text{S75})$$

$$|\Phi_{\text{Ref}}\rangle_{DAB} = 1/\sqrt{C} \left[ \sum_{\alpha \in \{0,1\}} \sqrt{q_{\text{vir}\alpha}^\phi} |\alpha\rangle_D \left( \sum_{j \in \mathcal{C}_{\text{Ref}}^{(\alpha)}} \sqrt{c_j^{(\alpha)}} |k_j'^{(\alpha)}\rangle_A |\phi_j\rangle_B \right) \right], \quad (\text{S76})$$

where

$$C = 1 + \sum_{\alpha \in \{0,1\}} \sum_{j \in \mathcal{C}_{\text{Tar}}^{(\alpha)}} q_{\text{vir}\alpha}^\phi c_j^{(\alpha)} = \sum_{\alpha \in \{0,1\}} \sum_{j \in \mathcal{C}_{\text{Ref}}^{(\alpha)}} q_{\text{vir}\alpha}^\phi c_j^{(\alpha)}, \quad (\text{S77})$$

is a normalization factor. Note that  $|\Phi_{\text{Tar}}\rangle_{DAB} = |\Phi_{\text{Ref}}\rangle_{DAB}$ . Finally, we substitute  $|\phi_j\rangle_B \rightarrow |\psi_j\rangle_B$  and  $|\phi_{\text{vir}\alpha}\rangle_B \rightarrow |\psi_{\text{vir}\alpha}\rangle_B$  in Eqs. (S75) and (S76), and then substitute  $q_{\text{vir}\alpha}^\phi \rightarrow q_{\text{vir}\alpha}^\psi$  only in the terms multiplying the state  $|\psi_{\text{vir}\alpha}\rangle_B$ , obtaining

$$|\Psi_{\text{Tar}}\rangle_{DAB} = 1/\sqrt{C} \left[ \sum_{\alpha \in \{0,1\}} |\alpha\rangle_D \left( \sqrt{q_{\text{vir}\alpha}^\psi} |0\rangle_A |\psi_{\text{vir}\alpha}\rangle_B + \sqrt{q_{\text{vir}\alpha}^\phi} \sum_{j \in \mathcal{C}_{\text{Tar}}^{(\alpha)}} \sqrt{c_j^{(\alpha)}} |k_j^{(\alpha)}\rangle_A |\psi_j\rangle_B \right) \right], \quad (\text{S78})$$

$$|\Psi_{\text{Ref}}\rangle_{DAB} = 1/\sqrt{C} \left[ \sum_{\alpha \in \{0,1\}} \sqrt{q_{\text{vir}\alpha}^\phi} |\alpha\rangle_D \left( \sum_{j \in \mathcal{C}_{\text{Ref}}^{(\alpha)}} \sqrt{c_j^{(\alpha)}} |k_j'^{(\alpha)}\rangle_A |\psi_j\rangle_B \right) \right]. \quad (\text{S79})$$

We can then define the quantum coin state as

$$|\Psi_{\text{coin}}\rangle_{CDAB} = \frac{1}{\sqrt{2}} (|0_Z\rangle_C |\Psi_{\text{Tar}}\rangle_{DAB} + |1_Z\rangle_C |\Psi_{\text{Ref}}\rangle_{DAB}). \quad (\text{S80})$$

Let us rewrite Eqs. (S78) and (S79) as

$$|\Psi_{\text{Tar}}\rangle_{DAB} = \sum_{\alpha \in \{0,1\}} \sqrt{p_{\text{Tar}\alpha}|\text{Tar}} |\alpha\rangle_D |\Psi_{\text{Tar}\alpha}\rangle_{AB}, \quad (\text{S81})$$

$$|\Psi_{\text{Ref}}\rangle_{DAB} = \sum_{\alpha \in \{0,1\}} \sqrt{p_{\text{Ref}\alpha}|\text{Ref}} |\alpha\rangle_D |\Psi_{\text{Ref}\alpha}\rangle_{AB}, \quad (\text{S82})$$

where

$$p_{\text{Tar}\alpha}|\text{Tar} = \frac{q_{\text{vir}\alpha}^\psi + q_{\text{vir}\alpha}^\phi \sum_{j \in \mathcal{C}_{\text{Tar}}^{(\alpha)}} c_j^{(\alpha)}}{C}, \quad (\text{S83})$$

$$p_{\text{Ref}\alpha}|\text{Ref} = \frac{q_{\text{vir}\alpha}^\phi \sum_{j \in \mathcal{C}_{\text{Ref}}^{(\alpha)}} c_j^{(\alpha)}}{C}, \quad (\text{S84})$$

and

$$|\Psi_{\text{Tar}\alpha}\rangle_{AB} = \sqrt{p_{\text{vir}\alpha}|\text{Tar}\alpha} |0\rangle_A |\psi_{\text{vir}\alpha}\rangle + \sum_{j \in \mathcal{C}_{\text{Tar}}^{(\alpha)}} \sqrt{p_{j|\text{Tar}\alpha}} |k_j^{(\alpha)}\rangle_A |\psi_j\rangle_B, \quad (\text{S85})$$

$$|\Psi_{\text{Ref}\alpha}\rangle_{AB} = \sum_{j \in \mathcal{C}_{\text{Ref}}^{(\alpha)}} \sqrt{p_{j|\text{Ref}\alpha}} |k_j'^{(\alpha)}\rangle_A |\psi_j\rangle_B, \quad (\text{S86})$$

with

$$p_{\text{vir}\alpha|\text{TAR}\alpha} = \frac{q_{\text{vir}\alpha}^{\psi}}{q_{\text{vir}\alpha}^{\psi} + q_{\text{vir}\alpha}^{\phi} \sum_{j \in \mathcal{C}_{\text{TAR}}^{(\alpha)}} c_j^{(\alpha)}}, \quad (\text{S87})$$

$$p_{j|\text{TAR}\alpha} = \frac{q_{\text{vir}\alpha}^{\phi} c_j^{(\alpha)}}{q_{\text{vir}\alpha}^{\psi} + q_{\text{vir}\alpha}^{\phi} \sum_{j' \in \mathcal{C}_{\text{TAR}}^{(\alpha)}} c_{j'}^{(\alpha)}} \quad \text{for } j \in \mathcal{C}_{\text{TAR}}^{(\alpha)}, \quad (\text{S88})$$

$$p_{j|\text{REF}\alpha} = \frac{c_j^{(\alpha)}}{\sum_{j' \in \mathcal{C}_{\text{REF}}^{(\alpha)}} c_{j'}^{(\alpha)}} \quad \text{for } j \in \mathcal{C}_{\text{REF}}^{(\alpha)}. \quad (\text{S89})$$

### Tagging

Similarly to Section SM1 B 3, we consider the addition of the following fictitious tag assignment step to the Virtual Protocol:

- 
- 1.5. **Tag assignment:** For each event  $l$ , Alice assigns it a single tag  $t \in \{\text{TARO}, \text{TAR1}, \text{REF0}, \text{REF1}\}$  with probability  $p_{t|l}$ , or no tag with probability  $1 - \sum_t p_{t|l}$ . Then, for the tagged events, Alice marks each emission as  $Z_C$  ( $X_C$ ) with probability  $p_{Z_C}$  ( $p_{X_C} = 1 - p_{Z_C}$ ).
- 

In this general case, we need to consider the tags  $\{\text{TARO}, \text{TAR1}, \text{REF0}, \text{REF1}\}$ , rather than just  $\{\text{TAR}, \text{REF}\}$ , because the same state could appear twice in each of Eqs. (S78) and (S79). For example, if  $0_Z \in \mathcal{C}_{\text{REF}}^{(0)}$  and  $0_Z \in \mathcal{C}_{\text{REF}}^{(1)}$ , the state  $|\psi_{0_Z}\rangle_B$  would appear twice in Eq. (S79), and one needs to distinguish whether an emission of  $|\psi_{0_Z}\rangle_B$  is assigned to the  $|0\rangle_D$  part (REF0) or the  $|1\rangle_D$  part (REF1) of the state.

The conditional tag assignment probabilities  $p_{t|l}$  should be chosen appropriately such that the probability that an emission with tag  $t$  originated from event  $l$ ,  $p_{l|t}$ , matches Eqs. (S87) to (S89). As before, we can use Bayes' Theorem to obtain an expression for  $p_{t|l}$  in terms of  $p_{l|t}$ ,  $p_t$  and  $p_l$ , i.e.,

$$p_{t|l} = \frac{p_t p_{l|t}}{p_l}, \quad (\text{S90})$$

where  $p_{l|t}$  is given by Eqs. (S87) to (S89),

$$\begin{aligned} p_l &= p_{Z_A} p_{Z_B} q_{\text{vir}\alpha}^{\psi} & \text{for } l \in \{\text{vir}\alpha\}_{\alpha \in \{0,1\}}, \\ p_l &= \frac{p_{Z_A}}{2} p_{X_B} & \text{for } l \in \{0_Z, 1_Z\}, \end{aligned} \quad (\text{S91})$$

and in the three-state scenario,

$$p_l = p_{X_A} p_{X_B} \quad \text{for } l = 0_X, \quad (\text{S92})$$

while, in the four-state scenario,

$$p_l = \frac{p_{X_A}}{2} p_{X_B} \quad \text{for } l \in \{0_X, 1_X\}. \quad (\text{S93})$$

Note that conditional tag assignment probabilities  $\{p_{t|l}\}$  become fixed once we fix  $\{p_t\}$ . Taking the sum over  $t \in \{\text{TARO}, \text{TAR1}, \text{REF0}, \text{REF1}\}$  on both sides of Eq. (S90) and using the fact that  $\sum_t p_{t|l} \leq 1$ , we derive the following constraints,

$$\sum_t p_t p_{l|t} \leq p_l, \quad \forall l. \quad (\text{S94})$$

Let  $p_{\text{TAR}} = p_{\text{TAR0}} + p_{\text{TAR1}}$  and  $p_{\text{REF}} = p_{\text{REF0}} + p_{\text{REF1}}$ . We want that

$$p_{\text{TAR}\alpha} = p_{\text{TAR}} p_{\text{TAR}\alpha|\text{TAR}}, \quad (\text{S95})$$

$$p_{\text{REF}\alpha} = p_{\text{REF}} p_{\text{REF}\alpha|\text{REF}}, \quad (\text{S96})$$

where  $p_{\text{TAR}\alpha|\text{TAR}}$  and  $p_{\text{REF}\alpha|\text{REF}}$  are given by Eqs. (S83) and (S84). We also want that  $p_{\text{TAR}} = p_{\text{REF}}$ , since the reference and target states have the same coefficient in Eq. (S80). Putting everything together, we obtain

$$\begin{aligned}
p_l &\geq \sum_t p_t p_{l|t} = \sum_{\alpha \in \{0,1\}} (p_{\text{TAR}\alpha} p_{l|\text{TAR}\alpha} + p_{\text{REF}\alpha} p_{l|\text{REF}\alpha}) \\
&= \sum_{\alpha \in \{0,1\}} (p_{\text{TAR}} p_{\text{TAR}\alpha|\text{TAR}} p_{l|\text{TAR}\alpha} + p_{\text{REF}} p_{\text{REF}\alpha|\text{REF}} p_{l|\text{REF}\alpha}) \\
&= \sum_{\alpha \in \{0,1\}} (p_{\text{TAR}} p_{\text{TAR}\alpha|\text{TAR}} p_{l|\text{TAR}\alpha} + p_{\text{TAR}} p_{\text{REF}\alpha|\text{REF}} p_{l|\text{REF}\alpha}) \\
&= p_{\text{TAR}} \sum_{\alpha \in \{0,1\}} (p_{\text{TAR}\alpha|\text{TAR}} p_{l|\text{TAR}\alpha} + p_{\text{REF}\alpha|\text{REF}} p_{l|\text{REF}\alpha}).
\end{aligned} \tag{S97}$$

The only constraint on the value of  $p_{\text{TAR}}$  is that Eq. (S97) holds for all  $l$ . Therefore, we can set its value as

$$p_{\text{TAR}} = \min_l \frac{p_l}{\sum_{\alpha \in \{0,1\}} (p_{\text{TAR}\alpha|\text{TAR}} p_{l|\text{TAR}\alpha} + p_{\text{REF}\alpha|\text{REF}} p_{l|\text{REF}\alpha})}. \tag{S98}$$

Once we set  $p_{\text{TAR}}$ , the tag selection probabilities  $p_{\text{TAR}\alpha}$  and  $p_{\text{REF}\alpha}$  become fixed, and so do the conditional tag assignment probabilities  $p_{t|l}$ . As in Section SM1 B 3, we have that, in the limit  $N \rightarrow \infty$ ,

$$\begin{aligned}
N_{l,t,Z_C}^{\beta x} &\simeq p_{Z_C} p_{t|l} N_l^{\beta x}, \\
N_{l,t,Z_C}^{\text{det}} &\simeq p_{Z_C} p_{t|l} N_l^{\text{det}}.
\end{aligned} \tag{S99}$$

### Coin Protocol

In the scenario described above, the tags  $\{\text{TAR0}, \text{TAR1}, \text{REF0}, \text{REF1}\}$  are assigned such that an emission with a tag **TAR0** is indistinguishable from the preparation of the state  $|\Psi_{\text{TAR0}}\rangle_{AB}$ , and similar for the others. Moreover, since the probabilities  $p_{\text{TAR0}}$  and  $p_{\text{TAR1}}$  ( $p_{\text{REF0}}$  and  $p_{\text{REF1}}$ ) satisfy Eq. (S95) (Eq. (S96)), an emission with a tag  $t \in \{\text{TAR0}, \text{TAR1}\}$  ( $t \in \{\text{REF0}, \text{REF1}\}$ ) is equivalent to the preparation of the state  $|\Psi_{\text{TAR}}\rangle_{DAB}$  ( $|\Psi_{\text{REF}}\rangle_{DAB}$ ). Finally, since  $p_{\text{TAR0}} + p_{\text{TAR1}} = p_{\text{REF0}} + p_{\text{REF1}}$ , an emission with a tag  $t \in \{\text{TAR0}, \text{TAR1}, \text{REF0}, \text{REF1}\}$  is equivalent to that originating from the quantum coin state  $|\Psi_{\text{coin}}\rangle_{CDAB}$ . This equivalence allows us to define a Coin Protocol as in Section SM1 B 4, in which Alice prepares the quantum coin state with probability  $p_C := p_{\text{TAR0}} + p_{\text{TAR1}} + p_{\text{REF0}} + p_{\text{REF1}} = 2p_{\text{TAR}}$ . Using similar arguments as in Section SM1 B 4, due to the equivalence between the Virtual Protocol after the tag assignment and the Coin Protocol, we have that

$$\begin{aligned}
N_{Z_C=0}^{\text{err}} &\equiv \sum_{\alpha \in \{0,1\}} \left[ N_{\text{vir}\alpha, \text{TAR}\alpha, Z_C}^{(\alpha \oplus 1)x} + \sum_{j \in C_{\text{TAR}}^{(\alpha)}} N_{j, \text{TAR}\alpha, Z_C}^{(\alpha \oplus 1)x} \right], \\
N_{Z_C=1}^{\text{err}} &\equiv \sum_{\alpha \in \{0,1\}} \sum_{j \in C_{\text{REF}}^{(\alpha)}} N_{j, \text{REF}\alpha, Z_C}^{(\alpha \oplus 1)x}, \\
N_{Z_C=0}^{\text{det}} &\equiv \sum_{\alpha \in \{0,1\}} \left[ N_{\text{vir}\alpha, \text{TAR}\alpha, Z_C}^{\text{det}} + \sum_{j \in C_{\text{TAR}}^{(\alpha)}} N_{j, \text{TAR}\alpha, Z_C}^{\text{det}} \right], \\
N_{Z_C=1}^{\text{det}} &\equiv \sum_{\alpha \in \{0,1\}} \sum_{j \in C_{\text{REF}}^{(\alpha)}} N_{j, \text{REF}\alpha, Z_C}^{\text{det}}.
\end{aligned} \tag{S100}$$

Substituting the random sampling relations in Eq. (S99) into Eq. (S100), we obtain that, in the limit  $N \rightarrow \infty$ ,

$$\begin{aligned}
N_{Z_C=0}^{\text{err}} &\simeq p_{Z_C} \left( p_{\text{TAR}|\text{vir}} N_{\text{ph}} + \sum_{\alpha \in \{0,1\}} \sum_{j \in \mathcal{C}_{\text{TAR}}^{(\alpha)}} p_{\text{TAR}\alpha|j} N_j^{(\alpha \oplus 1)x} \right), \\
N_{Z_C=1}^{\text{err}} &\simeq p_{Z_C} \left( \sum_{\alpha \in \{0,1\}} \sum_{j \in \mathcal{C}_{\text{Ref}}^{(\alpha)}} p_{\text{REF}\alpha|j} N_j^{(\alpha \oplus 1)x} \right), \\
N_{Z_C=0}^{\text{det}} &\simeq p_{Z_C} \left( p_{\text{TAR}|\text{vir}} N_{\text{key}}^{\text{det}} + \sum_{\alpha \in \{0,1\}} \sum_{j \in \mathcal{C}_{\text{TAR}}^{(\alpha)}} p_{\text{TAR}\alpha|j} N_j^{\text{det}} \right), \\
N_{Z_C=1}^{\text{det}} &\simeq p_{Z_C} \left( \sum_{\alpha \in \{0,1\}} \sum_{j \in \mathcal{C}_{\text{Ref}}^{(\alpha)}} p_{\text{REF}\alpha|j} N_j^{\text{det}} \right),
\end{aligned} \tag{S101}$$

where we have used that  $p_{\text{TAR}0|\text{vir}0} = p_{\text{TAR}1|\text{vir}1} =: p_{\text{TAR}|\text{vir}}$ . The latter relationship can be derived by substituting into Eq. (S90) the definition of  $p_{\text{vir}0|\text{TAR}0}$  and  $p_{\text{vir}1|\text{TAR}1}$  in Eq. (S87), the definition of  $p_{\text{vir}0}$  and  $p_{\text{vir}1}$  in Eq. (S91), and the definition of  $p_{\text{TAR}0}$  and  $p_{\text{TAR}1}$  in Eq. (S95). Also, in Eq. (S101), we have used  $N_{\text{key}}^{\text{det}} = N_{\text{vir}0}^{0x} + N_{\text{vir}0}^{1x} + N_{\text{vir}1}^{0x} + N_{\text{vir}1}^{1x}$ , where  $N_{\text{key}}^{\text{det}}$  is the total number of detected key rounds, i.e., the length of the sifted key.

As in Section SM1 B 4, we have that, in the Coin Protocol,

$$N_{Z_C=0}^{\text{err}} \lesssim N_{Z_C=0}^{\text{det}} G + \left( \frac{N_{Z_C=1}^{\text{err}}}{N_{Z_C=1}^{\text{det}}}, 1 - \frac{p_{Z_C} p_C N \Delta}{N_{Z_C=0}^{\text{det}} + N_{Z_C=1}^{\text{det}}} \right). \tag{S102}$$

Finally, substituting Eq. (S101),  $p_C = 2p_{\text{TAR}}$ ,  $N_l^{\text{det}} = N_l^{0x} + N_l^{1x}$  for  $l \in \{j\}_j$ , and the values of  $\{p_{t|l}\}$  into Eq. (S102), and rearranging, we obtain a bound of the form

$$N_{\text{ph}} \lesssim f(\{N_j^{\beta x}\}_{j,\beta}, N_{\text{key}}^{\text{det}}) =: N_{\text{ph}}^{\text{U}}, \tag{S103}$$

as desired.

## E. General finite-key analysis for prepare-and-measure protocols

Here, we extend the general analysis presented in the previous Section to the finite-key regime. First, we introduce the concentration inequalities employed and then, show how to derive an upper bound on the number of phase errors  $N_{\text{ph}}$  for a general P&M protocol. Finally, we plot the secret-key rate obtainable for the particular BB84 scenario considered in the Main Text as a function of the total number of transmitted signals  $N$ .

### 1. Concentration inequalities

Let  $\xi_1, \xi_2, \dots, \xi_n$  be a sequence of independent Bernoulli random variables and let  $\xi := \sum_{u=1}^n \xi_u$ , whose expectation value is  $\mu_\xi := E[\xi]$ . Also, let us define the notation  $L \stackrel{\epsilon}{\leq} R$  to mean that the event  $L \leq R$  occurs except with probability at most  $\epsilon$ , i.e.,  $\Pr[L > R] \leq \epsilon$ .

- *Chernoff's bound* [S16]

This bound states that for a known  $\mu_\xi$ , we have that

$$\mu_\xi - \Delta_C^-(\mu_\xi) \stackrel{\epsilon_C}{\leq} \xi \stackrel{\epsilon_C}{\leq} \mu_\xi + \Delta_C^+(\mu_\xi), \tag{S104}$$

where  $\Delta_C^-(x) = \sqrt{2x \ln(1/\epsilon_C)}$  and  $\Delta_C^+(x) = \sqrt{3x \ln(1/\epsilon_C)}$ .

- *Hoeffding's bound* [S23]

This bound states that

$$\xi - \Delta_H(n) \stackrel{\epsilon_H}{\leq} \mu_\xi \stackrel{\epsilon_H}{\leq} \xi + \Delta_H(n), \tag{S105}$$

where  $\Delta_H(n) = \sqrt{n \ln(1/\epsilon_H)/2}$ .

Let us now consider  $\zeta_1, \zeta_2, \dots, \zeta_n$  to be *any* (not necessarily independent) sequence of Bernoulli random variables and let  $\{\mathcal{F}_l\}_{l=1}^n$  be a filtration identifying random variables, including  $\zeta_1, \zeta_2, \dots, \zeta_n$ . That is,  $\mathcal{F}_l$  is a  $\sigma$ -algebra satisfying  $\mathcal{F}_{l-1} \subseteq \mathcal{F}_l$  and  $E[\zeta_{l'}|\mathcal{F}_l] = \zeta_{l'}$  for  $l' \leq l$ . Also, let  $\Lambda_l = \sum_{u=1}^l \zeta_u$ , with  $l \leq n$ . Below, we state a specific result that can be directly derived from Azuma's inequality [S24]; for simplicity, in this paper, we refer to this as Azuma's inequality.

- *Azuma's inequality*

This bound states that

$$\Pr\left(\Lambda_n - \sum_{u=1}^n \Pr(\zeta_u = 1|\mathcal{F}_{u-1}) > b\sqrt{n}\right) \leq \exp\left(-\frac{b^2}{2}\right), \text{ and} \quad (\text{S106})$$

$$\Pr\left(\sum_{u=1}^n \Pr(\zeta_u = 1|\mathcal{F}_{u-1}) - \Lambda_n > b\sqrt{n}\right) \leq \exp\left(-\frac{b^2}{2}\right), \quad (\text{S107})$$

for any  $b \in (0, 1)$ . In particular, this means that

$$\Lambda_n - \Delta_A(n) \leq \sum_{\epsilon_A} \sum_{u=1}^n \Pr(\zeta_u = 1|\mathcal{F}_{u-1}) \leq \Lambda_n + \Delta_A(n), \quad (\text{S108})$$

where  $\Delta_A(n) = \sqrt{2n \ln(1/\epsilon_A)}$ .

Note that Chernoff's and Hoeffding's bounds only apply to independent random variables. However, Azuma's inequality applies to *any* random variables, including those that are correlated, and therefore it can be used to evaluate the security of our analysis against coherent attacks in the finite-key regime. Recently, another concentration inequality for sums of dependent random variables has been proposed by Kato [S25]. This result can be seen as a refined form of Azuma's inequality that is much tighter when the expected value of the sum of the random variables is low. For a complete description of the application of this inequality to QKD, see Appendix F in [S15].

## 2. Analysis for a general prepare-and-measure protocol

As shown in Section SE1, in the finite-key regime, the Coin Protocol inequality becomes

$$N_{Z_C=0}^{\text{err}} - \Delta_A \leq_{6\epsilon_A} (N_{Z_C=0}^{\text{det}} + \Delta_A) G_+ \left( \frac{N_{Z_C=1}^{\text{err}} + \Delta_A}{N_{Z_C=1}^{\text{det}} - \Delta_A}, 1 - \frac{2p_{Z_C}(N_{X_C=1} + \Delta_A)}{p_{X_C}(N_{Z_C}^{\text{det}} - \Delta_A)} \right), \quad (\text{S109})$$

where we have employed Azuma's inequality using  $\Delta_A := \Delta_A(N^{\text{det}})$  with  $N^{\text{det}}$  denoting the number of detected rounds. By substituting the definition of  $N_{Z_C=0}^{\text{err}}$  in Eq. (S100) into Eq. (S109) and rearranging, we obtain

$$N_{\text{ph}, \text{TAR}, Z_C} \leq_{6\epsilon_A} (N_{Z_C=0}^{\text{det}} + \Delta_A) G_+ \left( \frac{N_{Z_C=1}^{\text{err}} + \Delta_A}{N_{Z_C=1}^{\text{det}} - \Delta_A}, 1 - \frac{2p_{Z_C}(N_{X_C=1} + \Delta_A)}{p_{X_C}(N_{Z_C}^{\text{det}} - \Delta_A)} \right) + \Delta_A - \sum_{\alpha \in \{0,1\}} \sum_{j \in \mathcal{C}_{\text{TAR}}^{(\alpha)}} N_{j, \text{TAR}, \alpha, Z_C}^{(\alpha \oplus 1)_X}, \quad (\text{S110})$$

where we have defined  $N_{\text{ph}, \text{TAR}, Z_C} := \sum_{\alpha \in \{0,1\}} N_{\text{vir}, \alpha, \text{TAR}, \alpha, Z_C}^{(\alpha \oplus 1)_X}$ . Although the values of  $N_{Z_C=\alpha}^{\text{err}}$ ,  $N_{Z_C=\alpha}^{\text{det}}$ ,  $N_{X_C=1}$ ,  $N_{Z_C}^{\text{det}} = \sum_{\alpha \in \{0,1\}} N_{Z_C=\alpha}^{\text{det}}$  and  $N_{j, \text{TAR}, \alpha, Z_C}^{(\alpha \oplus 1)_X}$  in Eq. (S110) are not directly observable in the experiment, we can apply the Chernoff bound to establish lower and upper limits for these variables, such that an upper bound on  $N_{\text{ph}, \text{TAR}, Z_C}$  can be obtained. In particular, we have that

$$N_{X_C=1} \leq_{\epsilon_C} \hat{N}_{X_C=1} + \Delta_C^+(\hat{N}_{X_C=1}) =: \bar{N}_{X_C=1}, \quad (\text{S111})$$

where  $\hat{N}_{X_C=1} = N p_C p_{X_C} \Delta/2$ . Also, we have that

$$\begin{aligned}
N_{Z_C=1}^{\text{err}} &\leq_{v_r \epsilon_C} \bar{N}_{Z_C=1}^{\text{err}} := \sum_{\alpha \in \{0,1\}} \sum_{j \in \mathcal{C}_{\text{Ref}}^{(\alpha)}} \bar{N}_{j, \text{REF} \alpha, Z_C}^{(\alpha \oplus 1)X}, \\
N_{Z_C=0}^{\text{det}} &\leq_{(v_t+1)\epsilon_C} \bar{N}_{Z_C=0}^{\text{det}} := \bar{N}_{\text{key}, \text{TAR}, Z_C}^{\text{det}} + \sum_{\alpha \in \{0,1\}} \sum_{j \in \mathcal{C}_{\text{TAR}}^{(\alpha)}} \bar{N}_{j, \text{TAR} \alpha, Z_C}^{\text{det}}, \\
N_{Z_C=0}^{\text{det}} &\geq_{(v_t+1)\epsilon_C} \underline{N}_{Z_C=0}^{\text{det}} := \underline{N}_{\text{key}, \text{TAR}, Z_C}^{\text{det}} + \sum_{\alpha \in \{0,1\}} \sum_{j \in \mathcal{C}_{\text{TAR}}^{(\alpha)}} \underline{N}_{j, \text{TAR} \alpha, Z_C}^{\text{det}}, \\
N_{Z_C=1}^{\text{det}} &\geq_{v_r \epsilon_C} \underline{N}_{Z_C=1}^{\text{det}} := \sum_{\alpha \in \{0,1\}} \sum_{j \in \mathcal{C}_{\text{Ref}}^{(\alpha)}} \underline{N}_{j, \text{REF} \alpha, Z_C}^{\text{det}},
\end{aligned} \tag{S112}$$

where we have used Eq. (S100) and

$$\begin{aligned}
\underline{N}_{l,t,Z_C}^{\beta X} &:= \hat{N}_{l,t,Z_C}^{\beta X} - \Delta_C^-(\hat{N}_{l,t,Z_C}^{\beta X}) \leq_{\epsilon_C} N_{l,t,Z_C}^{\beta X} \leq_{\epsilon_C} \hat{N}_{l,t,Z_C}^{\beta X} + \Delta_C^+(\hat{N}_{l,t,Z_C}^{\beta X}) =: \bar{N}_{l,t,Z_C}^{\beta X}, \\
\underline{N}_{l,t,Z_C}^{\text{det}} &:= \hat{N}_{l,t,Z_C}^{\text{det}} - \Delta_C^-(\hat{N}_{l,t,Z_C}^{\text{det}}) \leq_{\epsilon_C} N_{l,t,Z_C}^{\text{det}} \leq_{\epsilon_C} \hat{N}_{l,t,Z_C}^{\text{det}} + \Delta_C^+(\hat{N}_{l,t,Z_C}^{\text{det}}) =: \bar{N}_{l,t,Z_C}^{\text{det}}, \\
\underline{N}_{\text{key}, \text{TAR}, Z_C}^{\text{det}} &:= \hat{N}_{\text{key}, \text{TAR}, Z_C}^{\text{det}} - \Delta_C^-(\hat{N}_{\text{key}, \text{TAR}, Z_C}^{\text{det}}) \leq_{\epsilon_C} N_{\text{key}, \text{TAR}, Z_C}^{\text{det}} \leq_{\epsilon_C} \hat{N}_{\text{key}, \text{TAR}, Z_C}^{\text{det}} + \Delta_C^+(\hat{N}_{\text{key}, \text{TAR}, Z_C}^{\text{det}}) =: \bar{N}_{\text{key}, \text{TAR}, Z_C}^{\text{det}},
\end{aligned} \tag{S113}$$

with  $v_r = |\mathcal{C}_{\text{Ref}}^{(0)}| + |\mathcal{C}_{\text{Ref}}^{(1)}|$ ,  $v_t = |\mathcal{C}_{\text{TAR}}^{(0)}| + |\mathcal{C}_{\text{TAR}}^{(1)}|$ ,  $\hat{N}_{l,t,Z_C}^{\beta X} = p_{Z_C} p_{t|l} N_l^{\beta X}$ ,  $\hat{N}_{l,t,Z_C}^{\text{det}} = p_{Z_C} p_{t|l} N_l^{\text{det}}$ ,  $N_{\text{key}, \text{TAR}, Z_C}^{\text{det}} = \sum_{\alpha \in \{0,1\}} N_{\text{vir} \alpha, \text{TAR} \alpha, Z_C}^{\text{det}}$ , and  $\hat{N}_{\text{key}, \text{TAR}, Z_C}^{\text{det}} = p_{Z_C} p_{\text{TAR}|\text{vir}} N_{\text{key}}^{\text{det}}$ . By substituting Eqs. (S111) to (S113) into Eq. (S110), we get that

$$\begin{aligned}
N_{\text{ph}, \text{TAR}, Z_C} &\leq_{6\epsilon_A + (2v_r + 3v_t + 3)\epsilon_C} (\bar{N}_{Z_C=0}^{\text{det}} + \Delta_A) G + \left( \frac{\bar{N}_{Z_C=1}^{\text{err}} + \Delta_A}{\underline{N}_{Z_C=1}^{\text{det}} - \Delta_A}, 1 - \frac{2p_{Z_C}(\bar{N}_{X_C=1} + \Delta_A)}{p_{X_C}(\underline{N}_{Z_C=0}^{\text{det}} + \underline{N}_{Z_C=1}^{\text{det}} - \Delta_A)} \right) \\
&\quad + \Delta_A - \sum_{\alpha \in \{0,1\}} \sum_{j \in \mathcal{C}_{\text{TAR}}^{(\alpha)}} \underline{N}_{j, \text{TAR} \alpha, Z_C}^{(\alpha \oplus 1)X}.
\end{aligned} \tag{S114}$$

Then, we can obtain an expression in terms of  $N_{\text{ph}}$  by using our knowledge of  $N_{\text{ph}, \text{TAR}, Z_C}$  and Hoeffding's bound such that

$$N_{\text{ph}, \text{TAR}, Z_C} \geq_{\epsilon_H} p_{Z_C} p_{\text{TAR}|\text{vir}} N_{\text{ph}} - \Delta_H(N_{\text{ph}}) \geq p_{Z_C} p_{\text{TAR}|\text{vir}} N_{\text{ph}} - \Delta_H(N_{\text{key}}^{\text{det}}), \tag{S115}$$

where in the last inequality we have upper bounded  $\Delta_H(N_{\text{ph}})$  by  $\Delta_H(N_{\text{key}}^{\text{det}})$ , where  $N_{\text{key}}^{\text{det}}$  is the number of detected key rounds. Finally, by substituting Eq. (S115) into Eq. (S114) and rearranging, we obtain an upper bound on the number of phase errors:

$$\begin{aligned}
N_{\text{ph}} &\leq_{\epsilon_{\text{tot}}} \frac{1}{p_{Z_C} p_{\text{TAR}|\text{vir}}} \left[ (\bar{N}_{Z_C=0}^{\text{det}} + \Delta_A) G + \left( \frac{\bar{N}_{Z_C=1}^{\text{err}} + \Delta_A}{\underline{N}_{Z_C=1}^{\text{det}} - \Delta_A}, 1 - \frac{2p_{Z_C}(\bar{N}_{X_C=1} + \Delta_A)}{p_{X_C}(\underline{N}_{Z_C=0}^{\text{det}} + \underline{N}_{Z_C=1}^{\text{det}} - \Delta_A)} \right) \right. \\
&\quad \left. - \sum_{\alpha \in \{0,1\}} \sum_{j \in \mathcal{C}_{\text{TAR}}^{(\alpha)}} \underline{N}_{j, \text{TAR} \alpha, Z_C}^{(\alpha \oplus 1)X} + \Delta_A + \Delta_H(N_{\text{key}}^{\text{det}}) \right] =: N_{\text{ph}}^{\text{U}},
\end{aligned} \tag{S116}$$

where  $\epsilon_{\text{tot}} := 6\epsilon_A + (2v_r + 3v_t + 3)\epsilon_C + \epsilon_H$  is the sum of the failure probabilities of all the concentration inequalities applied. After performing error correction, error verification and privacy amplification, Alice and Bob obtain a secret key of length

$$N_{\text{sec}} = N_{\text{key}}^{\text{det}} [1 - h(e_{\text{ph}}^{\text{U}})] - \lambda_{\text{EC}} - \log_2 \frac{1}{\epsilon_{\text{corr}}} - \log_2 \frac{1}{\epsilon_{\text{PA}}}, \tag{S117}$$

where  $e_{\text{ph}}^{\text{U}} := N_{\text{ph}}^{\text{U}}/N_{\text{key}}^{\text{det}}$  is the upper bound on the phase-error rate,  $\lambda_{\text{EC}} = fh(e_Z)$  is the cost of error correction, with  $f$  denoting the error correction efficiency and  $e_Z$  the bit-error rate,  $\epsilon_{\text{corr}}$  is the probability that the reconciled keys are not identical (due to the failure of error verification) and  $\epsilon_{\text{PA}}$  is a free parameter that can be regarded as the failure

probability of privacy amplification. It is known [S26] that, if  $N_{\text{ph}}$  is bounded such that  $\Pr[N_{\text{ph}}^{\text{U}} > N_{\text{ph}}] \leq \epsilon_{\text{tot}}$  and the secret-key length is set as in Eq. (S117), then the protocol is  $\epsilon_{\text{secre}}$ -secret, with  $\epsilon_{\text{secre}} = \sqrt{2\sqrt{\epsilon_{\text{tot}}} + \epsilon_{\text{PA}}}$ . Since the protocol is also  $\epsilon_{\text{corr}}$ , then it is  $\epsilon_s$ -secure with  $\epsilon_s = \epsilon_{\text{corr}} + \epsilon_{\text{secre}}$ .

We remark that the key rate formula in Eq. (S117) assumes the phase-error correction security framework [S13, S26]. However, our security proof is compatible with the leftover hashing lemma in combination with the entropic uncertainty relation (EUR) [S8–S10]. We remark that previous works have shown that a bound on the phase-error rate such as the one derived in our work is enough to guarantee security in the variable length scenario [S27, S28].

### 3. Secret-key rate for a particular BB84 scenario

To evaluate the secret-key rate offered by our analysis in the finite-key regime we consider, as an example, the BB84 scenario introduced in the Main Text (see also Section SM1 C). To simulate the data that one would obtain in the Actual Protocol, we use the channel model in Section SE3 A. For this, we assume the following experimental parameters:  $f = 1.16$ , dark count probability  $p_d = 10^{-8}$  [S29, S30] and detector efficiency  $\eta_d = 0.73$  [S30]. Moreover, we select  $\epsilon_{\text{secre}} = \epsilon_{\text{corr}} = 10^{-10}$  [S31] and for simplicity, we set  $\epsilon_C = \epsilon_H = \epsilon_A =: \hat{\epsilon}$ , from which it follows that  $\epsilon_{\text{tot}} = 19\hat{\epsilon}$ . For simplicity, we also assume that  $\epsilon_{\text{PA}} = \epsilon_{\text{tot}}$ , and therefore  $\epsilon_{\text{tot}} = \epsilon_{\text{secre}}^2/4$ . In the simulations, we optimize over the probabilities  $p_{Z_A}$ ,  $p_{Z_B}$  and  $p_{Z_C}$ , and consider different values of the block size  $N$ , which represents the total number of emitted signals. To evaluate the achievable secret-key rate under different amounts of information leakage, we fix the qubit flaws to  $\delta = 0.063$  [S32, S33] and take  $\epsilon \in \{10^{-3}, 10^{-6}\}$ . The results obtained are shown in Fig. S4, where a reasonable finite-key scaling is achieved for practical values of  $N$ . Also, as expected, a lower value of  $\epsilon$  results in higher secret-key rates (see also Fig. 1 in the Main Text).

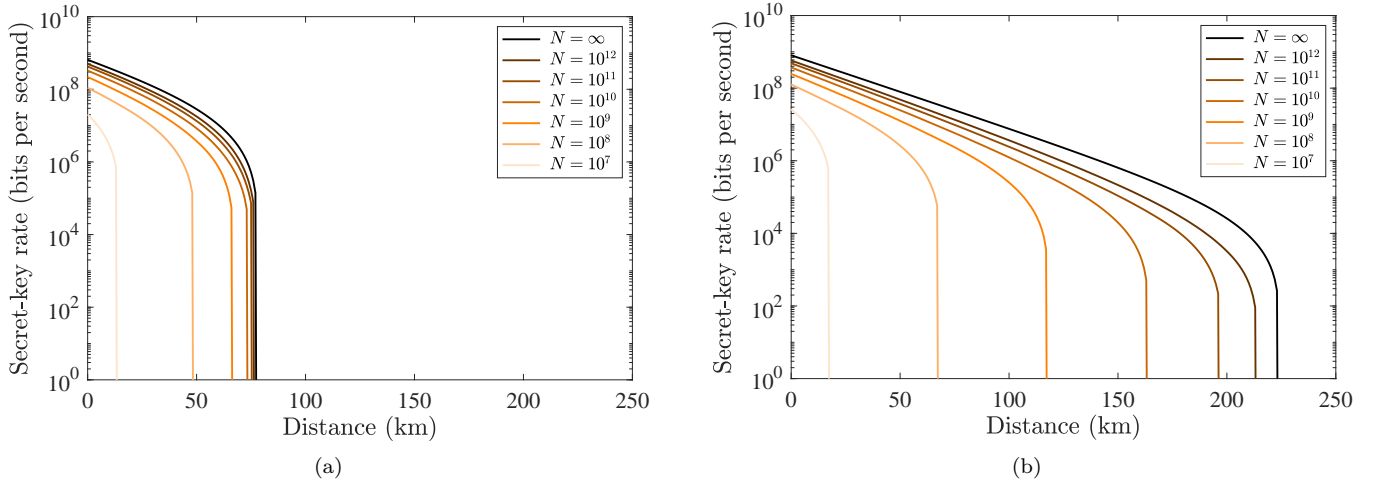

Figure S4. Finite-size secret-key rate as a function of distance when applying our analysis with Azuma’s inequality for different values of the block size  $N$ . We assume that  $\delta = 0.063$  and take (a)  $\epsilon = 10^{-3}$  and (b)  $\epsilon = 10^{-6}$ .

The finite-key analysis presented in the previous Section can also be carried out using Kato’s rather than Azuma’s inequality. As explained above, the former can offer a tighter bound on  $N_{\text{ph}}$ , resulting in higher secret-key rates. However, we remark that its use requires an extra condition: the users need to make an attempt at predicting the results that they will obtain in the QKD session before they actually run the protocol. This inequality is tight only if these predictions are close to the actual experimental data. In Fig. S5, we present the results obtained when employing Kato’s inequality under the assumption that the users make perfect predictions. This figure shows a considerable improvement in performance when compared to Fig. S4, especially for  $\epsilon = 10^{-6}$  and lower values of  $N$ .

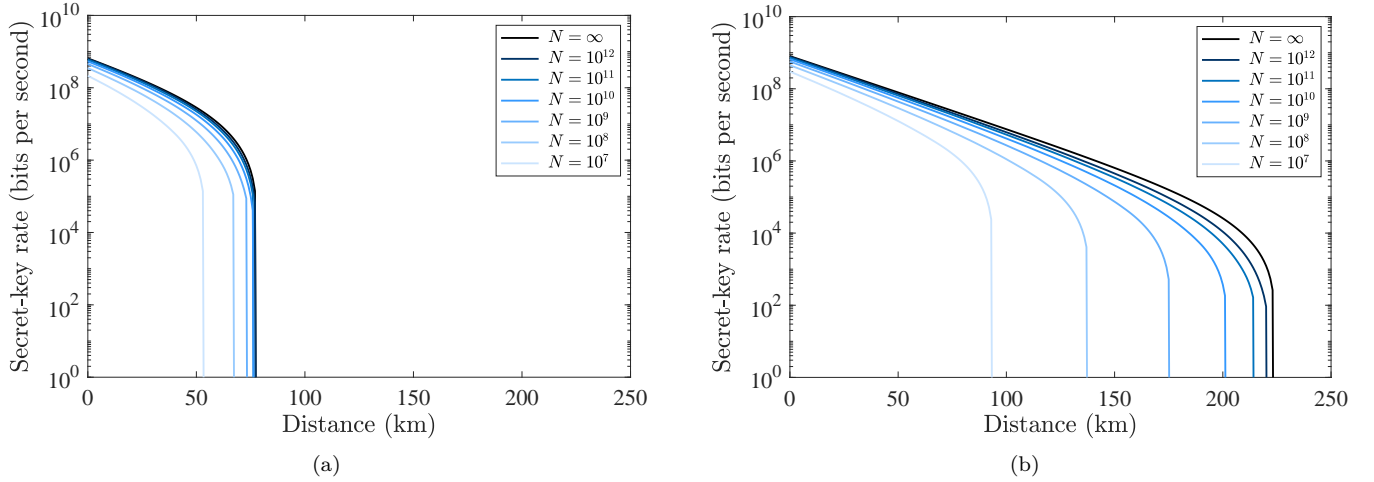

Figure S5. Finite-size secret-key rate as a function of distance when applying our analysis with Kato’s inequality for different values of the block size  $N$ . We assume that  $\delta = 0.063$  and take (a)  $\epsilon = 10^{-3}$  and (b)  $\epsilon = 10^{-6}$ .

## SM2. SECURITY PROOF FOR MDI-TYPE PROTOCOLS

### A. Protocol description, assumptions and security framework

#### 1. Protocol description

As in the P&M case, our proof is applicable irrespectively of whether Alice and Bob emit three or four different states each. Without loss of generality, in the former (latter) case, we label these states as  $j \in \{0_Z, 1_Z, 0_X\}$  ( $j \in \{0_Z, 1_Z, 0_X, 1_X\}$ ). States such that  $j \in \{0_Z, 1_Z\}$  ( $j \notin \{0_Z, 1_Z\}$ ) are considered  $Z$ -basis ( $X$ -basis) states. For simplicity, we assume that Alice and Bob select the  $Z$ -basis states with probability  $p_Z/2$  each.

---

#### MDI-type Protocol

1. **Quantum communication:** For each of the  $N$  rounds: (a) Alice (Bob) chooses a state from the set  $\{|\psi_j\rangle_{B_a}\}_j$  ( $\{|\psi_j\rangle_{B_b}\}_j$ ) with probability  $p_j$ , and sends it to the middle node Charlie through a quantum channel. (b) Charlie performs a measurement on the incoming signals and announces the result.
  2. **Basis and bit announcement:** For each round in which Charlie announced a successful detection, Alice (Bob) announces the  $Z$  basis if her (his) setting choice was  $j \in \{0_Z, 1_Z\}$ , or the  $X$  basis otherwise. Then, for each detected round in which both users announced the  $Z$  basis, Alice assigns the round to “key” (“test”) with probability  $p_{\text{key}|Z}$  ( $p_{\text{test}|Z} = 1 - p_{\text{key}|Z}$ ), and announces this information. All the other detected rounds are assigned to “test”. Then, the users announce their setting choices for the rounds assigned to “test”, and define their sifted keys as the bit outcomes of the rounds assigned to “key”.
  3. **Parameter estimation:** The users quantify the number of events  $N_{ij}^{\text{det}}$  in which Alice’s (Bob’s) setting choice was  $i$  ( $j$ ), Charlie announced a detection, and the round was assigned to “test”; the number of detected key events  $N_{\text{key}}^{\text{det}}$  (i.e., the length of the sifted key); and the total number of detected rounds  $N^{\text{det}} := N_{\text{key}}^{\text{det}} + \sum_{i,j} N_{ij}^{\text{det}}$ . Then, they use this information to obtain an upper bound on the phase-error rate  $e_{\text{ph}}$  of the sifted key.
  4. **Data post-processing:** Alice sends Bob syndrome information about her sifted key through an authenticated classical channel for him to correct his own sifted key. After, Alice and Bob perform error verification by computing a hash of their corrected keys using a random two-universal hash function and then check whether they are identical. If so, Alice and Bob perform privacy amplification by employing a random two-universal hash function to extract a secure key pair from the corrected keys. Otherwise, they abort the protocol.
- 

As for the P&M scenario, for simplicity, we assume that the users perform error correction for a predetermined bit-error rate, which is inferred from *a priori* knowledge of the channel. However, as explained in Section SM1 A 1, after

a few modifications, our analysis could also be applied to the case in which the users sacrifice a small fraction of the sifted key to estimate its bit-error rate.

## 2. Assumptions

For MDI-type protocols, our analysis only requires the following assumption:

(A1) *Bounded fidelity to qubit states:* Alice's (Bob's) emitted states  $\{|\psi_j\rangle_{B_a}\}_j$  ( $\{|\psi_j\rangle_{B_b}\}_j$ ) are  $\epsilon$ -close (in terms of fidelity) to some characterized qubit states  $\{|\phi_j\rangle_{B_a}\}_j$  ( $\{|\phi_j\rangle_{B_b}\}_j$ ), i.e., for all  $j$ ,

$$|\langle\phi_j|\psi_j\rangle_{B_a(B_b)}|^2 \geq 1 - \epsilon, \quad (\text{S118})$$

where  $\epsilon$  is known. Again, for notational simplicity, we consider throughout the proof that the states emitted by Alice and Bob are pure and identical for all rounds. However, as explained in the Main Text and Methods, our security analysis can be trivially extended without any modifications to the scenario in which the states are mixed and/or different for different rounds (see Eq. (1) in the Main Text). Moreover, with a simple modification to Eq. (S118) and to the post-processing step of the protocol, our analysis can be applied in the presence of setting-dependent pulse correlations i.e., when the state emitted in a given round depends on the setting choices made in previous rounds. For more information, see Section SM3.

As in the P&M scenario, Eq. (S118) implies that we can assume that the states emitted by Alice (Bob) have the form

$$|\psi_j\rangle_{B_a(B_b)} = \sqrt{1 - \epsilon} |\phi_j\rangle_{B_a(B_b)} + \sqrt{\epsilon} |\phi_j^\perp\rangle_{B_a(B_b)}, \quad (\text{S119})$$

where  $|\phi_j^\perp\rangle_{B_a(B_b)}$  is a state such that  $\langle\phi_j|\phi_j^\perp\rangle_{B_a(B_b)} = 0$  (see Eq. (S2) for the proof of this claim).

## 3. Security framework

The sifted key is generated from the detected key rounds, which are a subset of the detected rounds in which both Alice and Bob selected the  $Z$  basis. Note that, in these rounds, the users could have replaced their emissions by the generation of the entangled state

$$|\Psi_Z\rangle_{A_u B_u} = \frac{1}{\sqrt{2}} (|0_Z\rangle_{A_u} |\psi_{0_Z}\rangle_{B_u} + e^{i\omega_u} |1_Z\rangle_{A_u} |\psi_{1_Z}\rangle_{B_u}), \quad (\text{S120})$$

where  $\omega_u \in [0, 2\pi)$  can be freely chosen, and  $u \in \{a, b\}$  indicates if the state is prepared by Alice or Bob. The amount of privacy amplification that needs to be applied to the sifted key to turn it into a secret key can be directly related to the error rate that Alice and Bob would have observed if, in these rounds, they had measured systems their  $A_a$  and  $A_b$  in the  $X$  basis, i.e., the phase-error rate  $e_{\text{ph}}$ . For simplicity, here, we will assume that a “phase error” is defined as an event in which Alice and Bob obtain the same  $X$ -basis outcome<sup>4</sup>, i.e., both obtain  $0_X$  or both obtain  $1_X$ . Note that this entanglement-based view is equivalent to a scenario in which, in the key rounds, Alice and Bob emit the virtual states

$$\begin{aligned} |\psi_{\text{vir}0}\rangle_{B_u} &= \frac{1}{2\sqrt{q_{\text{vir}0}^{\psi,u}}} (|\psi_{0_Z}\rangle_{B_u} + e^{i\omega_u} |\psi_{1_Z}\rangle_{B_u}), \\ |\psi_{\text{vir}1}\rangle_{B_u} &= \frac{1}{2\sqrt{q_{\text{vir}1}^{\psi,u}}} (|\psi_{0_Z}\rangle_{B_u} - e^{i\omega_u} |\psi_{1_Z}\rangle_{B_u}), \end{aligned} \quad (\text{S121})$$

---

<sup>4</sup> In general, the appropriate definition of a phase error depends on the MDI protocol under consideration. In some protocols, such as the standard MDI-QKD [S7], the definition of a phase error actually depends on the specific announcement made by Charlie. In this case, one should define separate sifted key pairs according to the specific announcement made by Charlie, and apply our analysis to compute a bound on the phase-error rate separately for each sifted key pair. On the other hand, for scenarios in which the definition of a phase error does not depend on the specific announcement made by Charlie, such as the coherent-light-based MDI protocol [S34] considered in Section SM4A, this separation is not necessary.

with

$$\begin{aligned} q_{\text{vir}0}^{\psi,u} &= \frac{1}{4} \left\| |\psi_{0z}\rangle_{B_u} + e^{i\omega_u} |\psi_{1z}\rangle_{B_u} \right\|^2 = \frac{1}{2} (1 + \text{Re} \{ e^{i\omega_u} \langle \psi_{0z} | \psi_{1z} \rangle_{B_u} \}), \\ q_{\text{vir}1}^{\psi,u} &= \frac{1}{4} \left\| |\psi_{0z}\rangle_{B_u} - e^{i\omega_u} |\psi_{1z}\rangle_{B_u} \right\|^2 = \frac{1}{2} (1 - \text{Re} \{ e^{i\omega_u} \langle \psi_{0z} | \psi_{1z} \rangle_{B_u} \}). \end{aligned} \quad (\text{S122})$$

### B. Constructing the reference and target states, and the Virtual Protocol with tag assignment

The starting point of the analysis are the MDI loss-tolerant formulas

$$\begin{aligned} |\phi_{\text{vir}00}\rangle_{B_a B_b} &+ \sum_{(i,j) \in \mathcal{C}_{\text{Tar}}^{(00)}} c_{ij}^{(00)} |\phi_{ij}\rangle_{B_a B_b} = \sum_{(i,j) \in \mathcal{C}_{\text{Ref}}^{(00)}} c_{ij}^{(00)} |\phi_{ij}\rangle_{B_a B_b}, \\ |\phi_{\text{vir}11}\rangle_{B_a B_b} &+ \sum_{(i,j) \in \mathcal{C}_{\text{Tar}}^{(11)}} c_{ij}^{(11)} |\phi_{ij}\rangle_{B_a B_b} = \sum_{(i,j) \in \mathcal{C}_{\text{Ref}}^{(11)}} c_{ij}^{(11)} |\phi_{ij}\rangle_{B_a B_b}, \\ |\phi_{\text{vir}10}\rangle_{B_a B_b} &+ \sum_{(i,j) \in \mathcal{C}_{\text{Tar}}^{(10)}} c_{ij}^{(10)} |\phi_{ij}\rangle_{B_a B_b} = \sum_{(i,j) \in \mathcal{C}_{\text{Ref}}^{(10)}} c_{ij}^{(10)} |\phi_{ij}\rangle_{B_a B_b}, \\ |\phi_{\text{vir}01}\rangle_{B_a B_b} &+ \sum_{(i,j) \in \mathcal{C}_{\text{Tar}}^{(01)}} c_{ij}^{(01)} |\phi_{ij}\rangle_{B_a B_b} = \sum_{(i,j) \in \mathcal{C}_{\text{Ref}}^{(01)}} c_{ij}^{(01)} |\phi_{ij}\rangle_{B_a B_b}, \end{aligned} \quad (\text{S123})$$

with  $c_{ij}^{(\alpha\beta)} \geq 0$  for all  $i, j, \alpha, \beta$ , and where we have defined  $|\phi_{ij}\rangle_{B_a B_b} = |\phi_i\rangle_{B_a} \otimes |\phi_j\rangle_{B_b}$  and  $|\phi_{\text{vir}\alpha\beta}\rangle_{B_a B_b} = |\phi_{\text{vir}\alpha}\rangle_{B_a} \otimes |\phi_{\text{vir}\beta}\rangle_{B_b}$ . To obtain these expressions, one should compute the P&M loss-tolerant formulas in Eq. (S70) for both Alice and Bob, isolate the terms  $|\phi_{\text{vir}\alpha}\rangle_{B_a}$ , take the tensor products of the resulting left- and right-hand sides, and reorganize terms.

Using the formulas in Eq. (S123) and following a similar approach to that described in Section SM1 D, we construct the following reference and target states:

$$|\Psi_{\text{Tar}}\rangle_{DAB} = 1/\sqrt{C} \left[ \sum_{\alpha,\beta} |\alpha\beta\rangle_{D_a D_b} \left( \sqrt{q_{\text{vir}\alpha\beta}^{\psi}} |0\rangle_A |\psi_{\text{vir}\alpha\beta}\rangle_{B_a B_b} + \sqrt{q_{\text{vir}\alpha\beta}^{\phi}} \sum_{(i,j) \in \mathcal{C}_{\text{Tar}}^{(\alpha\beta)}} \sqrt{c_{ij}^{(\alpha\beta)}} |k_{ij}^{(\alpha\beta)}\rangle_A |\psi_{ij}\rangle_{B_a B_b} \right) \right], \quad (\text{S124})$$

$$|\Psi_{\text{Ref}}\rangle_{DAB} = 1/\sqrt{C} \left[ \sum_{\alpha,\beta} \sqrt{q_{\text{vir}\alpha\beta}^{\phi}} |\alpha\beta\rangle_{D_a D_b} \left( \sum_{(i,j) \in \mathcal{C}_{\text{Ref}}^{(\alpha\beta)}} \sqrt{c_{ij}^{(\alpha\beta)}} |k'_{ij}^{(\alpha\beta)}\rangle_A |\psi_{ij}\rangle_{B_a B_b} \right) \right], \quad (\text{S125})$$

where we have defined  $D := D_a D_b$ ,  $B := B_a B_b$ ,  $|\psi_{ij}\rangle_{B_a B_b} := |\psi_i\rangle_{B_a} \otimes |\psi_j\rangle_{B_b}$ ,  $|\psi_{\text{vir}\alpha\beta}\rangle_{B_a B_b} := |\psi_{\text{vir}\alpha}\rangle_{B_a} \otimes |\psi_{\text{vir}\beta}\rangle_{B_b}$ ,  $q_{\text{vir}\alpha\beta}^{\psi} := q_{\text{vir}\alpha}^{\psi} q_{\text{vir}\beta}^{\psi}$ ,  $q_{\text{vir}\alpha\beta}^{\phi} := q_{\text{vir}\alpha}^{\phi} q_{\text{vir}\beta}^{\phi}$ , and

$$C = 1 + \sum_{\alpha,\beta} \sum_{(i,j) \in \mathcal{C}_{\text{Tar}}^{(\alpha\beta)}} q_{\text{vir}\alpha\beta}^{\phi} c_{ij}^{(\alpha\beta)} = \sum_{\alpha,\beta} \sum_{(i,j) \in \mathcal{C}_{\text{Ref}}^{(\alpha\beta)}} q_{\text{vir}\alpha\beta}^{\phi} c_{ij}^{(\alpha\beta)}. \quad (\text{S126})$$

The sets  $\{|0\rangle_A\} \cup \{|k_{ij}^{(\alpha\beta)}\rangle_A\}_{ij \in \mathcal{C}_{\text{Tar}}^{(\alpha\beta)}}$  and  $\{|k'_{ij}^{(\alpha\beta)}\rangle_A\}_{ij \in \mathcal{C}_{\text{Ref}}^{(\alpha\beta)}}$  are two orthonormal bases that should be appropriately chosen such that  $|\Psi_{\text{Tar}}\rangle_{DAB} = |\Psi_{\text{Ref}}\rangle_{DAB}$  when  $\epsilon = 0$ . These orthonormal bases must exist due to the equalities in Eq. (S123). As in the P&M scenario, the quantum coin can then be defined as

$$|\Psi_{\text{coin}}\rangle_{CDAB} = \frac{1}{\sqrt{2}} (|0z\rangle_C |\Psi_{\text{Tar}}\rangle_{DAB} + |1z\rangle_C |\Psi_{\text{Ref}}\rangle_{DAB}). \quad (\text{S127})$$

Now, let us rewrite Eqs. (S124) and (S125) as

$$|\Psi_{\text{Tar}}\rangle_{DAB} = \sum_{\alpha,\beta} \sqrt{p_{\text{Tar}\alpha\beta|\text{Tar}}} |\alpha\beta\rangle_{D_a D_b} |\Psi_{\text{Tar}\alpha\beta}\rangle_{AB}, \quad (\text{S128})$$

$$|\Psi_{\text{Ref}}\rangle_{DAB} = \sum_{\alpha,\beta} \sqrt{p_{\text{Ref}\alpha\beta|\text{Ref}}} |\alpha\beta\rangle_{D_a D_b} |\Psi_{\text{Ref}\alpha\beta}\rangle_{AB}, \quad (\text{S129})$$

where

$$p_{\text{TAR}\alpha\beta|\text{TAR}} = \frac{q_{\text{vir}\alpha\beta}^{\psi} + q_{\text{vir}\alpha\beta}^{\phi} \sum_{(i,j) \in \mathcal{C}_{\text{TAR}}^{(\alpha\beta)}} c_{ij}^{(\alpha\beta)}}{C}, \quad (\text{S130})$$

$$p_{\text{REF}\alpha\beta|\text{REF}} = \frac{q_{\text{vir}\alpha\beta}^{\phi} \sum_{(i,j) \in \mathcal{C}_{\text{REF}}^{(\alpha\beta)}} c_{ij}^{(\alpha\beta)}}{C}, \quad (\text{S131})$$

and

$$|\Psi_{\text{TAR}\alpha\beta}\rangle_{AB} = \sqrt{p_{\text{vir}\alpha\beta|\text{TAR}\alpha\beta}} |0\rangle_A |\psi_{\text{vir}\alpha\beta}\rangle + \sum_{(i,j) \in \mathcal{C}_{\text{TAR}}^{(\alpha\beta)}} \sqrt{p_{ij|\text{TAR}\alpha\beta}} |k_{ij}^{(\alpha\beta)}\rangle_A |\psi_{ij}\rangle_{B_a B_b}, \quad (\text{S132})$$

$$|\Psi_{\text{REF}\alpha\beta}\rangle_{AB} = \sum_{(i,j) \in \mathcal{C}_{\text{REF}}^{(\alpha\beta)}} \sqrt{p_{ij|\text{REF}\alpha\beta}} |k_{ij}'^{(\alpha\beta)}\rangle_A |\psi_{ij}\rangle_{B_a B_b}, \quad (\text{S133})$$

with

$$p_{\text{vir}\alpha\beta|\text{TAR}\alpha\beta} = \frac{q_{\text{vir}\alpha\beta}^{\psi}}{q_{\text{vir}\alpha\beta}^{\psi} + q_{\text{vir}\alpha\beta}^{\phi} \sum_{(i,j) \in \mathcal{C}_{\text{TAR}}^{(\alpha\beta)}} c_{ij}^{(\alpha\beta)}}, \quad (\text{S134})$$

$$p_{ij|\text{TAR}\alpha\beta} = \frac{q_{\text{vir}\alpha\beta}^{\phi} c_{ij}^{(\alpha\beta)}}{q_{\text{vir}\alpha\beta}^{\psi} + q_{\text{vir}\alpha\beta}^{\phi} \sum_{(i',j') \in \mathcal{C}_{\text{TAR}}^{(\alpha\beta)}} c_{i'j'}^{(\alpha\beta)}} \quad \text{for } (i,j) \in \mathcal{C}_{\text{TAR}}^{(\alpha\beta)}, \quad (\text{S135})$$

$$p_{ij|\text{REF}\alpha\beta} = \frac{c_{ij}^{(\alpha\beta)}}{\sum_{(i',j') \in \mathcal{C}_{\text{REF}}^{(\alpha\beta)}} c_{i'j'}^{(\alpha\beta)}} \quad \text{for } (i,j) \in \mathcal{C}_{\text{REF}}^{(\alpha\beta)}. \quad (\text{S136})$$

In the Virtual Protocol, we can label the emissions in the key rounds by  $l \in \{\text{vir}\alpha\beta\}_{\alpha\beta}$  and the emissions in the test rounds by  $l \in \{ij\}_{ij}$ . Each emission with label  $l$  should be assigned a tag  $t \in \{\text{TAR00}, \text{TAR01}, \text{TAR10}, \text{TAR11}, \text{REF00}, \text{REF01}, \text{REF10}, \text{REF11}\}$  with probability

$$p_{t|l} = \frac{p_t p_{l|t}}{p_l}, \quad (\text{S137})$$

where  $p_{l|t}$  is given by Eqs. (S134) to (S136) and  $p_t$  is the overall probability to assign tag  $t$ . Also, for  $l \in \{0_Z 0_Z, 0_Z 1_Z, 1_Z 0_Z, 1_Z 1_Z\}$ ,  $p_l$  corresponds to the probability that in the Actual Protocol Alice and Bob emit these states *and* the round is a test round, i.e.,  $p_{0_Z 0_Z} = p_{0_Z 1_Z} = p_{1_Z 0_Z} = p_{1_Z 1_Z} = p_Z^2 p_{\text{test}|Z}/4$ . Similarly, for  $l \in \{\text{vir}\alpha\beta\}_{\alpha\beta}$ , we have that  $p_{\text{vir}\alpha\beta} = p_Z^2 p_{\text{key}|Z} q_{\text{vir}\alpha\beta}^{\psi}$ . Taking the sum over  $t$  on both sides of Eq. (S137) and using the fact that  $\sum_t p_{t|l} \leq 1$ , we derive the following constraints,

$$\sum_t p_t p_{l|t} \leq p_l, \quad \forall l. \quad (\text{S138})$$

Now, let  $p_{\text{TAR}} = \sum_{\alpha\beta} p_{\text{TAR}\alpha\beta}$  and  $p_{\text{REF}} = \sum_{\alpha\beta} p_{\text{REF}\alpha\beta}$ . We want that

$$p_{\text{TAR}\alpha\beta} = p_{\text{TAR}} p_{\text{TAR}\alpha\beta|\text{TAR}}, \quad (\text{S139})$$

$$p_{\text{REF}\alpha\beta} = p_{\text{REF}} p_{\text{REF}\alpha\beta|\text{REF}}, \quad (\text{S140})$$

where  $p_{\text{TAR}\alpha\beta|\text{TAR}}$  and  $p_{\text{REF}\alpha\beta|\text{REF}}$  are given by Eqs. (S130) and (S131). We also want that  $p_{\text{TAR}} = p_{\text{REF}}$ . Putting everything together, we obtain

$$\begin{aligned} p_l &\geq \sum_t p_t p_{l|t} = \sum_{t \in \{\text{TAR}\alpha\beta\}_{\alpha\beta}} p_t p_{l|t} + \sum_{t \in \{\text{REF}\alpha\beta\}_{\alpha\beta}} p_t p_{l|t} \\ &= \sum_{\alpha\beta} (p_{\text{TAR}} p_{\text{TAR}\alpha\beta|\text{TAR}} p_{l|\text{TAR}\alpha\beta} + p_{\text{REF}} p_{\text{REF}\alpha\beta|\text{REF}} p_{l|\text{REF}\alpha\beta}) \\ &= \sum_{\alpha\beta} (p_{\text{TAR}} p_{\text{TAR}\alpha\beta|\text{TAR}} p_{l|\text{TAR}\alpha\beta} + p_{\text{TAR}} p_{\text{REF}\alpha\beta|\text{REF}} p_{l|\text{REF}\alpha\beta}) \\ &= p_{\text{TAR}} \sum_{\alpha\beta} (p_{\text{TAR}\alpha\beta|\text{TAR}} p_{l|\text{TAR}\alpha\beta} + p_{\text{REF}\alpha\beta|\text{REF}} p_{l|\text{REF}\alpha\beta}). \end{aligned} \quad (\text{S141})$$

The only constraint on the value of  $p_{\text{TAR}}$  is that Eq. (S141) holds for all  $l$ . Therefore, we can set its value as

$$p_{\text{TAR}} = \min_l \frac{p_l}{\sum_{\alpha\beta} (p_{\text{TAR}\alpha\beta|\text{TAR}} p_l |\text{TAR}\alpha\beta + p_{\text{REF}\alpha\beta|\text{REF}} p_l |\text{REF}\alpha\beta)}. \quad (\text{S142})$$

Once we set  $p_{\text{TAR}}$ , the tag selection probabilities  $p_{\text{TAR}\alpha\beta}$  and  $p_{\text{REF}\alpha\beta}$  become fixed, and so do the conditional tag assignment probabilities  $p_{t|l}$ .

Finally, as before, we assume that the users randomly mark each tagged emission as  $Z_C$  with probability  $p_{Z_C}$ , or as  $X_C$  otherwise. By the Chernoff bound [S16], in the limit  $N \rightarrow \infty$ , we have that

$$N_{l,t,Z_C}^{\text{det}} \simeq p_{Z_C} p_{t|l} N_l^{\text{det}}, \quad (\text{S143})$$

where  $N_{l,t,Z_C}^{\text{det}}$  is the total number of emissions with label  $l$  and tag  $t$  that are marked as  $Z_C$ .

### C. Coin protocol

Similarly to the P&M scenario, after the tag assignments explained above, the Virtual Protocol becomes equivalent to the Coin Protocol, in which Alice and Bob generate the quantum coin state  $|\Psi_{\text{coin}}\rangle_{CDAB}$  with probability  $p_C = 2p_{\text{TAR}}$ , and then measure the coin system  $C$  in the  $Z_C$  or  $X_C$  bases with probabilities  $p_{Z_C}$  and  $p_{X_C}$ , respectively. For the rounds in which they measured the coin system  $C$  in  $Z_C$ , they measure their systems  $D_a$  and  $D_b$  in the computational basis, obtaining the measurement outcomes  $\alpha$  and  $\beta$ , respectively, and check whether or not their result is such that  $\alpha = \beta$  (error) or  $\alpha \neq \beta$  (no error). Also, if  $Z_C = 0$ , they measure system  $A$  in the  $\{|0\rangle_A\} \cup \{|k_{ij}^{(\alpha\beta)}\rangle_A\}_{ij \in \mathcal{C}_{\text{TAR}}^{(\alpha\beta)}}$  basis, and if  $Z_C = 1$ , they measure system  $A$  in the  $\{|k'_{ij}^{(\alpha\beta)}\rangle_A\}_{ij \in \mathcal{C}_{\text{Ref}}^{(\alpha\beta)}}$ ; thereby learning the label  $l$  that the emission corresponds to. Due to the equivalence between the Coin Protocol and the Virtual Protocol with tag assignment, we have that

$$\begin{aligned} N_{Z_C=0}^{\text{err}} &\equiv \sum_{\alpha=\beta} \left( N_{\text{vir}\alpha\beta, \text{TAR}\alpha\beta, Z_C}^{\text{det}} + \sum_{(i,j) \in \mathcal{C}_{\text{TAR}}^{(\alpha\beta)}} N_{ij, \text{TAR}\alpha\beta, Z_C}^{\text{det}} \right), \\ N_{Z_C=1}^{\text{err}} &\equiv \sum_{\alpha=\beta} \sum_{(i,j) \in \mathcal{C}_{\text{Ref}}^{(\alpha\beta)}} N_{ij, \text{REF}\alpha\beta, Z_C}^{\text{det}}, \\ N_{Z_C=0}^{\text{det}} &\equiv \sum_{\alpha, \beta} \left( N_{\text{vir}\alpha\beta, \text{TAR}\alpha\beta, Z_C}^{\text{det}} + \sum_{(i,j) \in \mathcal{C}_{\text{TAR}}^{(\alpha\beta)}} N_{ij, \text{TAR}\alpha\beta, Z_C}^{\text{det}} \right), \\ N_{Z_C=1}^{\text{det}} &\equiv \sum_{\alpha, \beta} \sum_{(i,j) \in \mathcal{C}_{\text{Ref}}^{(\alpha\beta)}} N_{ij, \text{REF}\alpha\beta, Z_C}^{\text{det}}, \end{aligned} \quad (\text{S144})$$

where  $N_{Z_C=z}^{\text{det}}$  is the number of detected rounds in which Alice and Bob obtained outcome  $z \in \{0, 1\}$  when measuring the coin system  $C$  in the  $Z_C$  basis, and  $N_{Z_C=z}^{\text{err}}$  is the number of these rounds in which the outcome of their measurement on systems  $D_a$  and  $D_b$  is such that  $\alpha = \beta$ . Substituting Eq. (S143) into Eq. (S144), we have that, in the asymptotic regime,

$$\begin{aligned} N_{Z_C=0}^{\text{err}} &\simeq p_{Z_C} \left( p_{\text{TAR}|\text{vir}} N_{\text{ph}} + \sum_{\alpha=\beta} \sum_{(i,j) \in \mathcal{C}_{\text{TAR}}^{(\alpha\beta)}} p_{\text{TAR}\alpha\beta|ij} N_{ij}^{\text{det}} \right), \\ N_{Z_C=1}^{\text{err}} &\simeq p_{Z_C} \left( \sum_{\alpha=\beta} \sum_{(i,j) \in \mathcal{C}_{\text{Ref}}^{(\alpha\beta)}} p_{\text{REF}\alpha\beta|ij} N_{ij}^{\text{det}} \right), \\ N_{Z_C=0}^{\text{det}} &\simeq p_{Z_C} \left( p_{\text{TAR}|\text{vir}} N_{\text{key}}^{\text{det}} + \sum_{\alpha, \beta} \sum_{(i,j) \in \mathcal{C}_{\text{TAR}}^{(\alpha\beta)}} p_{\text{TAR}\alpha\beta|ij} N_{ij}^{\text{det}} \right), \\ N_{Z_C=1}^{\text{det}} &\simeq p_{Z_C} \left( \sum_{\alpha, \beta} \sum_{(i,j) \in \mathcal{C}_{\text{Ref}}^{(\alpha\beta)}} p_{\text{REF}\alpha\beta|ij} N_{ij}^{\text{det}} \right). \end{aligned} \quad (\text{S145})$$

In Eq. (S145), we have used that  $p_{\text{TAR}|\text{vir}} := p_{\text{TAR00}|\text{vir00}} = p_{\text{TAR01}|\text{vir01}} = p_{\text{TAR10}|\text{vir10}} = p_{\text{TAR11}|\text{vir11}}$ ,  $N_{\text{ph}} := N_{\text{vir00}}^{\text{det}} + N_{\text{vir11}}^{\text{det}}$  and  $N_{\text{key}}^{\text{det}} = N_{\text{vir00}}^{\text{det}} + N_{\text{vir01}}^{\text{det}} + N_{\text{vir10}}^{\text{det}} + N_{\text{vir11}}^{\text{det}}$ , where  $N_{\text{key}}^{\text{det}}$  is the total number of detected key rounds, i.e., the size of the sifted key. Finally, substituting Eq. (S145) into the quantum coin inequality, Eq. (S43), and isolating  $N_{\text{ph}}$ , we obtain a bound on the number of phase errors in terms of the observables of the actual protocol.

#### D. General finite-key analysis for MDI protocols

Here, we extend the previous analysis to the finite-key regime, using the same approach as in Section SM1 E. As shown in Section SE1, in the finite-key regime, the Coin Protocol inequality becomes

$$N_{Z_C=0}^{\text{err}} - \Delta_A \leq_{6\epsilon_A} (N_{Z_C=0}^{\text{det}} + \Delta_A) G_+ \left( \frac{N_{Z_C=1}^{\text{err}} + \Delta_A}{N_{Z_C=1}^{\text{det}} - \Delta_A}, 1 - \frac{2p_{Z_C}(N_{X_C=1} + \Delta_A)}{p_{X_C}(N_{Z_C}^{\text{det}} - \Delta_A)} \right), \quad (\text{S146})$$

where we have employed Azuma's inequality using  $\Delta_A := \Delta_A(N_{\text{key}}^{\text{det}})$  with  $N_{\text{key}}^{\text{det}}$  denoting the total number of detected rounds. By substituting the definition of  $N_{Z_C=0}^{\text{err}}$  in Eq. (S144) into Eq. (S146) and rearranging, we obtain

$$N_{\text{ph},\text{TAR},Z_C} \leq_{6\epsilon_A} (N_{Z_C=0}^{\text{det}} + \Delta_A) G_+ \left( \frac{N_{Z_C=1}^{\text{err}} + \Delta_A}{N_{Z_C=1}^{\text{det}} - \Delta_A}, 1 - \frac{2p_{Z_C}(N_{X_C=1} + \Delta_A)}{p_{X_C}(N_{Z_C}^{\text{det}} - \Delta_A)} \right) + \Delta_A - \sum_{\alpha=\beta} \sum_{(i,j) \in \mathcal{C}_{\text{TAR}}^{(\alpha\beta)}} N_{ij,\text{TAR}\alpha\beta,Z_C}^{\text{det}}, \quad (\text{S147})$$

where we have defined  $N_{\text{ph},\text{TAR},Z_C} := \sum_{\alpha=\beta} N_{\text{vir}\alpha\beta,\text{TAR}\alpha\beta,Z_C}^{\text{det}}$ . Also, by the Chernoff bound, we have that

$$N_{X_C=1} \leq_{\epsilon_C} \hat{N}_{X_C=1} + \Delta_C^+(\hat{N}_{X_C=1}) =: \bar{N}_{X_C=1}, \quad (\text{S148})$$

where  $\hat{N}_{X_C=1} = N p_C p_{X_C} \Delta/2$ , and that

$$\begin{aligned} \underline{N}_{l,t,Z_C}^{\text{det}} &:= \hat{N}_{l,t,Z_C}^{\text{det}} - \Delta_C^-(\hat{N}_{l,t,Z_C}^{\text{det}}) \leq N_{l,t,Z_C}^{\text{det}} \leq \hat{N}_{l,t,Z_C}^{\text{det}} + \Delta_C^+(\hat{N}_{l,t,Z_C}^{\text{det}}) =: \bar{N}_{l,t,Z_C}^{\text{det}}, \\ \underline{N}_{\text{key},\text{TAR},Z_C}^{\text{det}} &:= \hat{N}_{\text{key},\text{TAR},Z_C}^{\text{det}} - \Delta_C^-(\hat{N}_{\text{key},\text{TAR},Z_C}^{\text{det}}) \leq N_{\text{key},\text{TAR},Z_C}^{\text{det}} \leq \hat{N}_{\text{key},\text{TAR},Z_C}^{\text{det}} + \Delta_C^+(\hat{N}_{\text{key},\text{TAR},Z_C}^{\text{det}}) =: \bar{N}_{\text{key},\text{TAR},Z_C}^{\text{det}}, \end{aligned} \quad (\text{S149})$$

where  $\hat{N}_{l,t,Z_C}^{\text{det}} = p_{Z_C} p_{t|l} N_l^{\text{det}}$ ,  $N_{\text{key},\text{TAR},Z_C}^{\text{det}} = \sum_{\alpha,\beta} N_{\text{vir}\alpha\beta,\text{TAR}\alpha\beta,Z_C}^{\text{det}}$  and  $\hat{N}_{\text{key},\text{TAR},Z_C}^{\text{det}} = p_{Z_C} p_{\text{TAR}|\text{vir}} N_{\text{key}}^{\text{det}}$ . Also, by Hoeffding's bound, we have that

$$N_{\text{ph},\text{TAR},Z_C} \geq_{\epsilon_H} p_{Z_C} p_{\text{TAR}|\text{vir}} N_{\text{ph}} - \Delta_H(N_{\text{ph}}) \geq p_{Z_C} p_{\text{TAR}|\text{vir}} N_{\text{ph}} - \Delta_H(N_{\text{key}}^{\text{det}}), \quad (\text{S150})$$

where in the last inequality we have upper bounded  $\Delta_H(N_{\text{ph}})$  by  $\Delta_H(N_{\text{key}}^{\text{det}})$ , where  $N_{\text{key}}^{\text{det}}$  is the number of detected key rounds. Substituting Eq. (S149) into Eq. (S144), we obtain

$$\begin{aligned} N_{Z_C=1}^{\text{err}} &\leq_{\# \epsilon_C} \bar{N}_{Z_C=1}^{\text{err}} := \sum_{\alpha=\beta} \sum_{(i,j) \in \mathcal{C}_{\text{Ref}}^{(\alpha\beta)}} \bar{N}_{ij,\text{REF}\alpha\beta,Z_C}^{\text{det}}, \\ N_{Z_C=0}^{\text{det}} &\leq_{\# \epsilon_C} \bar{N}_{Z_C=0}^{\text{det}} := \bar{N}_{\text{key},\text{TAR},Z_C}^{\text{det}} + \sum_{\alpha,\beta} \sum_{(i,j) \in \mathcal{C}_{\text{TAR}}^{(\alpha\beta)}} \bar{N}_{ij,\text{TAR}\alpha\beta,Z_C}^{\text{det}}, \\ N_{Z_C=0}^{\text{det}} &\geq_{\# \epsilon_C} \underline{N}_{Z_C=0}^{\text{det}} := \underline{N}_{\text{key},\text{TAR},Z_C}^{\text{det}} + \sum_{\alpha,\beta} \sum_{(i,j) \in \mathcal{C}_{\text{TAR}}^{(\alpha\beta)}} \underline{N}_{ij,\text{TAR}\alpha\beta,Z_C}^{\text{det}}, \\ N_{Z_C=1}^{\text{det}} &\geq_{\# \epsilon_C} \underline{N}_{Z_C=1}^{\text{det}} := \sum_{\alpha,\beta} \sum_{(i,j) \in \mathcal{C}_{\text{Ref}}^{(\alpha\beta)}} \underline{N}_{ij,\text{REF}\alpha\beta,Z_C}^{\text{det}}, \end{aligned} \quad (\text{S151})$$

where by, e.g.,  $\leq_{\# \epsilon_C}$ , we mean that the probability that the inequality fails is a factor times  $\epsilon_C$ , and for simplicity we will only calculate the total factor in the final formula. Substituting Eqs. (S148) to (S151) into Eq. (S147), we obtain an upper bound on the number of phase errors

$$\begin{aligned} N_{\text{ph}} &\leq_{\epsilon_{\text{tot}}} \frac{1}{p_{Z_C} p_{\text{TAR}|\text{vir}}} \left[ (\bar{N}_{Z_C=0}^{\text{det}} + \Delta_A) G_+ \left( \frac{\bar{N}_{Z_C=1}^{\text{err}} + \Delta_A}{\underline{N}_{Z_C=1}^{\text{det}} - \Delta_A}, 1 - \frac{2p_{Z_C}(\bar{N}_{X_C=1} + \Delta_A)}{p_{X_C}(\underline{N}_{Z_C=0}^{\text{det}} + \underline{N}_{Z_C=1}^{\text{det}} - \Delta_A)} \right) \right. \\ &\quad \left. - \sum_{\alpha=\beta} \sum_{(i,j) \in \mathcal{C}_{\text{TAR}}^{(\alpha\beta)}} \underline{N}_{ij,\text{TAR}\alpha\beta,Z_C}^{\text{det}} + \Delta_A + \Delta_H(N_{\text{key}}^{\text{det}}) \right] =: N_{\text{ph}}^{\text{U}}, \end{aligned} \quad (\text{S152})$$

where  $\epsilon_{\text{tot}} := 6\epsilon_A + (2(|\mathcal{C}_{\text{Tar}}^{(00)}| + |\mathcal{C}_{\text{Tar}}^{(01)}| + |\mathcal{C}_{\text{Tar}}^{(10)}| + |\mathcal{C}_{\text{Tar}}^{(11)}| + |\mathcal{C}_{\text{Ref}}^{(00)}| + |\mathcal{C}_{\text{Ref}}^{(01)}| + |\mathcal{C}_{\text{Ref}}^{(10)}| + |\mathcal{C}_{\text{Ref}}^{(11)}| + 3)\epsilon_C + \epsilon_H$  is the sum of the failure probabilities of all the concentration inequalities applied. After performing error correction, error verification and privacy amplification, Alice and Bob obtain an  $(\epsilon_{\text{corr}} + \epsilon_{\text{sec}})$ -secure key of length

$$N_{\text{sec}} = N_{\text{key}}^{\text{det}} [1 - h(e_{\text{ph}}^{\text{U}})] - \lambda_{\text{EC}} - \log_2 \frac{1}{\epsilon_{\text{corr}}} - \log_2 \frac{1}{\epsilon_{\text{PA}}}, \quad (\text{S153})$$

where  $e_{\text{ph}}^{\text{U}} := N_{\text{ph}}^{\text{U}}/N_{\text{key}}^{\text{det}}$  is the upper bound on the phase-error rate,  $\lambda_{\text{EC}} = fh(e_Z)$  is the cost of error correction, with  $f$  denoting the error correction efficiency and  $e_Z$  the observed bit-error rate,  $\epsilon_{\text{corr}}$  is the probability that the reconciled keys are not identical (due to the failure of error verification),  $\epsilon_{\text{PA}}$  is a free parameter that can be regarded as the failure probability of privacy amplification, and  $\epsilon_{\text{secr}} = \sqrt{2\epsilon_{\text{tot}} + \epsilon_{\text{PA}}}$ .

### SM3. SECURITY ANALYSIS FOR NON-IID SOURCES

For simplicity, in both the Main Text and Sections SM1 and SM2, we have implicitly assumed that the emitted states are pure, independent and identical across rounds. Here, we show how to apply our security analysis to scenarios in which this is not the case. For simplicity, we focus on the P&M scenario, although all results apply equally to MDI-type scenarios.

#### A. Independent but not identical pure states

As explained in Methods, our security proof can be applied without any modification when the emitted states are independent but different for different rounds, as long as Eq. (S1) holds for all rounds. That is, as long as the state emitted in the  $k$ -th round, which we can denote as  $|\psi_{j_k}^{(k)}\rangle_{B_k}$ , satisfies

$$|\langle \phi_{j_k} | \psi_{j_k}^{(k)} \rangle_{B_k}|^2 \geq 1 - \epsilon, \quad (\text{S154})$$

for all  $k$ , where  $\{|\phi_j\rangle\}_j$  are a set of known qubit states. Note that, in this case, the target and reference states  $|\Psi_{\text{Tar}}^{(k)}\rangle_{D_k A_k B_k}$  and  $|\Psi_{\text{Ref}}^{(k)}\rangle_{D_k A_k B_k}$ , and thus also the quantum coin state  $|\Psi_{\text{coin}}^{(k)}\rangle_{C_k D_k A_k B_k}$ , depend on the round  $k$ . However, this does not cause any problem in the security analysis presented in Section SM1 (and similarly for Section SM2), as the derivation of the coin protocol inequality in Section SE1 still holds, and the procedure in Section SE2 can still be used to obtain a bound on  $\text{Re} \langle \Psi_{\text{Ref}}^{(k)} | \Psi_{\text{Tar}}^{(k)} \rangle_{D_k A_k B_k}$  that holds for all  $k$ .

#### B. Independent but not identical mixed states

Also, as explained in Methods, our security proof can be applied without any modification when the emitted states  $\rho_j^{(k)}$  are mixed, as long as Eq. (1) of the Main Text is satisfied, i.e.,

$$\langle \phi_j | \rho_j^{(k)} | \phi_j \rangle_{B_k} \geq 1 - \epsilon. \quad (\text{S155})$$

This is because, by Uhlmann's theorem, there must exist a purification  $|\psi_j^{(k)}\rangle_{B_k S_k}$  of  $\rho_j^{(k)}$  such that

$$|\langle \phi_j | \psi_j^{(k)} \rangle_{B_k S_k}|^2 = \langle \phi_j | \rho_j^{(k)} | \phi_j \rangle_{B_k} \geq 1 - \epsilon, \quad (\text{S156})$$

where we have defined  $|\phi_j\rangle_{B_k S_k} := |\phi_j\rangle_{B_k} |0\rangle_{S_k}$ . This implies that our analysis can be applied to the mixed state case simply by substituting  $|\psi_j^{(k)}\rangle_{B_k} \rightarrow |\psi_j^{(k)}\rangle_{B_k S_k}$  and  $|\phi_j^{(k)}\rangle_{B_k} \rightarrow |\phi_j^{(k)}\rangle_{B_k S_k}$  in the scenario just described in Section SM3 A.

Moreover, we remark that our proof can be applied even if Eq. (S155) does not hold for *all* rounds of the protocol, as long as one can obtain a bound on the number of rounds for which it does not hold. In this scenario, one can apply the *tagging* idea introduced in [S35]; namely, one simply assumes that all rounds that violate Eq. (S155) are detected and *tagged* (i.e., its outcomes are assumed to be known to Eve), and then applies our security proof to the non-tagged rounds.

### C. Setting-independent pulse correlations

Our analysis is also directly applicable in a scenario that previous works have described as *setting-independent pulse correlations* [S36], i.e., when the emitted pulses are correlated but are independent of the setting choices made in previous rounds. Without loss of generality, in this case, we can consider that there exists a sequence of arbitrarily correlated random variables  $G_1 \dots G_N$  such that the states emitted in different rounds are independent given a particular sequence of outcomes  $g_1 \dots g_N$  of  $G_1 \dots G_N$ . That is, the global state emitted conditional on  $g_1 \dots g_N$  and a particular sequence of setting choices  $j_1 \dots j_N$  can be written as

$$\rho_{j_1}^{(g_1)} \otimes \dots \otimes \rho_{j_N}^{(g_N)}. \quad (\text{S157})$$

In this case, our security analysis is applicable as long as

$$\langle \phi_{j_k} | \rho_{j_k}^{(g_k)} | \phi_{j_k} \rangle_{B_k} \geq 1 - \epsilon, \quad (\text{S158})$$

for all  $k$ ,  $j_k$  and  $g_k$ . This is because, as shown in [S20], we can prove security by assuming a fictitious but mathematically equivalent scenario in which, in the very beginning of the protocol, Alice learns the sequence of outcomes  $g_1, \dots, g_N$  of  $G_1, \dots, G_N$ . Then, we have that, conditioned on a particular outcome  $g_1, \dots, g_N$ , the resulting scenario is equivalent to that discussed in Section SM3B above, which directly implies that we can use our analysis to obtain a bound of the form

$$\Pr[N_{\text{ph}}^{\text{U}} > N_{\text{ph}} | G_1 = g_1, \dots, G_N = g_N] \leq \epsilon_{\text{tot}}. \quad (\text{S159})$$

However, since this bound holds for any  $g_1, \dots, g_N$ , it follows that

$$\Pr[N_{\text{ph}}^{\text{U}} > N_{\text{ph}}] \leq \epsilon_{\text{tot}}, \quad (\text{S160})$$

which is what we need to guarantee security.

### D. Setting-dependent pulse correlations

With some modifications, our security proof can also be applied in the presence of setting-dependent pulse correlations, i.e., when the state emitted in a particular round depends also on the setting choices made in previous rounds. For this, it is useful to first examine the entangled state generated by Alice in the entanglement-based view of the protocol, for both the uncorrelated and correlated cases. In the former case, the state emitted in any round  $k$ , denoted as  $|\psi_{j_k}\rangle_{B_k}$ , depends solely on the  $k$ -th setting choice  $j_k$ , and Alice's state preparation is equivalent to the generation of the global entangled state

$$|\Psi_{\text{indep}}\rangle_{\mathbf{AB}} = \bigotimes_k \sum_{j_k} \sqrt{p_{j_k}} |j_k\rangle_{A_k} |\psi_{j_k}\rangle_{B_k}, \quad (\text{S161})$$

where  $\{|j_k\rangle_{A_k}\}_{j_k}$  forms an orthonormal basis for the ancillary system  $A_k$ ,  $\mathbf{A} := A_1 \dots A_N$  and  $\mathbf{B} := B_1 \dots B_N$ . Note that, in Eq. (S161), the state of systems  $A_k B_k$  and the state of systems  $A_{k'} B_{k'}$  is separable for all  $k \neq k'$ .

Now, let us consider correlated sources, starting with the simplest case: nearest-neighbor pulse correlations. In this scenario, the state emitted in the  $k$ -th round, denoted as  $|\psi_{j_k|j_{k-1}}\rangle_{B_k}$ , depends not only on the  $k$ -th setting choice  $j_k$  but also on the previous setting choice  $j_{k-1}$ . This situation is equivalent to Alice preparing the global entangled state<sup>5</sup>

$$|\Psi_{\text{correl}}\rangle_{\mathbf{AB}} = \sum_{j_1} \sqrt{p_{j_1}} |j_1\rangle_{A_1} |\psi_{j_1}\rangle_{B_1} \otimes \sum_{j_2} \sqrt{p_{j_2}} |j_2\rangle_{A_2} |\psi_{j_2|j_1}\rangle_{B_2} \otimes \dots \otimes \sum_{j_N} \sqrt{p_{j_N}} |j_N\rangle_{A_N} |\psi_{j_N|j_{N-1}}\rangle_{B_N}. \quad (\text{S162})$$

Importantly, the state of the systems  $A_k$  and  $B_{k+1}$  is now entangled, and thus  $|\Psi_{\text{correl}}\rangle_{\mathbf{AB}}$  lacks the separable structure of  $|\Psi_{\text{indep}}\rangle_{\mathbf{AB}}$  in Eq. (S161). At first glance, this presents an impediment to applying our security proof. However, we can overcome this problem by following the approach introduced in [S2, S20, S37, S38], which involves dividing the

<sup>5</sup> Note that, more generally, the emitted states may depend on the round  $k$ , and may be mixed rather than pure. However, as just shown in Sections SM3A to SM3C, this can be easily accommodated in our security proof, and for simplicity, we do not reflect this in the notation used here.

protocol rounds into even and odd subgroups, and separately proving the security of the key generated within each subgroup.

Say that we want to prove the security of the even subkey. To do so, we consider that Alice first measures all odd ancillas  $A_1 A_3 A_5 \dots$  in the computational basis, obtaining some measurement results  $j'_1, j'_3, j'_5, \dots$ , and the post-measurement state

$$|\Psi_{j'_1, j'_3, j'_5, \dots}\rangle_{AB} = |j'_1 j'_3 j'_5 \dots\rangle_{A_1 A_3 A_5 \dots} |\psi_{j'_1}\rangle_{B_1} \bigotimes_{k \text{ even}} \sum_{j_k} \sqrt{p_{j_k}} |j_k\rangle_{A_k} |\psi_{j_k | j'_{k-1}}\rangle_{B_k} |\psi_{j'_{k+1} | j_k}\rangle_{B_{k+1}}. \quad (\text{S163})$$

Our goal is to establish that a secure even subkey can be obtained from the entangled state in Eq. (S163) irrespectively of the sequence  $j'_1, j'_3, j'_5, \dots$ . This implies that the even subkey is also secure in the actual scenario independently of Alice's setting choices in the odd rounds.

Since we are considering the security of the even subkey, the state of systems  $A_1 A_3 A_5 \dots$  and  $B_1$  in Eq. (S163) is irrelevant and they can be traced out, resulting in the redefined state

$$|\Psi_{j'_1, j'_3, j'_5, \dots}\rangle_{AB} = \bigotimes_{k \text{ even}} \sum_{j_k} \sqrt{p_{j_k}} |j_k\rangle_{A_k} |\psi_{j_k | j'_{k-1}}\rangle_{B_k} |\psi_{j'_{k+1} | j_k}\rangle_{B_{k+1}}. \quad (\text{S164})$$

Note that Eq. (S164) has essentially the same structure as Eq. (S161), with the only differences being that in the former formula the tensor product is over even values of  $k$  only, and that the role played by  $|\psi_{j_k}\rangle_{B_k}$  in the latter formula is played by the combined state  $|\psi_{j_k | j'_{k-1}}\rangle_{B_k} |\psi_{j'_{k+1} | j_k}\rangle_{B_{k+1}}$  in the former. This takes into account the fact that, in the presence of nearest-neighbor pulse correlations, information about the  $k$ -th setting choice  $j_k$  is not only encoded into system  $B_k$  but also into system  $B_{k+1}$ . The equivalence between Eq. (S164) and Eq. (S161) directly implies that one can apply our analysis to prove the security of the even subkey by considering that the states emitted in the  $k$ -th round are  $\{|\psi_{j_k | j'_{k-1}}\rangle_{B_k} |\psi_{j'_{k+1} | j_k}\rangle_{B_{k+1}}\}_{j_k}$ . In particular, to apply our security proof, these states must satisfy

$$|\langle \phi_{j_k} | \psi_{j_k | j'_{k-1}}\rangle_{B_k} \langle \lambda_{j'_{k+1}} | \psi_{j'_{k+1} | j_k}\rangle_{B_{k+1}}|^2 \geq 1 - \epsilon, \quad (\text{S165})$$

for any setting choices  $j'_{k-1}, j_k, j'_{k+1}$ , where  $\{|\phi_{j_k}\rangle_{B_k}\}_{j_k}$  are known qubit states and  $|\lambda_{j'_{k+1}}\rangle_{B_{k+1}}$  is an arbitrary state on system  $B_{k+1}$  that is independent of  $j_k$ . This condition is the analogue to Eq. (S1) for the case of nearest-neighbor pulse correlations.

More generally, let us assume a maximum correlation length of  $l_c$  rounds and the knowledge that, for any setting choices  $j'_{k-l_c}, j'_{k-l_c+1}, \dots, j'_{k-1}, j_k, j'_{k+1}, \dots, j'_{k+l_c-1}, j'_{k+l_c}$ ,

$$|\langle \phi_{j_k} | \psi_{j_k | j'_{k-1}, j'_{k-2}, \dots, j'_{k-l_c}}\rangle_{B_k} \langle \lambda_{j'_{k-l_c+1}, \dots, j'_{k-1}, j'_{k+1}, \dots, j'_{k+l_c}} | \psi_{j'_{k-l_c+1}, \dots, j'_{k-1}, j_k, j'_{k+1}, \dots, j'_{k+l_c}}\rangle_{B_{k+1} B_{k+2} \dots B_{k+l_c}}|^2 \geq 1 - \epsilon, \quad (\text{S166})$$

where

$$|\psi_{j'_{k-l_c+1}, \dots, j'_{k-1}, j_k, j'_{k+1}, \dots, j'_{k+l_c}}\rangle_{B_{k+1} B_{k+2} \dots B_{k+l_c}} := |\psi_{j'_{k+1} | j_k, j'_{k-1}, \dots, j'_{k-l_c+1}}\rangle_{B_{k+1}} \dots |\psi_{j'_{k+l_c} | j'_{k+l_c-1}, j'_{k+l_c-2}, \dots, j_k}\rangle_{B_{k+l_c}}, \quad (\text{S167})$$

represents the state of systems  $B_{k+1} B_{k+2} \dots B_{k+l_c}$  for a given list of setting choices  $j'_{k-l_c+1}, \dots, j'_{k-1}, j_k, j'_{k+1}, \dots, j'_{k+l_c}$ , and  $|\lambda_{j'_{k-l_c+1}, \dots, j'_{k-1}, j'_{k+1}, \dots, j'_{k+l_c}}\rangle_{B_{k+1} B_{k+2} \dots B_{k+l_c}}$  denotes an arbitrary state on systems  $B_{k+1} B_{k+2} \dots B_{k+l_c}$  that is independent of  $j_k$ . Then, if these conditions are met, one can divide the protocol rounds into  $(l_c + 1)$  subgroups and apply our analysis to prove the security of the key extracted from each individual subgroup.

In practice, it may be useful to decompose the bound in Eq. (S166) into two, i.e.,

$$|\langle \phi_{j_k} | \psi_{j_k | j'_{k-1} j'_{k-2} \dots j'_{k-l_c}}\rangle_{B_k}|^2 \geq 1 - \epsilon_{\text{qubit}}, \quad (\text{S168})$$

and

$$|\langle \lambda_{j'_{k-l_c+1}, \dots, j'_{k-1}, j'_{k+1}, \dots, j'_{k+l_c}} | \psi_{j'_{k-l_c+1}, \dots, j'_{k-1}, j_k, j'_{k+1}, \dots, j'_{k+l_c}}\rangle_{B_{k+1} B_{k+2} \dots B_{k+l_c}}|^2 \geq 1 - \epsilon_{\text{correl}}, \quad (\text{S169})$$

with  $\epsilon = 1 - (1 - \epsilon_{\text{qubit}})(1 - \epsilon_{\text{correl}}) \leq \epsilon_{\text{qubit}} + \epsilon_{\text{correl}}$ . Similarly to Eq. (S1), the bound in Eq. (S168) evaluates how close the emitted state in each round is to a known qubit state, and should incorporate the effect of other side channels beyond pulse correlations. In contrast, the bound in Eq. (S169) depends only on the magnitude of the pulse correlations; in general, to evaluate it one needs knowledge on how this magnitude decreases as the pulse separation  $l \in \{1, \dots, l_c\}$  increases. For example, let us assume that we are able to obtain a bound on the maximum deviation

that the state emitted in a given round can undergo when varying the setting choice made  $l$  rounds ago, i.e., obtain a bound  $\epsilon_l$  such that, for  $j_{k-l} \neq \tilde{j}_{k-l}$

$$\left| \langle \psi_{j_k | j_{k-1}, \dots, j_{k-l+1}, \tilde{j}_{k-l}, j_{k-l-1}, \dots, j_{k-l_c}} | \psi_{j_k | j_{k-1}, \dots, j_{k-l+1}, j_{k-l}, j_{k-l-1}, \dots, j_{k-l_c}} \rangle_{B_k} \right|^2 \geq 1 - \epsilon_l. \quad (\text{S170})$$

Then, following a similar approach to that in the Methods Section of [S2], one can mathematically define a state  $|\lambda_{j'_{k-l_c+1}, \dots, j'_{k-1}, j'_{k+1}, \dots, j'_{k+l_c}}\rangle_{B_{k+1}B_{k+2}\dots B_{k+l_c}}$  that is independent of  $j_k$  by considering the state of systems  $B_{k+1}B_{k+2}\dots B_{k+l_c}$  when the  $k$ -th setting choice has been fixed to a particular value  $j_k = \gamma$ , i.e.,

$$\begin{aligned} |\lambda_{j'_{k-l_c+1}, \dots, j'_{k-1}, j'_{k+1}, \dots, j'_{k+l_c}}\rangle_{B_{k+1}B_{k+2}\dots B_{k+l_c}} &:= |\psi_{j'_{k-l_c+1}, \dots, j'_{k-1}, \gamma, j'_{k+1}, \dots, j'_{k+l_c}}\rangle_{B_{k+1}B_{k+2}\dots B_{k+l_c}} \\ &= |\psi_{j'_{k+1} | \gamma, j'_{k-1}, \dots, j'_{k-l_c+1}}\rangle_{B_{k+1}} \dots |\psi_{j'_{k+l_c} | j'_{k+l_c-1}, j'_{k+l_c-2}, \dots, \gamma}\rangle_{B_{k+l_c}}, \end{aligned} \quad (\text{S171})$$

and it immediately follows that

$$\epsilon_{\text{correl}} = 1 - \prod_{l=1}^{l_c} (1 - \epsilon_l) \leq \sum_{l=1}^{l_c} \epsilon_l. \quad (\text{S172})$$

Note that the above analysis implicitly assumes that the correlations have a finite maximum correlation length  $l_c$ , i.e., that there is a certain  $l$  such that the setting choice made in the  $k$ -th round has absolutely no influence on the signal emitted in the  $(k+l)$ -th round for  $l > l_c$ . In practice, while it seems reasonable to assume that the correlation magnitude  $\epsilon_l$  should decrease rapidly with the length  $l$ , the expectation that this magnitude will drop to exactly zero for any finite value of  $l$  may not be justified. Nevertheless, as recently shown in [S39], security proofs such as ours can still be rigorously applied even if the length of the correlations is unbounded, using the following approach: (1) consider an effective maximum correlation length  $l_e$ , which should be such that the combined magnitude of the correlations between pulses separated by more than  $l_e$  rounds is extremely small; (2) apply our security proof assuming that the true correlation length  $l_c$  equals  $l_e$ ; and (3) rigorously account for the neglected long-range correlations by slightly increasing the security parameter of the final key  $\epsilon_{\text{sec}}$  by an amount that can be made as small as desired by increasing  $l_e$ .

We emphasize that, in this section, we have focused on *classical* pulse correlations, i.e., the scenario in which the classical setting choices made in a particular round influence the quantum states emitted in subsequent rounds. This effect is well-documented and widely recognized as a significant threat to the security of QKD systems, particularly those run at high speeds [S40]. Theoretically, another type of correlations, referred to as *quantum* correlations, could also be considered. These would occur if the photonic systems emitted in different rounds were entangled. However, entanglement is an extremely fragile resource that is challenging to generate even intentionally. Therefore, it is extremely unlikely that practical QKD sources emit pulses that are entangled across rounds. Even if such entanglement occurred, one expects that its magnitude would be minimal, providing a negligible advantage to an eavesdropper. In this context, we remark that our security proof could incorporate these quantum correlations by applying the results of [S39] in a similar way as described in the previous paragraph for residual long-range correlations: (1) obtain a bound on the trace distance  $d$  between the actual global state emitted by the source, which contains a minimal amount of quantum correlations, and the global state that would be emitted if these correlations did not exist; (2) apply our security proof assuming that these quantum correlations do not exist; and (3) increment the security parameter of the final key by  $2d$ .

#### SM4. SECURITY WITH WCP LIGHT SOURCES

In this Section, we discuss how our security proof can be applied to scenarios in which the light source emits weak coherent pulses (WCPs) rather than single photons. First, in Section SM4 A, we show how to directly apply our analysis to a coherent-light-based MDI protocol [S34] that does not require either intensity modulation or phase randomization, and thus avoids the security loopholes introduced by imperfections in these processes, achieving a very high degree of implementation security in a straightforward manner. Then, in Section SM4 B, we show how our analysis can be combined with the decoy-state method [S41–S43] to guarantee security in the more common scenario in which the light source is an intensity-modulated phase-randomized WCP source, and discuss how our techniques can be applied to take into account imperfections in both the intensity modulation and phase randomization processes.

### A. Coherent-light-based MDI protocol

Here, we apply our general security proof for MDI-type protocols, presented in Section SM2, to prove the security of the coherent-light-based MDI scheme proposed in [S34]. By doing so, we introduce two important improvements with respect to its existing security proof in [S34]: (1) the proof in [S34] is based on the reference technique (RT) [S2], and therefore requires a sequential assumption that may be especially difficult to guarantee for MDI-type protocols (see Section SM5 for more information); and (2) our security proof achieves significantly higher secret-key rates than that of [S34], even in terms of bits per pulse.

#### 1. Protocol description

In this scheme, Alice (Bob) tries to prepare the states  $\{|\sqrt{\mu}\rangle_{B_a(B_b)}, |-\sqrt{\mu}\rangle_{B_a(B_b)}, |\text{vac}\rangle_{B_a(B_b)}\}$ , where  $|\sqrt{\mu}\rangle_{B_a(B_b)}$  and  $|-\sqrt{\mu}\rangle_{B_a(B_b)}$  are coherent states of intensity  $\mu$  and opposite phases associated with bit values 0 and 1, respectively, and  $|\text{vac}\rangle_{B_a(B_b)}$  is a vacuum state that is used for parameter estimation. However, we assume that, due to various imperfections and side channels, the states that she (he) actually prepares,  $\{|\psi_{0Z}\rangle_{B_a(B_b)}, |\psi_{1Z}\rangle_{B_a(B_b)}, |\psi_{0X}\rangle_{B_a(B_b)}\}$ , are only  $\epsilon$ -close to these, i.e., they satisfy

$$\begin{aligned} |\langle\sqrt{\mu}|\psi_{0Z}\rangle_{B_u}|^2 &\geq 1 - \epsilon, \\ |\langle-\sqrt{\mu}|\psi_{1Z}\rangle_{B_u}|^2 &\geq 1 - \epsilon, \\ |\langle\text{vac}|\psi_{0X}\rangle_{B_u}|^2 &\geq 1 - \epsilon, \end{aligned} \quad (\text{S173})$$

where  $u \in \{a, b\}$ . The setup for this scheme is depicted in Fig. S6, and the full protocol is described below.

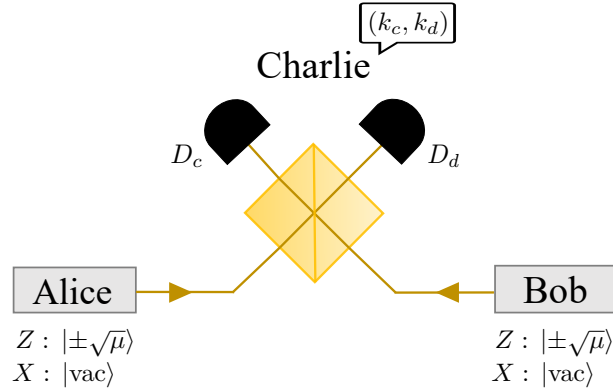

Figure S6. Illustration of the coherent-light-based MDI setup [S34]. In every round, Alice and Bob attempt to prepare a state in the set  $\{|\sqrt{\mu}\rangle, |-\sqrt{\mu}\rangle, |\text{vac}\rangle\}$  and send it to the middle node Charlie through a quantum channel. Charlie measures the incoming signals by interfering them with a 50:50 beamsplitter, followed by two threshold detectors  $D_c$  and  $D_d$ , which are associated with constructive and destructive interference, respectively; and announces the outcome  $(k_c, k_d)$ , where  $k_c = 1$  ( $k_d = 1$ ) if detector  $D_c$  ( $D_d$ ) clicks, and  $k_c = 0$  ( $k_d = 0$ ) otherwise.

---

### Coherent-light-based MDI protocol

1. **Quantum communication:** For each of the  $N$  rounds: (a) Alice (Bob) chooses a state from the set  $\{|\psi_{0Z}\rangle_{B_a(B_b)}, |\psi_{1Z}\rangle_{B_a(B_b)}, |\psi_{0X}\rangle_{B_a(B_b)}\}$  with probabilities  $\{p_Z/2, p_Z/2, p_X\}$ , where  $p_X := 1 - p_Z$ , and sends it to the middle node Charlie through a quantum channel. (b) If Charlie is honest (he could be completely dishonest and under Eve's control), he measures Alice and Bob's signals by interfering them at a 50:50 beamsplitter, followed by threshold detectors  $D_c$  and  $D_d$  placed at the output ports corresponding to constructive and destructive interference, respectively. After the measurement, Charlie reports the pair  $(k_c, k_d)$ , where  $k_c = 1$  ( $k_d = 1$ ) if detector  $D_c$  ( $D_d$ ) clicks and  $k_c = 0$  ( $k_d = 0$ ) otherwise. A round is considered detected (undetected) if  $k_c \neq k_d$  ( $k_c = k_d$ ).
2. **Basis and bit announcement:** For each detected round, Alice (Bob) announces the  $Z$  basis if her (his) setting choice was  $j \in \{0_Z, 1_Z\}$ , or the  $X$  basis otherwise. Then, for each detected round in which both users

announced the  $Z$  basis, Alice assigns the round to “key” (“test”) with probability  $p_{\text{key}|Z}$  ( $p_{\text{test}|Z} = 1 - p_{\text{key}|Z}$ ), and announces this information. All the other detected rounds are assigned to “test”. Then, the users announce their setting choices for the rounds assigned to “test”, and define their sifted keys as the bit outcomes of the rounds assigned to “key”. For the key rounds in which  $k_c = 0$  and  $k_d = 1$ , Bob flips his sifted key bit<sup>6</sup>.

3. **Parameter estimation:** The users quantify the number of events  $N_{ij}^{\text{det}}$  in which Alice’s (Bob’s) setting choice was  $i$  ( $j$ ), Charlie announced a detection, and the round was assigned to “test”; the number of detected key events  $N_{\text{key}}^{\text{det}}$  (i.e., the length of the sifted key); and the total number of detected rounds  $N^{\text{det}} := N_{\text{key}}^{\text{det}} + \sum_{i,j} N_{ij}^{\text{det}}$ . Then, they use this information to obtain an upper bound on the phase-error rate  $e_{\text{ph}}$  of the sifted key.
4. **Data post-processing:** Alice sends Bob syndrome information about her sifted key through an authenticated classical channel for him to correct his own sifted key. After, Alice and Bob perform error verification by computing a hash of their corrected keys using a random two-universal hash function and then check whether they are identical. If so, Alice and Bob perform privacy amplification by employing a random two-universal hash function to extract a secure key pair from the corrected keys. Otherwise, they abort the protocol.

## 2. Security analysis

To apply our security analysis, we need to select some qubit states  $\{|\phi_{0Z}\rangle_{B_u}, |\phi_{1Z}\rangle_{B_u}, |\phi_{0X}\rangle_{B_u}\}$  that are close to the actual states  $\{|\psi_{0Z}\rangle_{B_u}, |\psi_{1Z}\rangle_{B_u}, |\psi_{0X}\rangle_{B_u}\}$ . As in Ref. [S34], we select the first two to be

$$\begin{aligned} |\phi_{0Z}\rangle_{B_u} &= |\sqrt{\mu}\rangle_{B_u}, \\ |\phi_{1Z}\rangle_{B_u} &= |-\sqrt{\mu}\rangle_{B_u}, \end{aligned} \quad (\text{S174})$$

and for the third,  $|\phi_{0X}\rangle_{B_u}$ , we pick the projection of  $|\text{vac}\rangle_{B_u}$  onto the subspace spanned by  $\{|\sqrt{\mu}\rangle_{B_u}, |-\sqrt{\mu}\rangle_{B_u}\}$ .

Now let us define

$$|\Phi_Z\rangle_{A_u B_u} = \frac{1}{\sqrt{2}}(|0_Z\rangle_{A_u} |\phi_{0Z}\rangle_{B_u} + |1_Z\rangle_{A_u} |\phi_{1Z}\rangle_{B_u}) = \sqrt{q_{\text{vir}0}^\phi} |0_X\rangle_{A_u} |\phi_{\text{vir}0}\rangle_{B_u} + \sqrt{q_{\text{vir}1}^\phi} |1_X\rangle_{A_u} |\phi_{\text{vir}1}\rangle_{B_u}, \quad (\text{S175})$$

where

$$\begin{aligned} |\phi_{\text{vir}0}\rangle_{B_u} &= \frac{1}{2\sqrt{q_{\text{vir}0}^\phi}}(|\phi_{0Z}\rangle_{B_u} + |\phi_{1Z}\rangle_{B_u}), \\ |\phi_{\text{vir}1}\rangle_{B_u} &= \frac{1}{2\sqrt{q_{\text{vir}1}^\phi}}(|\phi_{0Z}\rangle_{B_u} - |\phi_{1Z}\rangle_{B_u}), \end{aligned} \quad (\text{S176})$$

and

$$\begin{aligned} q_{\text{vir}0}^\phi &= \frac{1 + e^{-2\mu}}{2}, \\ q_{\text{vir}1}^\phi &= \frac{1 - e^{-2\mu}}{2}. \end{aligned} \quad (\text{S177})$$

It is straightforward to show that  $|\phi_{\text{vir}0}\rangle_{B_u} = |C_{\text{even}}\rangle_{B_u}$  and  $|\phi_{\text{vir}1}\rangle_{B_u} = |C_{\text{odd}}\rangle_{B_u}$ , where  $|C_{\text{even}}\rangle_{B_u}$  and  $|C_{\text{odd}}\rangle_{B_u}$  are even and odd cat states, respectively, given by

$$|C_{\text{even}}\rangle_{B_u} \propto |\sqrt{\mu}\rangle_{B_u} + |-\sqrt{\mu}\rangle_{B_u}, \quad |C_{\text{odd}}\rangle_{B_u} \propto |\sqrt{\mu}\rangle_{B_u} - |-\sqrt{\mu}\rangle_{B_u}. \quad (\text{S178})$$

Since  $\{|\phi_{0Z}\rangle_{B_u}, |\phi_{1Z}\rangle_{B_u}, |\phi_{0X}\rangle_{B_u}\}$  is a set of three qubit states, we can obtain unique LT expressions for them (see Section SM1 D for more information), and in this case these can be calculated to be

$$\begin{aligned} |\phi_{\text{vir}0}\rangle_{B_u} \langle \phi_{\text{vir}0}|_{B_u} &= |\phi_{0X}\rangle_{B_u} \langle \phi_{0X}|_{B_u}, \\ |\phi_{\text{vir}1}\rangle_{B_u} \langle \phi_{\text{vir}1}|_{B_u} &= c_1 |\phi_{0Z}\rangle_{B_u} \langle \phi_{0Z}|_{B_u} + c_1 |\phi_{1Z}\rangle_{B_u} \langle \phi_{1Z}|_{B_u} - c_2 |\phi_{0X}\rangle_{B_u} \langle \phi_{0X}|_{B_u}, \end{aligned} \quad (\text{S179})$$

<sup>6</sup> This conditional bit flip is performed in the Actual Protocol to ensure that the bit-error rate of the sifted key is kept low. However, when considering the security of the sifted key this bit flip is irrelevant, and in the security proof, we only consider whether a round has been reported as detected ( $k_c \neq k_d$ ) or undetected ( $k_c = k_d$ ).

where

$$\begin{aligned} c_1 &= \frac{1 + \coth(\mu)}{2} = \frac{e^{2\mu}}{e^{2\mu} - 1} \geq 0, \\ c_2 &= \coth(\mu) = \frac{e^{2\mu} + 1}{e^{2\mu} - 1} \geq 1. \end{aligned} \quad (\text{S180})$$

Taking the tensor products of the expressions in Eq. (S179), and passing all negative terms to the left-hand side, we obtain the following MDI loss-tolerant expressions

$$\begin{aligned} |\phi_{\text{vir}00}\rangle\langle\phi_{\text{vir}00}|_{B_a B_b} &= |\phi_{0_X 0_X}\rangle\langle\phi_{0_X 0_X}|_{B_a B_b}, \\ |\phi_{\text{vir}01}\rangle\langle\phi_{\text{vir}01}|_{B_a B_b} &+ c_2 |\phi_{0_X 0_X}\rangle\langle\phi_{0_X 0_X}|_{B_a B_b} = c_1 |\phi_{0_X 0_Z}\rangle\langle\phi_{0_X 0_Z}|_{B_a B_b} + c_1 |\phi_{0_X 1_Z}\rangle\langle\phi_{0_X 1_Z}|_{B_a B_b}, \\ |\phi_{\text{vir}10}\rangle\langle\phi_{\text{vir}10}|_{B_a B_b} &+ c_2 |\phi_{0_X 0_X}\rangle\langle\phi_{0_X 0_X}|_{B_a B_b} = c_1 |\phi_{0_Z 0_X}\rangle\langle\phi_{0_Z 0_X}|_{B_a B_b} + c_1 |\phi_{1_Z 0_X}\rangle\langle\phi_{1_Z 0_X}|_{B_a B_b}, \\ |\phi_{\text{vir}11}\rangle\langle\phi_{\text{vir}11}|_{B_a B_b} &+ c_1 c_2 |\phi_{0_Z 0_X}\rangle\langle\phi_{0_Z 0_X}|_{B_a B_b} + c_1 c_2 |\phi_{1_Z 0_X}\rangle\langle\phi_{1_Z 0_X}|_{B_a B_b} + c_1 c_2 |\phi_{0_X 0_Z}\rangle\langle\phi_{0_X 0_Z}|_{B_a B_b} \\ &+ c_1 c_2 |\phi_{0_X 1_Z}\rangle\langle\phi_{0_X 1_Z}|_{B_a B_b} = c_1^2 |\phi_{0_Z 0_Z}\rangle\langle\phi_{0_Z 0_Z}|_{B_a B_b} + c_1^2 |\phi_{0_Z 1_Z}\rangle\langle\phi_{0_Z 1_Z}|_{B_a B_b} + c_1^2 |\phi_{1_Z 0_Z}\rangle\langle\phi_{1_Z 0_Z}|_{B_a B_b} \\ &+ c_1^2 |\phi_{1_Z 1_Z}\rangle\langle\phi_{1_Z 1_Z}|_{B_a B_b} + c_2^2 |\phi_{0_X 0_X}\rangle\langle\phi_{0_X 0_X}|_{B_a B_b}. \end{aligned} \quad (\text{S181})$$

Then, we construct some states  $|\Phi_{\text{Tar}\alpha\beta}\rangle_{AB}$  and  $|\Phi_{\text{Ref}\alpha\beta}\rangle_{AB}$ , with  $B := B_a B_b$ , by taking purifications of the left- and right-hand sides of Eq. (S181). We choose purifications such that  $|\Phi_{\text{Tar}\alpha\beta}\rangle_{AB} = |\Phi_{\text{Ref}\alpha\beta}\rangle_{AB}$ , which exist due to the equalities in Eq. (S181), and can be shown to be

$$\begin{aligned} |\Phi_{\text{Tar}00}\rangle_{AB} &= |0\rangle_A |\phi_{\text{vir}00}\rangle_{B_a B_b}, \\ |\Phi_{\text{Ref}00}\rangle_{AB} &= |0\rangle_A |\phi_{0_X 0_X}\rangle_{B_a B_b}, \\ |\Phi_{\text{Tar}01}\rangle_{AB} &\propto |0\rangle_A |\phi_{\text{vir}01}\rangle_{B_a B_b} + \sqrt{c_2} |1\rangle_A |\phi_{0_X 0_X}\rangle_{B_a B_b}, \\ |\Phi_{\text{Ref}01}\rangle_{AB} &\propto \sqrt{c_1} |0'\rangle_A |\phi_{0_X 0_Z}\rangle_{B_a B_b} + \sqrt{c_1} |1'\rangle_A |\phi_{0_X 1_Z}\rangle_{B_a B_b}, \\ |\Phi_{\text{Tar}10}\rangle_{AB} &\propto |0\rangle_A |\phi_{\text{vir}10}\rangle_{B_a B_b} + \sqrt{c_2} |1\rangle_A |\phi_{0_X 0_X}\rangle_{B_a B_b}, \\ |\Phi_{\text{Ref}10}\rangle_{AB} &\propto \sqrt{c_1} |0'\rangle_A |\phi_{0_Z 0_X}\rangle_{B_a B_b} + \sqrt{c_1} |1'\rangle_A |\phi_{1_Z 0_X}\rangle_{B_a B_b}, \\ |\Phi_{\text{Tar}11}\rangle_{AB} &\propto |0\rangle_A |\phi_{\text{vir}11}\rangle_{B_a B_b} + \sqrt{c_1 c_2} |1\rangle_A |\phi_{0_Z 0_X}\rangle_{B_a B_b} + \sqrt{c_1 c_2} |2\rangle_A |\phi_{1_Z 0_X}\rangle_{B_a B_b} + \sqrt{c_1 c_2} |3\rangle_A |\phi_{0_X 0_Z}\rangle_{B_a B_b} \\ &+ \sqrt{c_1 c_2} |4\rangle_A |\phi_{0_X 1_Z}\rangle_{B_a B_b}, \\ |\Phi_{\text{Ref}11}\rangle_{AB} &\propto c_1 |0''\rangle_A |\phi_{0_Z 0_Z}\rangle_{B_a B_b} + c_1 |1''\rangle_A |\phi_{0_Z 1_Z}\rangle_{B_a B_b} + c_1 |2''\rangle_A |\phi_{1_Z 0_Z}\rangle_{B_a B_b} + c_1 |3''\rangle_A |\phi_{1_Z 1_Z}\rangle_{B_a B_b} \\ &+ c_2 |4''\rangle_A |\phi_{0_X 0_X}\rangle_{B_a B_b}, \end{aligned} \quad (\text{S182})$$

where

$$\begin{aligned} |0'\rangle_A &= \frac{1}{\sqrt{2}}(|0\rangle_A + |1\rangle_A), \\ |1'\rangle_A &= \frac{1}{\sqrt{2}}(-|0\rangle_A + |1\rangle_A), \end{aligned} \quad (\text{S183})$$

and

$$\begin{aligned} |0''\rangle_A &= \frac{1}{2} |0\rangle_A + \frac{1}{2\sqrt{2}} |1\rangle_A - \frac{1}{2\sqrt{2}} |2\rangle_A + \frac{1}{\sqrt{2}} |3\rangle_A, \\ |1''\rangle_A &= -\frac{1}{2} |0\rangle_A + \frac{1}{2\sqrt{2}} |1\rangle_A - \frac{1}{2\sqrt{2}} |2\rangle_A + \frac{1}{\sqrt{2}} |4\rangle_A, \\ |2''\rangle_A &= -\frac{1}{2} |0\rangle_A - \frac{1}{2\sqrt{2}} |1\rangle_A + \frac{1}{2\sqrt{2}} |2\rangle_A + \frac{1}{\sqrt{2}} |3\rangle_A, \\ |3''\rangle_A &= \frac{1}{2} |0\rangle_A - \frac{1}{2\sqrt{2}} |1\rangle_A + \frac{1}{2\sqrt{2}} |2\rangle_A + \frac{1}{\sqrt{2}} |4\rangle_A, \\ |4''\rangle_A &= \frac{1}{\sqrt{2}} |1\rangle_A + \frac{1}{\sqrt{2}} |2\rangle_A. \end{aligned} \quad (\text{S184})$$

To obtain Eq. (S184), for example, we first define the following state with real coefficients

$$|m''\rangle_A = d_0^{(m)} |0\rangle_A + d_1^{(m)} |1\rangle_A + d_2^{(m)} |2\rangle_A + d_3^{(m)} |3\rangle_A + d_4^{(m)} |4\rangle_A, \quad (\text{S185})$$

such that  $(d_0^{(m)})^2 + (d_1^{(m)})^2 + (d_2^{(m)})^2 + (d_3^{(m)})^2 + (d_4^{(m)})^2 = 1$  for all  $m \in \{0, 1, 2, 3, 4\}$ , and substitute Eq. (S185) and the definition of  $|\phi_{\text{vir}11}\rangle_{B_a B_b} := |\phi_{\text{vir}1}\rangle_{B_a} \otimes |\phi_{\text{vir}1}\rangle_{B_b}$  in Eq. (S176) into Eq. (S182). Then, we use the condition  $|\Phi_{\text{Tar}11}\rangle_{AB} = |\Phi_{\text{Ref}11}\rangle_{AB}$  to construct a system of equations for the variables  $\{d_0^{(m)}, d_1^{(m)}, d_2^{(m)}, d_3^{(m)}, d_4^{(m)}\}_{m=0}^4$ , and solve this system.

Using Eq. (S182) as a blueprint, we define the states  $|\Psi_{\text{Tar}\alpha\beta}\rangle_{AB}$  and  $|\Psi_{\text{Ref}\alpha\beta}\rangle_{AB}$  as

$$\begin{aligned}
|\Psi_{\text{Tar}00}\rangle_{AB} &= \sqrt{p_{\text{vir}00}|\text{TAR}00|} |0\rangle_A |\psi_{\text{vir}00}\rangle_{B_a B_b}, \\
|\Psi_{\text{Ref}00}\rangle_{AB} &= \sqrt{p_{0_X 0_X}|\text{REF}00|} |0\rangle_A |\psi_{0_X 0_X}\rangle_{B_a B_b}, \\
|\Psi_{\text{Tar}01}\rangle_{AB} &= \sqrt{p_{\text{vir}01}|\text{TAR}01|} |0\rangle_A |\psi_{\text{vir}01}\rangle_{B_a B_b} + \sqrt{p_{0_X 0_X}|\text{TAR}01|} |1\rangle_A |\psi_{0_X 0_X}\rangle_{B_a B_b}, \\
|\Psi_{\text{Ref}01}\rangle_{AB} &= \sqrt{p_{0_X 0_Z}|\text{REF}01|} |0'\rangle_A |\psi_{0_X 0_Z}\rangle_{B_a B_b} + \sqrt{p_{0_X 1_Z}|\text{REF}01|} |1'\rangle_A |\psi_{0_X 1_Z}\rangle_{B_a B_b}, \\
|\Psi_{\text{Tar}10}\rangle_{AB} &= \sqrt{p_{\text{vir}10}|\text{TAR}10|} |0\rangle_A |\psi_{\text{vir}10}\rangle_{B_a B_b} + \sqrt{p_{0_X 0_X}|\text{TAR}10|} |1\rangle_A |\psi_{0_X 0_X}\rangle_{B_a B_b}, \\
|\Psi_{\text{Ref}10}\rangle_{AB} &= \sqrt{p_{0_Z 0_X}|\text{REF}10|} |0'\rangle_A |\psi_{0_Z 0_X}\rangle_{B_a B_b} + \sqrt{p_{1_Z 0_X}|\text{REF}10|} |1'\rangle_A |\psi_{1_Z 0_X}\rangle_{B_a B_b}, \\
|\Psi_{\text{Tar}11}\rangle_{AB} &= \sqrt{p_{\text{vir}11}|\text{TAR}11|} |0\rangle_A |\psi_{\text{vir}11}\rangle_{B_a B_b} + \sqrt{p_{0_Z 0_X}|\text{TAR}11|} |1\rangle_A |\psi_{0_Z 0_X}\rangle_{B_a B_b} + \sqrt{p_{1_Z 0_X}|\text{TAR}11|} |2\rangle_A |\psi_{1_Z 0_X}\rangle_{B_a B_b} \\
&\quad + \sqrt{p_{0_X 0_Z}|\text{TAR}11|} |3\rangle_A |\psi_{0_X 0_Z}\rangle_{B_a B_b} + \sqrt{p_{0_X 1_Z}|\text{TAR}11|} |4\rangle_A |\psi_{0_X 1_Z}\rangle_{B_a B_b}, \\
|\Psi_{\text{Ref}11}\rangle_{AB} &= \sqrt{p_{0_Z 0_Z}|\text{REF}11|} |0''\rangle_A |\psi_{0_Z 0_Z}\rangle_{B_a B_b} + \sqrt{p_{0_Z 1_Z}|\text{REF}11|} |1''\rangle_A |\psi_{0_Z 1_Z}\rangle_{B_a B_b} + \sqrt{p_{1_Z 0_Z}|\text{REF}11|} |2''\rangle_A |\psi_{1_Z 0_Z}\rangle_{B_a B_b} \\
&\quad + \sqrt{p_{1_Z 1_Z}|\text{REF}11|} |3''\rangle_A |\psi_{1_Z 1_Z}\rangle_{B_a B_b} + \sqrt{p_{0_X 0_X}|\text{REF}11|} |4''\rangle_A |\psi_{0_X 0_X}\rangle_{B_a B_b},
\end{aligned} \tag{S186}$$

where

$$\begin{aligned}
p_{\text{vir}00}|\text{TAR}00| &= p_{0_X 0_X}|\text{REF}00| = 1, \\
p_{\text{vir}01}|\text{TAR}01| &= \frac{q_{\text{vir}01}^\psi}{q_{\text{vir}01}^\psi + c_2 q_{\text{vir}01}^\phi}, \\
p_{0_X 0_X}|\text{TAR}01| &= \frac{c_2 q_{\text{vir}01}^\phi}{q_{\text{vir}01}^\psi + c_2 q_{\text{vir}01}^\phi}, \\
p_{0_X 0_Z}|\text{REF}01| &= p_{0_X 1_Z}|\text{REF}01| = p_{0_Z 0_X}|\text{REF}10| = p_{1_Z 0_X}|\text{REF}10| = \frac{c_1}{2c_1} = \frac{1}{2}, \\
p_{\text{vir}10}|\text{TAR}10| &= \frac{q_{\text{vir}10}^\psi}{q_{\text{vir}10}^\psi + c_2 q_{\text{vir}10}^\phi}, \\
p_{0_X 0_X}|\text{TAR}10| &= \frac{c_2 q_{\text{vir}10}^\phi}{q_{\text{vir}10}^\psi + c_2 q_{\text{vir}10}^\phi}, \\
p_{\text{vir}11}|\text{TAR}11| &= \frac{q_{\text{vir}11}^\psi}{q_{\text{vir}11}^\psi + 4c_1 c_2 q_{\text{vir}11}^\phi}, \\
p_{0_Z 0_X}|\text{TAR}11| &= p_{1_Z 0_X}|\text{TAR}11| = p_{0_X 0_Z}|\text{TAR}11| = p_{0_X 1_Z}|\text{TAR}11| = \frac{c_1 c_2 q_{\text{vir}11}^\phi}{q_{\text{vir}11}^\psi + 4c_1 c_2 q_{\text{vir}11}^\phi}, \\
p_{0_Z 0_Z}|\text{REF}11| &= p_{1_Z 0_Z}|\text{REF}11| = p_{0_Z 1_Z}|\text{REF}11| = p_{1_Z 1_Z}|\text{REF}11| = \frac{c_1^2}{4c_1^2 + c_2^2}, \\
p_{0_X 0_X}|\text{REF}11| &= \frac{c_2^2}{4c_1^2 + c_2^2}.
\end{aligned} \tag{S187}$$

Then, we define  $|\Psi_{\text{Tar}}\rangle_{DAB}$  and  $|\Psi_{\text{Ref}}\rangle_{DAB}$ , with  $D := D_a D_b$ , as

$$|\Psi_{\text{Tar}}\rangle_{DAB} = \sum_{\alpha, \beta} \sqrt{p_{\text{TAR}\alpha\beta}|\text{TAR}|} |\alpha\beta\rangle_{D_a D_b} |\Psi_{\text{Tar}\alpha\beta}\rangle_{AB}, \tag{S188}$$

$$|\Psi_{\text{Ref}}\rangle_{DAB} = \sum_{\alpha, \beta} \sqrt{p_{\text{REF}\alpha\beta}|\text{REF}|} |\alpha\beta\rangle_{D_a D_b} |\Psi_{\text{Ref}\alpha\beta}\rangle_{AB}, \tag{S189}$$

where

$$\begin{aligned}
p_{\text{TAR}00|\text{TAR}} &= \frac{q_{\text{vir}00}^\psi}{C}, \\
p_{\text{REF}00|\text{REF}} &= \frac{q_{\text{vir}00}^\phi}{C}, \\
p_{\text{TAR}01|\text{TAR}} &= \frac{q_{\text{vir}01}^\psi + c_2 q_{\text{vir}01}^\phi}{C}, \\
p_{\text{REF}01|\text{REF}} &= \frac{2c_1 q_{\text{vir}01}^\phi}{C}, \\
p_{\text{TAR}10|\text{TAR}} &= \frac{q_{\text{vir}10}^\psi + c_2 q_{\text{vir}10}^\phi}{C}, \\
p_{\text{REF}10|\text{REF}} &= \frac{2c_1 q_{\text{vir}10}^\phi}{C}, \\
p_{\text{TAR}11|\text{TAR}} &= \frac{q_{\text{vir}11}^\psi + 4c_1 c_2 q_{\text{vir}11}^\phi}{C}, \\
p_{\text{REF}11|\text{REF}} &= \frac{(4c_1^2 + c_2^2) q_{\text{vir}11}^\phi}{C},
\end{aligned} \tag{S190}$$

with

$$C = q_{\text{vir}00}^\phi + 2c_1 q_{\text{vir}01}^\phi + 2c_1 q_{\text{vir}10}^\phi + (4c_1^2 + c_2^2) q_{\text{vir}11}^\phi. \tag{S191}$$

Now, applying Bayes' Theorem (see Eq. (S137)), and using  $p_{\text{TAR}} = \sum_{\alpha,\beta} p_{\text{TAR}\alpha\beta}$ ,  $p_{\text{REF}} = \sum_{\alpha,\beta} p_{\text{REF}\alpha\beta}$ ,  $p_{\text{TAR}} = p_{\text{REF}}$ ,  $p_{\text{TAR}\alpha\beta} = p_{\text{TAR}} p_{\text{TAR}\alpha\beta|\text{TAR}}$ , and  $p_{\text{REF}\alpha\beta} = p_{\text{REF}} p_{\text{REF}\alpha\beta|\text{REF}}$  (see Eqs. (S139) and (S140)), we obtain the fictitious tag assignment probabilities

$$\begin{aligned}
p_{\text{TAR}|\text{vir}} &:= p_{\text{TAR}00|\text{vir}00} = p_{\text{TAR}01|\text{vir}01} = p_{\text{TAR}10|\text{vir}10} = p_{\text{TAR}11|\text{vir}11} = \frac{p_{\text{TAR}}}{p_Z^2 p_{\text{key}|Z} C}, \\
p_{\text{REF}00|0_X 0_X} &= \frac{p_{\text{TAR}} q_{\text{vir}00}^\phi}{p_X^2 C}, \\
p_{\text{TAR}01|0_X 0_X} &= p_{\text{TAR}10|0_X 0_X} = \frac{p_{\text{TAR}} c_2 q_{\text{vir}01}^\phi}{p_X^2 C}, \\
p_{\text{REF}01|0_X 0_Z} &= p_{\text{REF}01|0_X 1_Z} = p_{\text{REF}10|0_Z 0_X} = p_{\text{REF}10|1_Z 0_X} = \frac{2p_{\text{TAR}} c_1 q_{\text{vir}01}^\phi}{p_X p_Z C}, \\
p_{\text{TAR}11|0_Z 0_X} &= p_{\text{TAR}11|1_Z 0_X} = p_{\text{TAR}11|0_X 0_Z} = p_{\text{TAR}11|0_X 1_Z} = \frac{2p_{\text{TAR}} c_1 c_2 q_{\text{vir}11}^\phi}{p_X p_Z C}, \\
p_{\text{REF}11|0_Z 0_Z} &= p_{\text{REF}11|1_Z 0_Z} = p_{\text{REF}11|0_Z 1_Z} = p_{\text{REF}11|1_Z 1_Z} = \frac{4p_{\text{TAR}} c_1^2 q_{\text{vir}11}^\phi}{p_Z^2 p_{\text{test}|Z} C}, \\
p_{\text{REF}11|0_X 0_X} &= \frac{p_{\text{TAR}} c_2^2 q_{\text{vir}11}^\phi}{p_X^2 C},
\end{aligned} \tag{S192}$$

where (see Eq. (S142))

$$p_{\text{TAR}} = C \min \left\{ p_Z^2 p_{\text{key}|Z}, \frac{p_Z p_X}{2(c_1 c_2 q_{\text{vir}11}^\phi + c_1 q_{\text{vir}01}^\phi)}, \frac{p_Z^2 p_{\text{test}|Z}}{4c_1^2 q_{\text{vir}11}^\phi}, \frac{p_X^2}{q_{\text{vir}00}^\phi + 2c_2 q_{\text{vir}01}^\phi + c_2^2 q_{\text{vir}11}^\phi} \right\}, \tag{S193}$$

with  $p_X := 1 - p_Z$  and  $p_{\text{test}|Z} := 1 - p_{\text{key}|Z}$ .

After making all these definitions, one can directly use the analysis in Section SM2 to obtain our bound on  $N_{\text{ph}}$ .

In this scenario, Eq. (S144) becomes

$$\begin{aligned}
N_{ZC=0}^{\text{err}} &= N_{\text{ph},\text{TAR},ZC} + N_{0Z0X,\text{TAR}11,ZC}^{\text{det}} + N_{1Z0X,\text{TAR}11,ZC}^{\text{det}} + N_{0X0Z,\text{TAR}11,ZC}^{\text{det}} + N_{0X1Z,\text{TAR}11,ZC}^{\text{det}}, \\
N_{ZC=1}^{\text{err}} &= N_{0X0X,\text{REF}00,ZC}^{\text{det}} + N_{0Z0Z,\text{REF}11,ZC}^{\text{det}} + N_{0Z1Z,\text{REF}11,ZC}^{\text{det}} + N_{1Z0Z,\text{REF}11,ZC}^{\text{det}} + N_{1Z1Z,\text{REF}11,ZC}^{\text{det}} + N_{0X0X,\text{REF}11,ZC}^{\text{det}}, \\
N_{ZC=0}^{\text{det}} &= N_{\text{key},\text{TAR},ZC}^{\text{det}} + N_{0Z0X,\text{TAR}11,ZC}^{\text{det}} + N_{1Z0X,\text{TAR}11,ZC}^{\text{det}} + N_{0X0Z,\text{TAR}11,ZC}^{\text{det}} + N_{0X1Z,\text{TAR}11,ZC}^{\text{det}} \\
&\quad + N_{0X0X,\text{TAR}01,ZC}^{\text{det}} + N_{0X0X,\text{TAR}10,ZC}^{\text{det}}, \\
N_{ZC=1}^{\text{det}} &= N_{0X0X,\text{REF}00,ZC}^{\text{det}} + N_{0Z0Z,\text{REF}11,ZC}^{\text{det}} + N_{0Z1Z,\text{REF}11,ZC}^{\text{det}} + N_{1Z0Z,\text{REF}11,ZC}^{\text{det}} + N_{1Z1Z,\text{REF}11,ZC}^{\text{det}} \\
&\quad + N_{0X0X,\text{REF}11,ZC}^{\text{det}} + N_{0X0Z,\text{REF}01,ZC}^{\text{det}} + N_{0X1Z,\text{REF}01,ZC}^{\text{det}} + N_{0Z0X,\text{REF}10,ZC}^{\text{det}} + N_{1Z0X,\text{REF}10,ZC}^{\text{det}},
\end{aligned} \tag{S194}$$

and Eq. (S145) becomes

$$\begin{aligned}
N_{ZC=0}^{\text{err}} &\simeq p_{ZC} \left( p_{\text{TAR}|\text{vir}} N_{\text{ph}} + p_{\text{TAR}11|0Z0X} N_{0Z0X}^{\text{det}} + p_{\text{TAR}11|1Z0X} N_{1Z0X}^{\text{det}} + p_{\text{TAR}11|0X0Z} N_{0X0Z}^{\text{det}} + p_{\text{TAR}11|0X1Z} N_{0X1Z}^{\text{det}} \right), \\
N_{ZC=1}^{\text{err}} &\simeq p_{ZC} \left( p_{\text{REF}00|0X0X} N_{0X0X}^{\text{det}} + p_{\text{REF}11|0Z0Z} N_{0Z0Z}^{\text{det}} + p_{\text{REF}11|0Z1Z} N_{0Z1Z}^{\text{det}} + p_{\text{REF}11|1Z0Z} N_{1Z0Z}^{\text{det}} \right. \\
&\quad \left. + p_{\text{REF}11|1Z1Z} N_{1Z1Z}^{\text{det}} + p_{\text{REF}11|0X0X} N_{0X0X}^{\text{det}} \right), \\
N_{ZC=0}^{\text{det}} &\simeq p_{ZC} \left( p_{\text{TAR}|\text{vir}} N_{\text{key}}^{\text{det}} + p_{\text{TAR}11|0Z0X} N_{0Z0X}^{\text{det}} + p_{\text{TAR}11|1Z0X} N_{1Z0X}^{\text{det}} + p_{\text{TAR}11|0X0Z} N_{0X0Z}^{\text{det}} + p_{\text{TAR}11|0X1Z} N_{0X1Z}^{\text{det}} \right. \\
&\quad \left. + p_{\text{TAR}01|0X0X} N_{0X0X}^{\text{det}} + p_{\text{TAR}10|0X0X} N_{0X0X}^{\text{det}} \right), \\
N_{ZC=1}^{\text{det}} &\simeq p_{ZC} \left( p_{\text{REF}00|0X0X} N_{0X0X}^{\text{det}} + p_{\text{REF}11|0Z0Z} N_{0Z0Z}^{\text{det}} + p_{\text{REF}11|0Z1Z} N_{0Z1Z}^{\text{det}} + p_{\text{REF}11|1Z0Z} N_{1Z0Z}^{\text{det}} + p_{\text{REF}11|1Z1Z} N_{1Z1Z}^{\text{det}} \right. \\
&\quad \left. + p_{\text{REF}11|0X0X} N_{0X0X}^{\text{det}} + p_{\text{REF}01|0X0Z} N_{0X0Z}^{\text{det}} + p_{\text{REF}01|0X1Z} N_{0X1Z}^{\text{det}} + p_{\text{REF}10|0Z0X} N_{0Z0X}^{\text{det}} + p_{\text{REF}10|1Z0X} N_{1Z0X}^{\text{det}} \right),
\end{aligned} \tag{S195}$$

where  $p_{t|ij}$  and  $p_{\text{TAR}|\text{vir}}$  are given by Eq. (S192). After substituting these expressions in the coin protocol inequality (Eq. (S43)) and isolating  $N_{\text{ph}}$ , we obtain the desired bound. Note that, to evaluate this bound, one needs an upper bound on the coin imbalance parameter  $\Delta := 1 - \text{Re} \langle \Psi_{\text{TAR}} | \Psi_{\text{Ref}} \rangle_{DAB}$ . Using Eqs. (S188), (S189) and related definitions, we can derive the inner product  $\langle \Psi_{\text{TAR}} | \Psi_{\text{Ref}} \rangle_{DAB}$  to be

$$\begin{aligned}
\langle \Psi_{\text{TAR}} | \Psi_{\text{Ref}} \rangle_{DAB} &= \frac{q_{\text{vir}0}^{\phi}}{4C} \left[ \langle \psi_{0X0X} | \psi_{0Z0Z} \rangle_{B_a B_b} + \langle \psi_{0X0X} | \psi_{0Z1Z} \rangle_{B_a B_b} + \langle \psi_{0X0X} | \psi_{1Z0Z} \rangle_{B_a B_b} + \langle \psi_{0X0X} | \psi_{1Z1Z} \rangle_{B_a B_b} \right] \\
&+ \frac{\sqrt{2c_1 q_{\text{vir}01}^{\phi}}}{2C} \left[ \frac{1}{4} \left( \langle \psi_{0X0Z} | \psi_{0Z0Z} \rangle_{B_a B_b} - \langle \psi_{0X0Z} | \psi_{0Z1Z} \rangle_{B_a B_b} + \langle \psi_{0X0Z} | \psi_{1Z0Z} \rangle_{B_a B_b} - \langle \psi_{0X0Z} | \psi_{1Z1Z} \rangle_{B_a B_b} \right. \right. \\
&- \langle \psi_{0X1Z} | \psi_{0Z0Z} \rangle_{B_a B_b} + \langle \psi_{0X1Z} | \psi_{0Z1Z} \rangle_{B_a B_b} - \langle \psi_{0X1Z} | \psi_{1Z0Z} \rangle_{B_a B_b} + \langle \psi_{0X1Z} | \psi_{1Z1Z} \rangle_{B_a B_b} + \langle \psi_{0Z0X} | \psi_{0Z0Z} \rangle_{B_a B_b} \\
&+ \langle \psi_{0Z0X} | \psi_{0Z1Z} \rangle_{B_a B_b} - \langle \psi_{0Z0X} | \psi_{1Z0Z} \rangle_{B_a B_b} - \langle \psi_{0Z0X} | \psi_{1Z1Z} \rangle_{B_a B_b} - \langle \psi_{1Z0X} | \psi_{0Z0Z} \rangle_{B_a B_b} - \langle \psi_{1Z0X} | \psi_{0Z1Z} \rangle_{B_a B_b} \\
&+ \langle \psi_{1Z0X} | \psi_{1Z0Z} \rangle_{B_a B_b} + \langle \psi_{1Z0X} | \psi_{1Z1Z} \rangle_{B_a B_b} \left. \right) + \sqrt{c_2 q_{\text{vir}01}^{\phi}} \left( \langle \psi_{0X0Z} | \psi_{0X0X} \rangle_{B_a B_b} + \langle \psi_{0X1Z} | \psi_{0X0X} \rangle_{B_a B_b} \right. \\
&+ \langle \psi_{0Z0X} | \psi_{0X0X} \rangle_{B_a B_b} + \langle \psi_{1Z0X} | \psi_{0X0X} \rangle_{B_a B_b} \left. \right) + \frac{c_1 q_{\text{vir}1}^{\phi}}{4C} \left( 2 - \langle \psi_{0Z0Z} | \psi_{0Z1Z} \rangle_{B_a B_b} - \langle \psi_{0Z0Z} | \psi_{1Z0Z} \rangle_{B_a B_b} \right. \\
&+ \langle \psi_{0Z0Z} | \psi_{1Z1Z} \rangle_{B_a B_b} + \langle \psi_{0Z1Z} | \psi_{1Z0Z} \rangle_{B_a B_b} - \langle \psi_{0Z1Z} | \psi_{1Z1Z} \rangle_{B_a B_b} - \langle \psi_{1Z0Z} | \psi_{1Z1Z} \rangle_{B_a B_b} \left. \right) + \frac{q_{\text{vir}11}^{\phi} \sqrt{c_1 c_2}}{2\sqrt{2}C} \\
&\times \left[ c_1 \left( \langle \psi_{0Z0Z} | \psi_{0Z0X} \rangle_{B_a B_b} - \langle \psi_{0Z0Z} | \psi_{1Z0X} \rangle_{B_a B_b} + 2 \langle \psi_{0Z0Z} | \psi_{0X0Z} \rangle_{B_a B_b} + \langle \psi_{0Z1Z} | \psi_{0Z0X} \rangle_{B_a B_b} - \langle \psi_{0Z1Z} | \psi_{1Z0X} \rangle_{B_a B_b} \right. \right. \\
&+ 2 \langle \psi_{0Z1Z} | \psi_{0X1Z} \rangle_{B_a B_b} - \langle \psi_{1Z0Z} | \psi_{0Z0X} \rangle_{B_a B_b} + \langle \psi_{1Z0Z} | \psi_{1Z0X} \rangle_{B_a B_b} + 2 \langle \psi_{1Z0Z} | \psi_{0X0Z} \rangle_{B_a B_b} - \langle \psi_{1Z1Z} | \psi_{0Z0X} \rangle_{B_a B_b} \\
&+ \langle \psi_{1Z1Z} | \psi_{1Z0X} \rangle_{B_a B_b} + 2 \langle \psi_{1Z1Z} | \psi_{0X1Z} \rangle_{B_a B_b} \left. \right) + 2c_2 \left( \langle \psi_{0X0X} | \psi_{0Z0X} \rangle_{B_a B_b} + \langle \psi_{0X0X} | \psi_{1Z0X} \rangle_{B_a B_b} \right) \left. \right].
\end{aligned} \tag{S196}$$

Using this expression and the assumption on the emitted states in Eq. (S173), one can obtain an upper bound on  $\Delta$  by solving an SDP; see Section SE2 B for the full construction of this SDP.

In Fig. S7, we evaluate the asymptotic secret-key rate obtainable using our analysis. For the simulations, we use the channel model in Section SE3 B, set  $p_Z = p_{\text{key}|Z} = p_{Z_C} = 0.9$  and consider the following experimental parameters: error correction inefficiency  $f = 1.16$  and dark count probability  $p_d = 10^{-8}$  [S29, S30]. For comparison, we also plot the secret-key rate obtainable using the previous analysis [S34]. Remarkably, despite considering a more general class of attacks, our proof can actually obtain considerably higher key rates than that of [S34], even in terms of secret bits per pulse. We note that, in practice, to apply the proof in [S34] rigorously, one would need to run the protocol at a low repetition rate to ensure sequentiality (see Section SM5), and therefore the performance advantage offered by our security proof would be even more pronounced if plotted in terms of bits per second<sup>7</sup>.

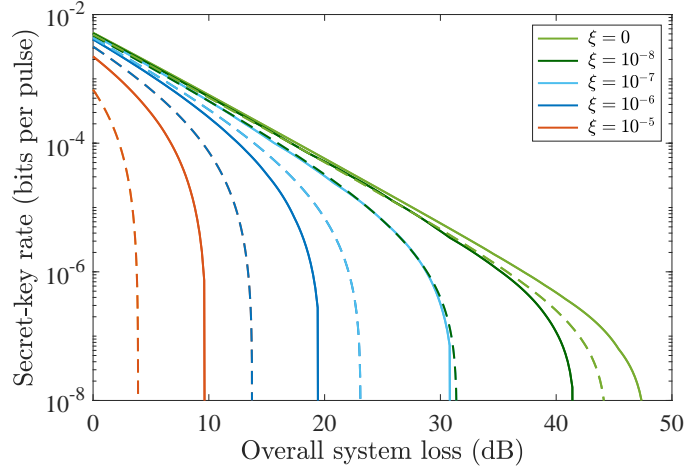

Figure S7. Asymptotic secret-key rate (in bits per pulse) for the coherent-light-based MDI scheme for several values of  $\xi = 1 - (1 - \epsilon)^2 \approx 2\epsilon$  using our analysis (solid lines), compared with the previous analysis in [S34] (dashed lines). For each value of the system loss, we have optimized the intensity  $\mu$  of the emitted coherent states. We note that the previous analysis is only valid against sequential attacks, while our analysis can protect against the most general attacks allowed by quantum mechanics.

### 3. Finite-key analysis

In the finite-key regime, we can simply apply the general analysis for MDI-type scenarios in Section SM2 D. Precisely, let us define

$$\begin{aligned}\overline{N}_{ij,t,Z_C}^{\text{det}} &= p_{Z_C} p_{t|ij} N_{ij}^{\text{det}} \pm \Delta_C^\pm(p_{Z_C} p_{t|ij} N_{ij}^{\text{det}}), \\ \overline{N}_{\text{key,TAR},Z_C}^{\text{det}} &= p_{Z_C} p_{\text{TAR}|\text{vir}} N_{\text{key}}^{\text{det}} \pm \Delta_C^\pm(p_{Z_C} p_{\text{TAR}|\text{vir}} N_{\text{key}}^{\text{det}}), \\ \overline{N}_{X_C=1} &= N p_{\text{TAR}} p_{X_C} \Delta + \Delta_C^+(N p_{\text{TAR}} p_{X_C} \Delta),\end{aligned}\tag{S197}$$

where  $p_{Z_C} \in (0, 1)$  is a fictitious probability that affects the statistical deviation terms and should be optimized for best performance,  $p_{X_C} := 1 - p_{Z_C}$ ,  $i, j \in \{0_Z, 1_Z, 0_X\}$ ,  $t \in \{\text{TAR00}, \text{TAR01}, \text{TAR10}, \text{TAR11}, \text{REF00}, \text{REF01}, \text{REF10}, \text{REF11}\}$ ,  $p_{t|ij}$  and  $p_{\text{TAR}|\text{vir}}$  are given by Eq. (S192);  $p_{\text{TAR}}$  is given by Eq. (S193);  $\Delta_C^-(x) = \sqrt{2x \ln(1/\epsilon_C)}$  and  $\Delta_C^+(x) = \sqrt{3x \ln(1/\epsilon_C)}$  (see Eq. (S104));  $N_{ij}^{\text{det}}$  is the observed number of detected events in which Alice emitted  $|\psi_i\rangle_{B_a}$ , Bob emitted  $|\psi_j\rangle_{B_b}$ , Charlie announced a detection, and the round was assigned to “test”;  $N_{\text{key}}^{\text{det}}$  is the size of the sifted key, i.e., the number of rounds in which  $i, j \in \{0_Z, 1_Z\}$ , Charlie announced a detection and the round was assigned to “key”; and  $\Delta$  is the coin imbalance parameter. Also, let us define

<sup>7</sup> As discussed at the end of Section SM5, ensuring sequentiality for MDI protocols is not as straightforward as for P&M protocols. For this reason, we do not include a comparison in terms of secret-key bits per second for this protocol.

$$\begin{aligned}
\overline{N}_{Z_C=1}^{\text{err}} &:= \overline{N}_{0_X 0_X, \text{REF}00, Z_C}^{\text{det}} + \overline{N}_{0_Z 0_Z, \text{REF}11, Z_C}^{\text{det}} + \overline{N}_{0_Z 1_Z, \text{REF}11, Z_C}^{\text{det}} + \overline{N}_{1_Z 0_Z, \text{REF}11, Z_C}^{\text{det}} \\
&\quad + \overline{N}_{1_Z 1_Z, \text{REF}11, Z_C}^{\text{det}} + \overline{N}_{0_X 0_X, \text{REF}11, Z_C}^{\text{det}}, \\
\overline{N}_{Z_C=0}^{\text{det}} &:= \overline{N}_{\text{key}, \text{TAR}, Z_C}^{\text{det}} + \overline{N}_{0_Z 0_X, \text{TAR}11, Z_C}^{\text{det}} + \overline{N}_{1_Z 0_X, \text{TAR}11, Z_C}^{\text{det}} + \overline{N}_{0_X 0_Z, \text{TAR}11, Z_C}^{\text{det}} + \overline{N}_{0_X 1_Z, \text{TAR}11, Z_C}^{\text{det}} \\
&\quad + \overline{N}_{0_X 0_X, \text{TAR}01, Z_C}^{\text{det}} + \overline{N}_{0_X 0_X, \text{TAR}10, Z_C}^{\text{det}}, \\
\overline{N}_{Z_C=1}^{\text{det}} &:= \overline{N}_{0_X 0_X, \text{REF}00, Z_C}^{\text{det}} + \overline{N}_{0_Z 0_Z, \text{REF}11, Z_C}^{\text{det}} + \overline{N}_{0_Z 1_Z, \text{REF}11, Z_C}^{\text{det}} + \overline{N}_{1_Z 0_Z, \text{REF}11, Z_C}^{\text{det}} + \overline{N}_{1_Z 1_Z, \text{REF}11, Z_C}^{\text{det}} \\
&\quad + \overline{N}_{0_X 0_X, \text{REF}11, Z_C}^{\text{det}} + \overline{N}_{0_X 0_Z, \text{REF}01, Z_C}^{\text{det}} + \overline{N}_{0_X 1_Z, \text{REF}01, Z_C}^{\text{det}} + \overline{N}_{0_Z 0_X, \text{REF}10, Z_C}^{\text{det}} + \overline{N}_{1_Z 0_X, \text{REF}10, Z_C}^{\text{det}}.
\end{aligned} \tag{S198}$$

Then, we have the following statistical bound on the number of phase errors

$$\begin{aligned}
N_{\text{ph}} \leq \frac{1}{\epsilon_{\text{tot}} p_{Z_C} p_{\text{TAR}|\text{vir}}} &\left[ (\overline{N}_{Z_C=0}^{\text{det}} + \Delta_A) G_+ \left( \frac{\overline{N}_{Z_C=1}^{\text{err}} + \Delta_A}{\overline{N}_{Z_C=1}^{\text{det}} - \Delta_A}, 1 - \frac{2p_{Z_C}(\overline{N}_{X_C=1} + \Delta_A)}{p_{X_C}(\overline{N}_{Z_C=0}^{\text{det}} + \overline{N}_{Z_C=1}^{\text{det}} - \Delta_A)} \right) \right. \\
&\quad \left. - \overline{N}_{0_Z 0_X, \text{TAR}11, Z_C}^{\text{det}} - \overline{N}_{1_Z 0_X, \text{TAR}11, Z_C}^{\text{det}} - \overline{N}_{0_X 0_Z, \text{TAR}11, Z_C}^{\text{det}} - \overline{N}_{0_X 1_Z, \text{TAR}11, Z_C}^{\text{det}} + \Delta_A + \Delta_H \right] =: N_{\text{ph}}^{\text{U}},
\end{aligned} \tag{S199}$$

where  $\epsilon_{\text{tot}} = 6\epsilon_A + 31\epsilon_C + \epsilon_H$ ,  $\Delta_A := \sqrt{2N_{\text{key}}^{\text{det}} \ln(1/\epsilon_A)}$  and  $\Delta_H := \sqrt{N_{\text{key}}^{\text{det}} \ln(1/\epsilon_H)/2}$  (see Section SM1 E 1 for more details), and the function  $G_+(y, z)$  is defined in Eq. (S39).

In Fig. S8, we show the secret-key rate offered by our analysis in the finite-key regime. For the simulations, we have used the channel model in Section SE3 B, the same experimental parameters as in Fig. S7, and have optimized over the probabilities  $p_Z$ ,  $p_{\text{key}|Z}$  and  $p_{Z_C}$ , and over the intensity of the coherent pulses  $\mu$ . Moreover, we have selected  $\epsilon_{\text{seccr}} = \epsilon_{\text{corr}} = 10^{-10}$  [S31] and for simplicity, we have set  $\epsilon_C = \epsilon_H = \epsilon_A =: \hat{\epsilon}$ , from which it follows that  $\epsilon_{\text{tot}} = 38\hat{\epsilon}$ . For simplicity, we have also assumed that  $\epsilon_{\text{PA}} = \epsilon_{\text{tot}}$ , and therefore  $\epsilon_{\text{tot}} = \epsilon_{\text{seccr}}^2/4$ . To evaluate the achievable secret-key rate under different amounts of information leakage, we have considered  $\epsilon \in \{10^{-6}, 10^{-8}\}$ . The figures show that our security analysis achieves a reasonable finite-key scaling for practical values of  $N$ , and in fact compares favorably with that of other MDI protocols (see, e.g., [S44]).

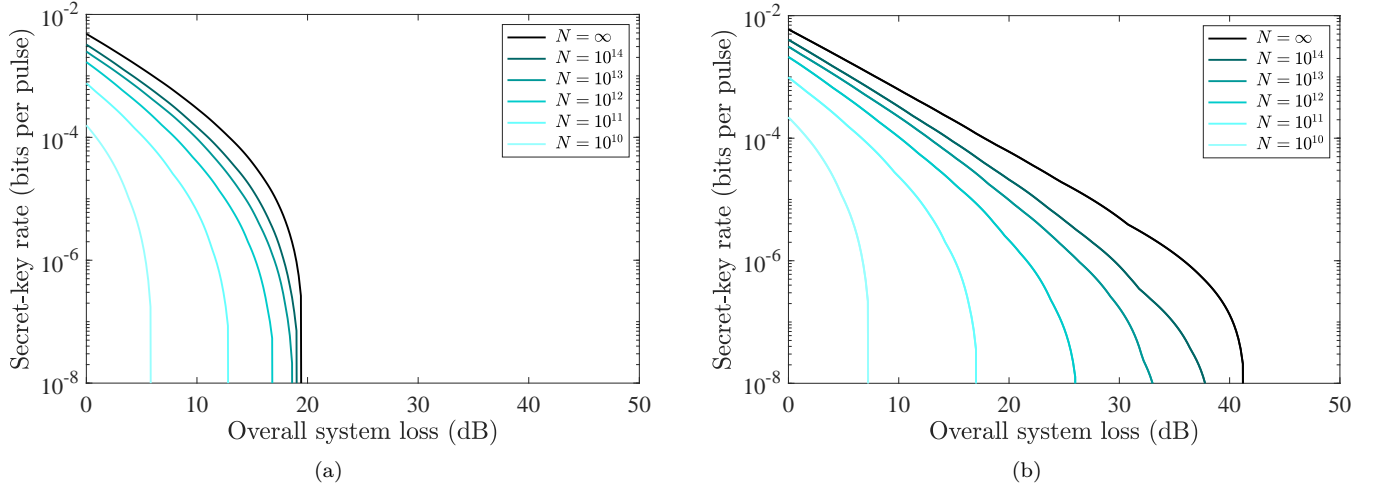

Figure S8. Finite-size secret-key rate (in bits per pulse) as a function of the overall system loss when applying our analysis to the coherent-light-based MDI scheme proposed by [S34] and using Azuma's inequality to derive the quantum coin inequality. We consider different values of the block size  $N$  and take (a)  $\xi = 10^{-6}$  and (b)  $\xi = 10^{-8}$ .

To generate the results in Fig. S8, we have used the phase-error rate bound in Eq. (S199), which was derived using Azuma's inequality. As explained in Section SM1 E, one can also substitute Azuma's inequality by Kato's inequality [S25], which requires the users to make a prediction about the experimental results that they expect to obtain after running the protocol. If the predictions are close to the actual observed outcomes, using this inequality improves the finite-key scaling, as can be seen in Fig. S9, which assumes optimal predictions. In particular, using Kato's inequality, a positive secret-key rate could be achieved even with a block size of just  $10^9$  transmitted signals.

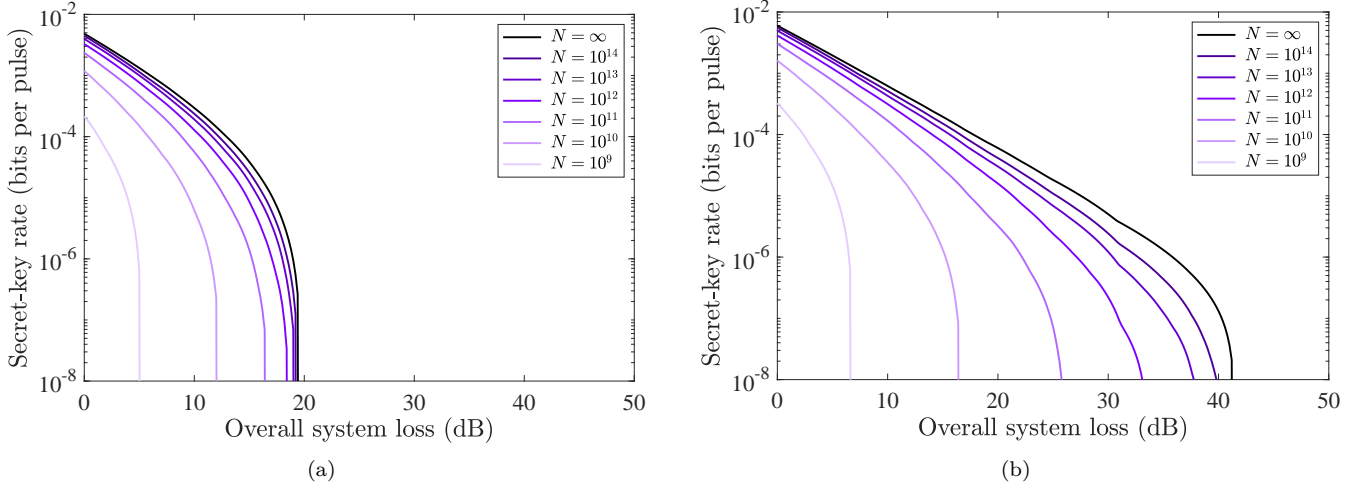

Figure S9. Finite-size secret-key rate (in bits per pulse) as a function of the overall system loss when applying our analysis to the coherent-light-based MDI scheme proposed by [S34] and using Kato's inequality to derive the quantum coin inequality. We consider different values of the block size  $N$  and take (a)  $\epsilon = 10^{-6}$  and (b)  $\epsilon = 10^{-8}$ .

## B. Decoy-state protocols

Here, we discuss how our security proof can be combined with the decoy-state method [S41–S43] and applied to the scenario in which the light source emits intensity-modulated phase-randomized (PR) WCPs. First, in Section SM4 B 1, we explain how the standard decoy-state analysis can be incorporated into our proof under the typical assumption that the intensity modulation and phase randomization processes are ideal. Then, in Section SM4 B 2, we show how our techniques could also be used to address the more realistic scenario in which these processes suffer from imperfections, including side channels.

### 1. Ideal PR-WCP light sources

Under the assumption of perfect intensity modulation and phase randomization, given that the intensity  $\mu$  has been chosen, the state produced by a weak laser source is

$$\rho_\mu = \frac{1}{2\pi} \int_0^{2\pi} |\sqrt{\mu}e^{i\theta}\rangle\langle\sqrt{\mu}e^{i\theta}| d\theta = \sum_{n=0}^{\infty} p_{n|\mu} |n\rangle\langle n|, \quad (\text{S200})$$

where  $|n\rangle$  is the  $n$ -th Fock state and  $p_{n|\mu}$  follows a Poisson distribution of mean  $\mu$ . The state  $\rho_\mu$  produced by the laser source then goes through an imperfect modulator that encodes the bit-and-basis setting choice  $j$  into it. The action of this modulator can, without loss of generality, be represented as an isometric operator  $\hat{V}_j$ , resulting in

$$\rho_{j,\mu} = \hat{V}_j \rho_\mu \hat{V}_j^\dagger = \sum_{n=0}^{\infty} p_{n|\mu} |\psi_j^{(n)}\rangle\langle\psi_j^{(n)}|_B, \quad (\text{S201})$$

where the eigenstates of  $\rho_{j,\mu}$ ,  $|\psi_j^{(n)}\rangle_B := \hat{V}_j |n\rangle$ , are independent of the intensity choice  $\mu$ . In this scenario, we can apply our security proof as long as Eq. (S1) holds for the single-photon emissions, i.e., as long as

$$|\langle\phi_j^{(1)}|\psi_j^{(1)}\rangle_B|^2 \geq 1 - \epsilon, \quad (\text{S202})$$

where  $\{|\phi_j^{(1)}\rangle_B\}_j$  is a set of characterized qubit states. To determine the amount of privacy amplification that needs to be applied to the sifted key pair to turn it into a secure key pair, we need to obtain the following: (1) a lower bound on the number of bits in the sifted key that originate from single-photon emissions,  $N_{\text{key}}^{\text{det},(1)}$ ; (2) an upper bound on the number of phase errors within these bits,  $N_{\text{ph}}^{(1)}$ .

Let us start by discussing the second term. The set of single-photon emissions effectively constitutes a subprotocol that is indistinguishable from a scenario in which the light source is a single-photon source. Therefore, our existing analysis can be applied to obtain a bound on the number of phase errors within this subprotocol,  $N_{\text{ph}}^{(1)}$ , in terms of the outcomes of the test rounds within the subprotocol,  $N_j^{\beta_X, (1)}$ . Specifically, Eq. (S116) applies to this scenario after making the substitutions  $N_{\text{ph}} \rightarrow N_{\text{ph}}^{(1)}$  and  $N_j^{\beta_X} \rightarrow N_j^{\beta_X, (1)}$ . The only difference with the single-photon source case is that now the quantities  $N_j^{\beta_X, (1)}$  cannot be directly observed, since the users do not know the photon number of each pulse. Nevertheless, one can simply use the observed values of  $N_{j, \mu}^{\beta_X}$  in combination with the standard decoy-state analysis to obtain appropriate lower or upper bounds on these quantities. Assuming first the asymptotic regime for simplicity of discussion, we have that  $N_{j, \mu}^{\beta_X} \simeq N p_\mu p_j Q_{j, \mu}^{\beta_X}$  and  $N_j^{\beta_X, (1)} \simeq N p_j Y_j^{\beta_X, (1)}$ , and a bound on  $Y_j^{\beta_X, (1)}$  can be expressed as the linear program

$$\begin{aligned} & \min/\max Y_j^{\beta_X, (1)} \\ & \text{s.t. } Q_{j, \mu}^{\beta_X} = \sum_n p_{n|\mu} Y_j^{\beta_X, (n)}, \quad \forall \mu. \end{aligned} \quad (\text{S203})$$

In an actual finite-key implementation, one needs to modify this linear program by applying concentration inequalities to take into account statistical fluctuations, as shown in [S45]. Similarly, a lower bound on  $N_{\text{key}}^{\text{det}, (1)}$  can also be obtained using linear programming. Analogously to Eq. (S117), the length of the secret key obtainable can then be expressed as

$$N_{\text{sec}} = N_{\text{key}}^{\text{det}, (1), \text{L}} \left[ 1 - h \left( \frac{N_{\text{ph}}^{(1), \text{U}}}{N_{\text{key}}^{\text{det}, (1), \text{L}}} \right) \right] - \lambda_{\text{EC}} - \log_2 \frac{1}{\epsilon_{\text{corr}}} - \log_2 \frac{1}{\epsilon_{\text{PA}}}, \quad (\text{S204})$$

and this key is  $(\epsilon_{\text{corr}} + \epsilon_{\text{secre}})$ -secure with  $\epsilon_{\text{secre}} = \sqrt{2} \sqrt{\epsilon_{\text{tot}} + \epsilon_{\text{PA}}}$ , where  $\epsilon_{\text{tot}}$  now refers to the sum of all concentration inequalities applied, both in our analysis and in the decoy-state analysis.

## 2. Realistic PR-WCP light sources

In practice, both the intensity modulation and the phase randomization processes may be imperfect. Previous works have looked at many of these imperfections, such as information leakage of the intensity setting [S17], intensity correlations [S46, S47], non-uniform phase randomization [S48, S49], and correlations between the phases of consecutive laser pulses [S50]. These imperfections, although distinct in nature, have a similar impact in the security of the protocol. Namely, in their presence, the eigenstates of the pulses generated by the light source are no longer perfect Fock states that are independent of the intensity setting  $\mu$ , i.e., Eq. (S200) now becomes

$$\rho_\mu = \sum_n p_{n|\mu} |n_\mu\rangle\langle n_\mu|. \quad (\text{S205})$$

Due to the dependence of the eigenstates on the intensity  $\mu$ , the standard decoy-state method presented in the previous Section cannot be directly applied. Still, given that the overall magnitude of the imperfections is not too large, we should have that  $|n_\mu\rangle \approx |n\rangle$ , and by quantifying the magnitude of the imperfections, one should be able to obtain a bound of the form

$$|\langle n | n_\mu \rangle|^2 \geq 1 - \epsilon_n. \quad (\text{S206})$$

Note that Eq. (S206) has a similar form to Eq. (S1). In what follows, we show how the ideas and formalism introduced by our security proof can also be used to prove security in this scenario.

After the pulse  $\rho_\mu$  goes through the (imperfect) modulation process, it becomes

$$\rho_{j, \mu} = \hat{V}_j \rho_\mu \hat{V}_j^\dagger = \sum_n p_{n|\mu} |\psi_{j, \mu}^{(n)}\rangle\langle\psi_{j, \mu}^{(n)}|_B, \quad (\text{S207})$$

where the eigenstates of  $\rho_{j, \mu}$ ,  $|\psi_{j, \mu}^{(n)}\rangle_B := \hat{V}_j |n_\mu\rangle$ , now depend on the intensity choice  $\mu$ . Still, due to Eq. (S206), we must have that

$$|\langle \psi_j^{(n)} | \psi_{j, \mu}^{(n)} \rangle_B|^2 \geq 1 - \epsilon_n, \quad (\text{S208})$$

where  $|\psi_j^{(n)}\rangle_B := \hat{V}_j |n\rangle$  is a state that does not depend on the intensity setting  $\mu$ .

Let us first assume the asymptotic regime for clarity. If  $\epsilon_n$  is small, the difference between the detection statistics of the states  $|\psi_{j,\mu}^{(n)}\rangle_B$  and  $|\psi_{j,\nu}^{(n)}\rangle_B$  for  $\mu \neq \nu$  cannot be very large. In particular, similarly to our security proof, one can consider a quantum coin state of the form

$$|\Psi_{j,\mu,\nu}^{(n)}\rangle_{CB} = \frac{1}{\sqrt{2}}(|0\rangle_C |\psi_{j,\mu}^{(n)}\rangle_B + |1\rangle_C |\psi_{j,\nu}^{(n)}\rangle_B), \quad (\text{S209})$$

and then evaluate the probability to obtain the outcome  $X_C = 1$  if system  $C$  is measured in the  $X$  basis to derive a bound of the form  $|Y_{j,\mu}^{(n)} - Y_{j,\nu}^{(n)}| \leq \Delta_{\mu,\nu}^{(n)}$ . Using this bound, we can modify the linear program in Eq. (S203) as

$$\begin{aligned} & \min/\max Y_{j,\mu_s}^{\beta_X, (1)} \\ & \text{s.t. } Q_{j,\mu}^{\beta_X} = \sum_n p_{n|\mu} Y_{j,\mu}^{\beta_X, (n)}, \quad \forall \mu \\ & |Y_{j,\mu}^{(n)} - Y_{j,\nu}^{(n)}| \leq \Delta_{\mu,\nu}^{(n)}, \quad \forall \mu, \nu. \end{aligned} \quad (\text{S210})$$

This idea can be turned into a rigorous security proof against general attacks that takes into account finite-size effects by applying the methodology introduced in our analysis. For this, one needs to define a fictitious scenario in which Alice probabilistically assigns tags to her emissions of  $|\psi_{j,\mu}^{(n)}\rangle_B$  and  $|\psi_{j,\nu}^{(n)}\rangle_B$ , in such a way that a tagged emission can be regarded as equivalent to that originating from  $|\Psi_{j,\mu,\nu}^{(n)}\rangle_{CB}$ . Then, by considering that Alice sometimes measures the quantum coin system  $C$  in the  $X$  basis, and deriving a bound on the maximum number of events in which she could have obtained the outcome  $X_C = 1$ , one can use the quantum coin inequality to bound the maximum deviation between the number of detected events in which Alice sent  $|\psi_{j,\mu}^{(n)}\rangle_B$  and  $|\psi_{j,\nu}^{(n)}\rangle_B$  within the tagged rounds. Finally, one can apply concentration inequalities to derive bounds on the maximum deviation between the total number of detected events in which Alice emitted these states,  $N_{j,\mu}^{(n)}$  and  $N_{j,\nu}^{(n)}$ , and use these bounds to construct an appropriate finite-size linear program to obtain appropriate bounds on  $N_{j,\mu_s}^{\beta_X, (1)}$ . After these are obtained, one simply substitutes them into Eq. (S116) to get an upper bound on  $N_{\text{ph}}^{(1)}$ . Using very similar ideas, one can also derive a lower bound on  $N_{\text{key}}^{\text{det}, (1)}$ , and then simply substitute these bounds into Eq. (S204) to evaluate the length of the secret key that can be distilled. In any case, the detailed analysis for this scenario is beyond the scope of this paper.

## SM5. WHY OUR SECURITY PROOF DOES NOT REQUIRE THE SEQUENTIAL ASSUMPTION

In this Section, we explain why the RT [S2] (see also [S1]) requires the QKD protocol to be run sequentially, which restricts its repetition rate, and why our analysis does not need this requirement. As discussed before, the aim of these security proofs is to estimate the phase-error rate. To do so, the RT considers an entanglement-based version of the Virtual Protocol in which Alice and Bob measure their respective systems one by one. The probability that Alice obtains  $l \in \{\text{vir}0, \text{vir}1, 0_Z, 1_Z, 0_X\}$  and Bob obtains  $\beta_X \in \{0_X, 1_X\}$  in the  $k$ -th round, conditioned on the outcomes  $\vec{v}_{k-1}$  of their previous  $k-1$  measurements, can be expressed as

$$\Pr[v_k = (l, \beta_X) | \vec{v}_{k-1}] = p_l \text{Tr} [|\psi_l\rangle\langle\psi_l| \hat{M}_{\beta_X}^{\vec{v}_{k-1}}], \quad (\text{S211})$$

where  $p_l$  is defined in Eq. (S91) and the operators  $\hat{M}_{\beta_X}^{\vec{v}_{k-1}} \geq 0$  depend on Eve's attack and on the previous measurement outcomes. Note that, for simplicity, we have implicitly assumed a three-state P&M protocol, but our discussion also applies to other P&M and MDI-type scenarios. The probability to obtain a phase error in the  $k$ -th round is then

$$\Pr[v_k = (\text{vir}0, 1_X) | \vec{v}_{k-1}] + \Pr[v_k = (\text{vir}1, 0_X) | \vec{v}_{k-1}]. \quad (\text{S212})$$

To derive a bound on this quantity, the RT employs a Cauchy-Schwarz type inequality that requires the operators  $\hat{M}_{\beta_X}^{\vec{v}_{k-1}}$  to satisfy  $\hat{M}_{\beta_X}^{\vec{v}_{k-1}} \leq \hat{\mathbb{I}}$ , which does not necessarily hold when Eve can correlate Bob's measurement outcomes on the rounds  $\{1, \dots, k-1\}$  with Alice's setting choice on round  $k$ . For example, let us suppose that Eve simply performs a SWAP gate between the photonic systems of the first and second rounds, and that Alice obtains  $l = 0_X$  and Bob obtains  $0_X$  in the first round. Because of the SWAP gate, the fact that Bob obtained  $0_X$  in the first round makes it more likely that Alice will obtain  $l = 0_X$  in the second round, and the fact that Alice obtained  $l = 0_X$  in the first round makes it almost certain that Bob will obtain  $0_X$  in the second round. Because of this, we may have that

$$\Pr[v_2 = (0_X, 0_X) | v_1 = (0_X, 0_X)] > p_{0_X}, \quad (\text{S213})$$

or equivalently,

$$\text{Tr} [ |\psi_{0_x}\rangle\langle\psi_{0_x}| \hat{M}_{0_x}^{v_1} ] > 1, \quad (\text{S214})$$

implying that  $\hat{M}_{0_x}^{v_1} \not\leq \hat{\mathbb{I}}$ .

The condition  $\hat{M}_{\beta_x}^{\bar{v}_{k-1}} \leq \hat{\mathbb{I}}$  is guaranteed to hold if Eve's attack is sequential (see Appendix D in [S20] for more details), rather than fully general, i.e., when it can be described as a sequence of  $N$  unitary operators, each acting on a single photonic system and on Eve's updated ancilla, see Fig. S10. In practice, to ensure that Eve's attack is sequential, the users need to run the protocol at a restricted repetition rate, as discussed in detail below. On the other hand, the security proof presented in this work is based on the quantum coin inequality in Eq. (S38), which does not require the sequential assumption, and thus does not impose any restriction on the repetition rate of the system. The key result used to derive this inequality is Eq. (S219), which holds even if Eve performs a fully general attack, because it merely uses the fact that the quantum coin is a qubit, i.e., a two-level system.

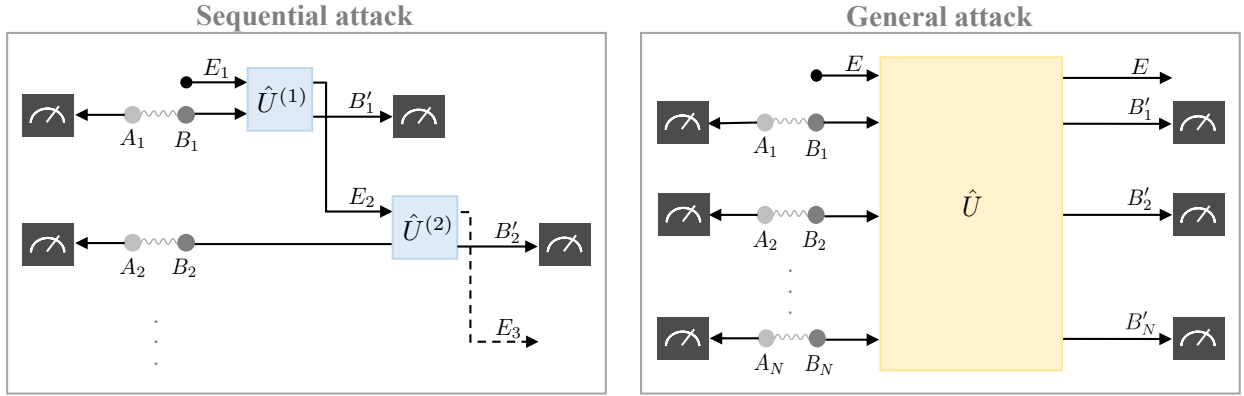

Figure S10. Diagram of the entanglement-based version of the protocol when Eve performs a sequential attack and a general attack. In the most general case, Eve can interact with all systems  $B_1 \dots B_N$  at the same time. However, in the sequential case, Eve must act on system  $B_k$  before she has access to system  $B_{k+1}$ . A sequential attack can be seen as an intermediate step between a collective attack and a general attack. More precisely, a collective attack is a special case of a sequential attack in which Alice and Bob's measurement results are guaranteed to be independent and identically distributed for different rounds of the protocol.

We note that the LT analysis [S14], which considered the case in which the emitted states are qubit states (i.e.,  $\epsilon = 0$ ), does not need the sequential assumption either. In the LT analysis, we first establish a relationship among probabilities of the form of Eq. (S211) by using a relationship between the qubit states, see Eqs. (S14) and (S15). Since this relationship between the states is linear thanks to the qubit structure, the relationship among the probabilities is also linear. Noting that this linear relationship holds even if  $\hat{M}_{\beta_x}^{\bar{v}_{k-1}} \not\leq \hat{\mathbb{I}}$  and also recalling that just by taking the sum over the probabilities and applying Azuma's or Kato's inequality we can obtain a bound on the number of phase errors, we conclude that the LT analysis does not require the sequential assumption.

#### A. Ensuring sequentiality by restricting the repetition rate

To ensure that Eve's attack is sequential, Alice and Bob need to prevent the possibility of any signalling from Alice's  $k$ -th pulse to Bob's  $(k-1)$ -th measurement result. The easiest way to achieve this is for Alice to only emit the  $k$ -th pulse after Bob has performed his  $(k-1)$ -th measurement [S20]. Let  $l_{\text{fib}}$  be the length of the fibre separating Alice and Bob,  $r$  be its refractive index, and  $c$  be the speed of light in a vacuum. Alice's photons travel through the fibre at a speed of  $c/r$ , and therefore they take a time of  $rl_{\text{fib}}/c$  to reach Bob. If Alice sends her first pulse at time  $t_1^A = 0$ , then Bob will measure it at a time not earlier than  $t_1^B = rl_{\text{fib}}/c$ . Therefore, the earliest time that Alice could send the second pulse is  $t_2^A = t_1^B = rl_{\text{fib}}/c$ . More generally, Alice needs to separate all her pulses by at least  $t_\Delta^A = rl_{\text{fib}}/c$ , and her repetition rate should be at most

$$f_{\text{max}} = \frac{1}{t_\Delta^A} = \frac{c}{rl_{\text{fib}}}. \quad (\text{S215})$$

In Fig. 2 of the Main Text, we have computed the key rate for the RT under this constraint; more specifically, we have assumed a repetition rate of  $\min(f_{\max}, 2.5 \text{ GHz})$ . For example, if  $r = 1.5$  and  $l_{\text{fib}} = 100 \text{ km}$ , we have that  $f_{\max} = 2 \text{ kHz}$ .

A recent work [S51] has suggested that, to achieve sequentiality, it may be enough to ensure that Bob's  $(k-1)$ -th measurement is outside the future light cone of Alice's  $k$ -th pulse emission. This takes into account the fact that, irrespectively of Eve's action, information about Alice's pulse cannot travel faster than  $c$  to Bob's measurement setup. Let  $l_{\text{act}}$  be the actual physical distance separating Alice and Bob, which must be such that  $l_{\text{act}} \leq l_{\text{fib}}$ , with equality if and only if the fibre is laid out in a straight line. Since information about Alice's pulse must take at least  $l_{\text{act}}/c$  to reach Bob, to ensure that her second pulse cannot possibly affect Bob's first measurement result, Alice needs to emit it at a time not earlier than

$$t_2^A = t_1^B - \frac{l_{\text{act}}}{c} = \frac{rl_{\text{fib}}}{c} - \frac{l_{\text{act}}}{c} = \frac{rl_{\text{fib}} - l_{\text{act}}}{c}, \quad (\text{S216})$$

and more generally, Alice needs to separate her pulses by at least  $t_\Delta^A = t_2^A$ . In other words, her repetition rate can be at most

$$f'_{\max} = \frac{1}{t_\Delta^A} = \frac{c}{rl_{\text{fib}} - l_{\text{act}}}. \quad (\text{S217})$$

Assuming again a standard fibre of  $r = 1.5$ , we have that  $f'_{\max}$  is three times larger than  $f_{\max}$  when  $l_{\text{act}} = l_{\text{fib}}$ , and less than that when  $l_{\text{act}} < l_{\text{fib}}$ . For example, assuming that  $l_{\text{act}} = l_{\text{fib}} = 100 \text{ km}$ , we have that  $f'_{\max} = 3f_{\max} = 6 \text{ kHz}$ , which is still a considerable restriction on the repetition rate. Because of this, our security proof can achieve significantly higher key rates per second than the RT even if one uses this relaxed relativistic constraint, as shown in Fig. S11.

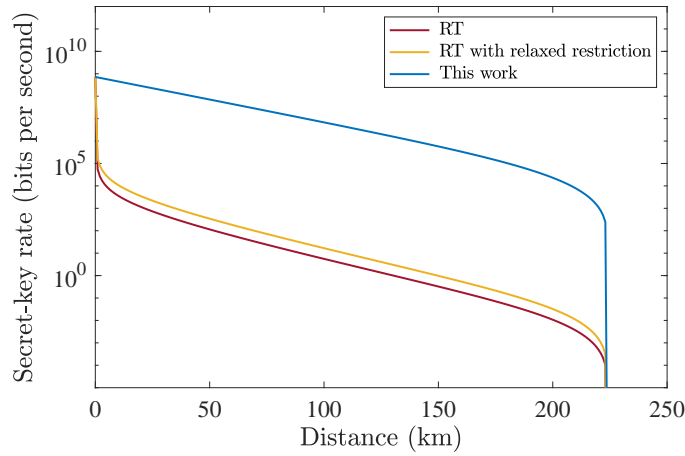

Figure S11. Secret-key rate achievable by the reference technique (RT) with the restriction that Alice emits each pulse after Bob has measured the previous pulse (red line), and with the restriction that Alice emits her pulses such that they could not have affected Bob's previous measurement result, based on relativistic arguments (yellow line); compared with that achievable by our security proof. We assume that the fibre connecting Alice and Bob is in a straight line ( $l_{\text{act}} = l_{\text{fib}}$ ) and that its refractive index is  $r = 1.5$ . Moreover, for our security proof, we assume a repetition rate of  $2.5 \text{ GHz}$ , and for the RT curves, we assume repetition rates of  $\min(f_{\max}, 2.5 \text{ GHz})$  and  $\min(f'_{\max}, 2.5 \text{ GHz})$ , respectively. Also, we consider the BB84 protocol, and the values  $\delta = 0.063$  and  $\epsilon = 10^{-6}$ .

We note that, in the discussion above, we have assumed a P&M protocol, in which Alice and Bob can ensure that the sequential condition has been met by comparing their timestamps at the end of the protocol. In MDI-type [S7] setups, ensuring the sequential condition seems much harder because Alice and Bob cannot trust Charlie's timestamps. Therefore, they would likely have to wait until they receive Charlie's outcome announcement for the  $(k-1)$ -th round before emitting their  $k$ -th pulse, which would impose even harsher restrictions on the repetition rate.

## SM6. RECIPE FOR EXPERIMENTALISTS

Here, we provide a step-by-step example of the application of our security analysis to an actual finite-key QKD implementation. For this, we have chosen the coherent-light-based MDI scheme [S34] analyzed in Section SM4 A,

for two main reasons: (1) its practical implementation using laser sources, and (2) the fact that for this scheme, our security proof can directly protect both Alice’s and Bob’s sources against any practical imperfection, including those associated to the light source itself, such as intensity fluctuations and correlations, achieving a very high level of implementation security. Still, we remark that this recipe would look fairly similar for other protocols to which our analysis is applicable, such as BB84, the three-state protocol or standard MDI-QKD.

The scheme is depicted in Fig. S6 and its protocol description is given in Section SM4 A. For each round, Alice and Bob attempt to generate a state in the set  $\{|\sqrt{\mu}\rangle, |-\sqrt{\mu}\rangle, |\text{vac}\rangle\}$  and send it to an untrusted middle node Charlie, who performs an interference measurement and announces the result. We refer to the coherent states  $|\pm\sqrt{\mu}\rangle$  as the  $Z$ -basis states, and these are used both for key generation and parameter estimation. The vacuum state  $|\text{vac}\rangle$  is only used for parameter estimation, and we refer to it as the  $X$ -basis state. To apply our analysis, one should follow these steps:

### 1. Specification of Security Parameters:

- Decide the total number of emitted rounds,  $N$ .
- Specify the correctness and secrecy parameters of the final key,  $\epsilon_{\text{corr}}$  and  $\epsilon_{\text{secr}}$ .
- Specify the failure probabilities for the application of each concentration inequality— $\epsilon_C$  for the Chernoff bound,  $\epsilon_H$  for Hoeffding’s inequality, and  $\epsilon_A$  for Azuma’s inequality—; and the privacy amplification parameter  $\epsilon_{\text{PA}}$ . These should be chosen such that  $\epsilon_{\text{secr}} = \sqrt{2}\sqrt{\epsilon_{\text{tot}} + \epsilon_{\text{PA}}}$ , where  $\epsilon_{\text{tot}} := 6\epsilon_A + 31\epsilon_C + \epsilon_H$  is the total failure probability of the phase-error rate estimation process.
- Specify the probability that each user emits a coherent state (rather than a vacuum state),  $p_Z$ ; the probability that a detected event in which both users emitted a coherent state is used for key generation (rather than parameter estimation),  $p_{\text{key}|Z}$ ; and a fictitious probability that does not refer to any action performed in the actual protocol (but does have an effect in the parameter estimation analysis),  $p_{Z_C}$ .

To select the parameters in the last two bullet points, one option would be simulate many runs of the protocol using different parameter combinations, and then choose the values that result in the highest secret-key rate. Another option would be to just give them some values, such as, e.g.,  $\epsilon_{\text{tot}} = \epsilon_{\text{PA}} = \epsilon_{\text{sec}}^2/4$ ,  $\epsilon_A = \epsilon_C = \epsilon_H = \epsilon_{\text{tot}}/38$ , and  $p_Z = p_{\text{key}|Z} = p_{Z_C} = 0.7$ .

### 2. State Characterization:

- Partially characterize Alice and Bob’s sources, to ensure that the states they emit,  $\{|\psi_{0Z}\rangle, |\psi_{1Z}\rangle, |\psi_{0X}\rangle\}$ , are  $\epsilon$ -close (in terms of fidelity) to the states  $\{|\sqrt{\mu}\rangle, |-\sqrt{\mu}\rangle, |\text{vac}\rangle\}$ .

### 3. Bound on Coin Imbalance Parameter:

- Obtain an upper bound on the coin imbalance parameter  $\Delta$  using the procedure laid out in Section SE2 B.

### 4. Quantum Communication:

- Execute the quantum communication phase of the protocol, obtaining a sifted key pair and the value of the observables  $N_{ij}^{\text{det}}$ ,  $N_{\text{key}}^{\text{det}}$  and  $N^{\text{det}}$  (see protocol description in Section SM4 A).
- Substitute these values into Eqs. (S197) to (S199) to obtain an upper bound on the number of phase errors  $N_{\text{ph}}$ .

### 5. Error Correction and Verification:

Implement the error correction and error verification processes to ensure the  $\epsilon_{\text{corr}}$ -correctness of the sifted key.

### 6. Privacy Amplification:

Apply privacy amplification to obtain a secure key pair of length  $N_{\text{sec}}$ , given by Eq. (S153).

After following Steps 1–6 above, the final key pair obtained is guaranteed to be  $(\epsilon_{\text{corr}} + \epsilon_{\text{secr}})$ -secure.

## Supplementary Equations

In the Supplementary Equations, we first prove the quantum coin inequality, which is used to derive an upper bound on the number of phase errors  $N_{\text{ph}}$ . After, in Section SE2, we show how to obtain  $\Delta$  in Eq. (S41) using numerical techniques based on SDP and then, using analytical techniques with an additional assumption. Then, in Section SE3, we explain the channel model used to simulate the results for the P&M protocols and for the coherent-light-based MDI protocol considered, and list the respective equations. Finally, in Section SE4, we give a high-level description of the code used to generate the figures in this work.

### SE1. PROOF OF THE QUANTUM COIN INEQUALITY

#### A. Prepare-and-measure scenario

Here, we prove the quantum coin inequality in Eq. (S38). To do so, we consider that Alice and Bob run the following scenario, which is equivalent to the Coin Protocol defined in Section SM1 B 4.

1. Alice prepares  $N$  copies of the state

$$|\Psi\rangle_{TC DAB} = \sqrt{p_C} |0\rangle_T |\Psi_{\text{coin}}\rangle_{C DAB} + \sqrt{1 - p_C} |1\rangle_T |0\rangle_C |0\rangle_D |\rho_{\text{comp}}\rangle_{AB}, \quad (\text{S218})$$

where  $|\rho_{\text{comp}}\rangle_{AB}$  is a purification of  $\rho_{\text{comp}}$ , and sends all photonic systems  $B$  through a quantum channel.

2. For each round, Bob performs the quantum nondemolition measurement  $\{\hat{m}_{\text{det}}, \hat{m}_f\}$ , and if he obtains a successful detection, he announces this. Let  $\mathcal{N}^{\text{det}}$  be the set of detected rounds.
3. For each round  $k \in \mathcal{N}^{\text{det}}$  (i.e., each detected round), Alice measures system  $T$  in the computational basis, learning if the round is a coin round ( $T = 0$ ) or a compensation round ( $T = 1$ ). Also, if  $T = 0$ , Alice and Bob perform the POVM  $\{\hat{m}_{\text{err}}, \hat{\mathbb{I}} - \hat{m}_{\text{err}}\}$ , and denote by  $m$  ( $\bar{m}$ ) the outcome associated to  $\hat{m}_{\text{err}}$  ( $\hat{\mathbb{I}} - \hat{m}_{\text{err}}$ ). Then, Alice chooses  $Z_C$  ( $X_C$ ) with probability  $p_{Z_C}$  ( $p_{X_C}$ ) and measures the coin system  $C$  in the selected basis.
4. For each round not in  $\mathcal{N}^{\text{det}}$ , Alice measures system  $T$  in the computational basis. If  $T = 0$ , Alice chooses  $Z_C$  ( $X_C$ ) with probability  $p_{Z_C}$  ( $p_{X_C}$ ) and measures the coin system  $C$  in the selected basis.

We are interested in Alice and Bob's measurements in Step 3 above. In particular, let us consider the state of the systems corresponding to the  $k$ -th round in  $\mathcal{N}^{\text{det}}$  conditioned on Alice and Bob having obtained some overall outcome  $\vec{v}_{k-1}$  for the previous  $k - 1$  detected rounds, and having obtained the outcomes  $T = 0$  and  $m$  for the  $k$ -th round but having not yet measured the  $k$ -th coin system  $C$ . Due to Eve's general attack and the conditioning on Alice and Bob's previous measurement results, the reduced state of the  $k$ -th system  $C$  will no longer be  $\text{Tr}_{DAB}[|\Psi_{\text{coin}}\rangle\langle\Psi_{\text{coin}}|_{C DAB}]$ . However, no operation has acted on this system, and its reduced state is still in the qubit space spanned by  $\{|0_Z\rangle_C, |1_Z\rangle_C\}$ . Because of this, and using the fact that the length of its Bloch vector cannot exceed 1, we can derive the following inequality [S22]

$$1 - 2P^{(k)}(X_C = 1|X_C, T = 0, m, \vec{v}_{k-1}) \leq 2\sqrt{P^{(k)}(Z_C = 0|Z_C, T = 0, m, \vec{v}_{k-1})P^{(k)}(Z_C = 1|Z_C, T = 0, m, \vec{v}_{k-1})}. \quad (\text{S219})$$

Here,  $P^{(k)}(Z_C = 0|Z_C, T = 0, m, \vec{v}_{k-1})$  refers to the probability that, in the  $k$ -th round in  $\mathcal{N}^{\text{det}}$ , Alice obtains the measurement outcome  $Z_C = 0$ , conditional on having obtained the outcomes  $T = 0$  and  $m$ , on having chosen the  $Z_C$  basis to measure the coin system for this round, and on having obtained some overall measurement result  $\vec{v}_{k-1}$  for the previous  $k - 1$  detected rounds. The rest of the probabilities in Eq. (S219) are defined analogously. Note that, when the symbols  $Z_C$  or  $X_C$  appear by themselves inside these probabilities, they refer to the selection of the  $Z_C$  or  $X_C$  basis to measure system  $C$ . However, when they appear together with an equals sign, such as  $Z_C = 0$ , it refers to the outcome of this measurement.

On the other hand, we have that

$$\begin{aligned}
& P^{(k)}(T = 0, m|\vec{v}_{k-1})P^{(k)}(X_C = 1|X_C, T = 0, m, \vec{v}_{k-1}) \\
&= P^{(k)}(T = 0, m|\vec{v}_{k-1}) \frac{P^{(k)}(X_C = 1, X_C, T = 0, m|\vec{v}_{k-1})}{P^{(k)}(X_C, T = 0, m|\vec{v}_{k-1})} \\
&= P^{(k)}(T = 0, m|\vec{v}_{k-1}) \frac{P^{(k)}(X_C = 1, X_C, T = 0, m|\vec{v}_{k-1})}{P^{(k)}(X_C|T = 0, m, \vec{v}_{k-1})P^{(k)}(T = 0, m|\vec{v}_{k-1})} \\
&= P^{(k)}(T = 0, m|\vec{v}_{k-1}) \frac{P^{(k)}(X_C = 1, X_C, T = 0, m|\vec{v}_{k-1})}{p_{X_C}P^{(k)}(T = 0, m|\vec{v}_{k-1})} \\
&= \frac{P^{(k)}(X_C = 1, X_C, T = 0, m|\vec{v}_{k-1})}{p_{X_C}},
\end{aligned} \tag{S220}$$

where in the third equality we have used the fact that, in a coin round (i.e., a round with an outcome  $T = 0$ ), the probability to select the  $X_C$  basis is independent of obtaining the outcome  $m$ , and equal to  $p_{X_C}$ . In a similar way, we have that

$$\begin{aligned}
& P^{(k)}(T = 0, m|\vec{v}_{k-1})P^{(k)}(Z_C = 0|Z_C, T = 0, m, \vec{v}_{k-1}) = \frac{P^{(k)}(Z_C = 0, Z_C, T = 0, m|\vec{v}_{k-1})}{p_{Z_C}}, \\
& P^{(k)}(T = 0, m|\vec{v}_{k-1})P^{(k)}(Z_C = 1|Z_C, T = 0, m, \vec{v}_{k-1}) = \frac{P^{(k)}(Z_C = 1, Z_C, T = 0, m|\vec{v}_{k-1})}{p_{Z_C}}.
\end{aligned} \tag{S221}$$

Multiplying by  $P^{(k)}(T = 0, m|\vec{v}_{k-1})$  on both sides of Eq. (S219), and using Eqs. (S220) and (S221) we obtain

$$\begin{aligned}
& P^{(k)}(T = 0, m|\vec{v}_{k-1}) - 2 \frac{P^{(k)}(X_C = 1, X_C, T = 0, m|\vec{v}_{k-1})}{p_{X_C}} \\
& \leq \frac{2}{p_{Z_C}} \sqrt{P^{(k)}(Z_C = 0, Z_C, T = 0, m|\vec{v}_{k-1})P^{(k)}(Z_C = 1, Z_C, T = 0, m|\vec{v}_{k-1})}.
\end{aligned} \tag{S222}$$

Replacing  $m$  by  $\bar{m}$  in Eqs. (S219) to (S222), we obtain

$$\begin{aligned}
& P^{(k)}(T = 0, \bar{m}|\vec{v}_{k-1}) - 2 \frac{P^{(k)}(X_C = 1, X_C, T = 0, \bar{m}|\vec{v}_{k-1})}{p_{X_C}} \\
& \leq \frac{2}{p_{Z_C}} \sqrt{P^{(k)}(Z_C = 0, Z_C, T = 0, \bar{m}|\vec{v}_{k-1})P^{(k)}(Z_C = 1, Z_C, T = 0, \bar{m}|\vec{v}_{k-1})} \\
& = \frac{2}{p_{Z_C}} \sqrt{P^{(k)}(Z_C = 0, Z_C, T = 0|\vec{v}_{k-1}) - P^{(k)}(Z_C = 0, Z_C, T = 0, m|\vec{v}_{k-1})} \\
& \quad \times \sqrt{P^{(k)}(Z_C = 1, Z_C, T = 0|\vec{v}_{k-1}) - P^{(k)}(Z_C = 1, Z_C, T = 0, m|\vec{v}_{k-1})}.
\end{aligned} \tag{S223}$$

Taking the sum of Eqs. (S222) and (S223), we obtain

$$\begin{aligned}
& P^{(k)}(T = 0|\vec{v}_{k-1}) - 2 \frac{P^{(k)}(X_C = 1, X_C, T = 0|\vec{v}_{k-1})}{p_{X_C}} \\
& \leq \frac{2}{p_{Z_C}} \left( \sqrt{P^{(k)}(Z_C = 0, Z_C, T = 0, m|\vec{v}_{k-1})P^{(k)}(Z_C = 1, Z_C, T = 0, m|\vec{v}_{k-1})} \right. \\
& \quad + \sqrt{P^{(k)}(Z_C = 0, Z_C, T = 0|\vec{v}_{k-1}) - P^{(k)}(Z_C = 0, Z_C, T = 0, m|\vec{v}_{k-1})} \\
& \quad \times \sqrt{P^{(k)}(Z_C = 1, Z_C, T = 0|\vec{v}_{k-1}) - P^{(k)}(Z_C = 1, Z_C, T = 0, m|\vec{v}_{k-1})} \Big).
\end{aligned} \tag{S224}$$

Also, we have that,

$$P^{(k)}(T = 0|\vec{v}_{k-1}) = \frac{P^{(k)}(T = 0|\vec{v}_{k-1})p_{Z_C}}{p_{Z_C}} = \frac{P^{(k)}(T = 0|\vec{v}_{k-1})P(Z_C|T = 0, \vec{v}_{k-1})}{p_{Z_C}} = \frac{P^{(k)}(Z_C, T = 0|\vec{v}_{k-1})}{p_{Z_C}}. \tag{S225}$$

Substituting Eq. (S225) into Eq. (S224), taking the sum over all rounds  $k \in \mathcal{N}^{\text{det}}$  on both sides of the inequality, and using the fact that  $\sqrt{xy}$  is a convex function of both  $x$  and  $y$ , we obtain

$$\begin{aligned}
& \frac{\sum_k P^{(k)}(Z_C, T=0|\vec{v}_{k-1})}{p_{Z_C}} - 2 \frac{\sum_k P^{(k)}(X_C=1, X_C, T=0|\vec{v}_{k-1})}{p_{X_C}} \\
& \leq \frac{2}{p_{Z_C}} \left( \sqrt{\sum_k P^{(k)}(Z_C=0, Z_C, T=0, m|\vec{v}_{k-1}) \sum_k P^{(k)}(Z_C=1, Z_C, T=0, m|\vec{v}_{k-1})} \right. \\
& \quad \left. + \sqrt{\sum_k P^{(k)}(Z_C=0, Z_C, T=0|\vec{v}_{k-1}) - \sum_k P^{(k)}(Z_C=0, Z_C, T=0, m|\vec{v}_{k-1})} \right. \\
& \quad \left. \times \sqrt{\sum_k P^{(k)}(Z_C=1, Z_C, T=0|\vec{v}_{k-1}) - \sum_k P^{(k)}(Z_C=1, Z_C, T=0, m|\vec{v}_{k-1})} \right). \tag{S226}
\end{aligned}$$

Now, let us rewrite Eq. (S226) as

$$\frac{\tilde{N}_{Z_C}^{\text{det}}}{p_{Z_C}} - \frac{2\tilde{N}_{X_C=1}^{\text{det}}}{p_{X_C}} \leq \frac{2}{p_{Z_C}} \left[ \sqrt{\tilde{N}_{Z_C=0}^{\text{err}} \tilde{N}_{Z_C=1}^{\text{err}}} + \sqrt{(\tilde{N}_{Z_C=0}^{\text{det}} - \tilde{N}_{Z_C=0}^{\text{err}})(\tilde{N}_{Z_C=1}^{\text{det}} - \tilde{N}_{Z_C=1}^{\text{err}})} \right], \tag{S227}$$

where we have defined  $\tilde{N}_{Z_C}^{\text{det}} := \sum_k P^{(k)}(Z_C, T=0|\vec{v}_{k-1})$ ,  $\tilde{N}_{X_C=1}^{\text{det}} := \sum_k P^{(k)}(X_C=1, X_C, T=0|\vec{v}_{k-1})$ ,  $\tilde{N}_{Z_C=x}^{\text{err}} := \sum_k P^{(k)}(Z_C=x, Z_C, T=0, m|\vec{v}_{k-1})$  and  $\tilde{N}_{Z_C=x}^{\text{det}} := \sum_k P^{(k)}(Z_C=x, Z_C, T=0|\vec{v}_{k-1})$ . Then, dividing by  $\tilde{N}_{Z_C}^{\text{det}}$  on both sides and using the fact that  $\tilde{N}_{Z_C}^{\text{det}} = \tilde{N}_{Z_C=0}^{\text{det}} + \tilde{N}_{Z_C=1}^{\text{det}} \geq 2\sqrt{\tilde{N}_{Z_C=0}^{\text{det}} \tilde{N}_{Z_C=1}^{\text{det}}}$ , we obtain

$$\begin{aligned}
1 - \frac{2p_{Z_C} \tilde{N}_{X_C=1}^{\text{det}}}{p_{X_C} \tilde{N}_{Z_C}^{\text{det}}} & \leq \frac{1}{\sqrt{\tilde{N}_{Z_C=0}^{\text{det}} \tilde{N}_{Z_C=1}^{\text{det}}}} \left[ \sqrt{\tilde{N}_{Z_C=0}^{\text{err}} \tilde{N}_{Z_C=1}^{\text{err}}} + \sqrt{(\tilde{N}_{Z_C=0}^{\text{det}} - \tilde{N}_{Z_C=0}^{\text{err}})(\tilde{N}_{Z_C=1}^{\text{det}} - \tilde{N}_{Z_C=1}^{\text{err}})} \right] \\
& = \sqrt{\frac{\tilde{N}_{Z_C=0}^{\text{err}}}{\tilde{N}_{Z_C=0}^{\text{det}}} \frac{\tilde{N}_{Z_C=1}^{\text{err}}}{\tilde{N}_{Z_C=1}^{\text{det}}}} + \sqrt{\left(1 - \frac{\tilde{N}_{Z_C=0}^{\text{err}}}{\tilde{N}_{Z_C=0}^{\text{det}}}\right) \left(1 - \frac{\tilde{N}_{Z_C=1}^{\text{err}}}{\tilde{N}_{Z_C=1}^{\text{det}}}\right)}. \tag{S228}
\end{aligned}$$

The inequality  $z \leq \sqrt{y'y} + \sqrt{1-y'}\sqrt{1-y}$ , with  $z, y, y' \in [0, 1]$ , is equivalent to the inequality  $G_-(y, z) \leq y' \leq G_+(y, z)$ , where [S2]

$$G_-(y, z) = \begin{cases} g_-(y, z) & \text{if } y > 1 - z^2 \\ 0 & \text{otherwise} \end{cases} \quad \text{and} \quad G_+(y, z) = \begin{cases} g_+(y, z) & \text{if } y < z^2 \\ 1 & \text{otherwise,} \end{cases} \tag{S229}$$

and

$$g_{\pm}(y, z) = y + (1 - z^2)(1 - 2y) \pm 2\sqrt{z^2(1 - z^2)y(1 - y)}. \tag{S230}$$

Therefore, Eq. (S228) implies that

$$\frac{\tilde{N}_{Z_C=0}^{\text{err}}}{\tilde{N}_{Z_C=0}^{\text{det}}} \leq G_+\left(\frac{\tilde{N}_{Z_C=1}^{\text{err}}}{\tilde{N}_{Z_C=1}^{\text{det}}}, 1 - \frac{2p_{Z_C} \tilde{N}_{X_C=1}^{\text{det}}}{p_{X_C} \tilde{N}_{Z_C}^{\text{det}}}\right). \tag{S231}$$

Then, by rearranging and applying Azuma's inequality (see Section SM1 E 1 for more details), we have that

$$N_{Z_C=0}^{\text{err}} - \Delta_A \leq_{6\epsilon_A} (N_{Z_C=0}^{\text{det}} + \Delta_A) G_+\left(\frac{N_{Z_C=1}^{\text{err}} + \Delta_A}{N_{Z_C=1}^{\text{det}} - \Delta_A}, 1 - \frac{2p_{Z_C} (N_{X_C=1}^{\text{det}} + \Delta_A)}{p_{X_C} (N_{Z_C}^{\text{det}} - \Delta_A)}\right), \tag{S232}$$

where we have used the fact that  $G_+(y, z) \leq G_+(\bar{y}, \bar{z})$  with  $\bar{y} \geq y$  and  $\bar{z} \leq z$ . In Eq. (S232),  $\Delta_A := \Delta_A(N^{\text{det}}) = \sqrt{2N^{\text{det}} \ln 1/\epsilon_A}$  where  $N^{\text{det}} = |\mathcal{N}^{\text{det}}|$  is the total number of detected rounds;  $N_{X_C=1}^{\text{det}}$  is the total number of detected coin events in which Alice selected the  $X_C$  basis and obtained  $X_C=1$ ;  $N_{Z_C}^{\text{det}} := N_{Z_C=0}^{\text{det}} + N_{Z_C=1}^{\text{det}}$  is the total number of detected coin rounds in which Alice chose the  $Z_C$  basis; and  $N_{Z_C=0}^{\text{err}}$ ,  $N_{Z_C=1}^{\text{err}}$ ,  $N_{Z_C=0}^{\text{det}}$  and  $N_{Z_C=1}^{\text{det}}$  are defined in Section SM1 B 4. Note that, since we started the analysis by assuming that Bob had obtained a particular set of

detections  $\mathcal{N}_{\text{det}}$ , our formula in Eq. (S232) appears to be a statistical statement conditional on this particular set  $\mathcal{N}_{\text{det}}$ , i.e., a shorthand for a statement of the form  $\Pr[L > R | \mathcal{N}_{\text{det}}] \leq 6\epsilon_A$ . However, since we have shown that this statement holds for any  $\mathcal{N}_{\text{det}}$ , we can remove the conditioning on  $\mathcal{N}_{\text{det}}$ , i.e., we simply have that  $\Pr[L > R] \leq 6\epsilon_A$ . Finally, using the fact that  $N_{X_C=1}^{\text{det}} \leq N_{X_C=1}$ , where  $N_{X_C=1}$  is the total number of coin events in which Alice selected the  $X_C$  basis and obtained  $X_C = 1$  (detected or not), we obtain

$$N_{Z_C=0}^{\text{err}} - \Delta_A \leq \frac{N_{Z_C=0}^{\text{det}} + \Delta_A}{6\epsilon_A} G_+ \left( \frac{N_{Z_C=1}^{\text{err}} + \Delta_A}{N_{Z_C=1}^{\text{det}} - \Delta_A}, 1 - \frac{2p_{Z_C}(N_{X_C=1} + \Delta_A)}{p_{X_C}(N_{Z_C}^{\text{det}} - \Delta_A)} \right). \quad (\text{S233})$$

We remark that a similar expression to Eq. (S233) can be obtained by applying Kato's inequality [S25] instead of Azuma's inequality, resulting in a tighter estimation of  $N_{Z_C=0}^{\text{err}}$  (see Section SM1 E).

In the asymptotic regime ( $N \rightarrow \infty$ ), Eq. (S233) becomes

$$N_{Z_C=0}^{\text{err}} \lesssim N_{Z_C=0}^{\text{det}} G_+ \left( \frac{N_{Z_C=1}^{\text{err}}}{N_{Z_C=1}^{\text{det}}}, 1 - \frac{2p_{Z_C} N_{X_C=1}}{p_{X_C} N_{Z_C}^{\text{det}}} \right). \quad (\text{S234})$$

By substituting  $N_{Z_C}^{\text{det}} := N_{Z_C=0}^{\text{det}} + N_{Z_C=1}^{\text{det}}$  in Eq. (S234), we obtain the quantum coin inequality in Eq. (S38), as desired.

## B. Measurement-device-independent scenario

For MDI-type schemes, the quantum coin inequality can be derived in a similar way as for the P&M case. For this, we first define a Coin Protocol as follows.

1. Alice and Bob prepare  $N$  copies of the state

$$|\Psi\rangle_{TC DAB} = \sqrt{p_C} |0\rangle_T |\Psi_{\text{coin}}\rangle_{C DAB} + \sqrt{1-p_C} |1\rangle_T |0\rangle_C |0\rangle_D |\rho_{\text{comp}}\rangle_{AB}, \quad (\text{S235})$$

where  $p_C = 2p_{\text{Tar}}$  and  $|\rho_{\text{comp}}\rangle_{AB}$  is a purification of  $\rho_{\text{comp}}$ . Then, they send all photonic systems  $B$  to Charlie through a quantum channel.

2. For each round, Charlie performs a measurement and announces whether the round was detected. Let  $\mathcal{N}^{\text{det}}$  be the set of detected rounds.
3. For each round  $k \in \mathcal{N}^{\text{det}}$  (i.e., each detected round), Alice and Bob measure system  $T$  in the computational basis, learning if the round is a coin round ( $T = 0$ ) or a compensation round ( $T = 1$ ). Also, if  $T = 0$ , Alice and Bob perform the POVM  $\{\hat{m}_{\text{err}}, \hat{\mathbb{I}} - \hat{m}_{\text{err}}\}$ , where  $\hat{m}_{\text{err}} = |0\rangle\langle 0|_{D_a} \otimes |0\rangle\langle 0|_{D_b} + |1\rangle\langle 1|_{D_a} \otimes |1\rangle\langle 1|_{D_b}$ , and denote by  $m$  ( $\bar{m}$ ) the outcome associated to  $\hat{m}_{\text{err}}$  ( $\hat{\mathbb{I}} - \hat{m}_{\text{err}}$ ). Then, Alice and Bob choose  $Z_C$  ( $X_C$ ) with probability  $p_{Z_C}$  ( $p_{X_C}$ ) and measure the coin system  $C$  in the selected basis.
4. For each round not in  $\mathcal{N}^{\text{det}}$ , Alice and Bob measure system  $T$  in the computational basis. If  $T = 0$ , Alice and Bob choose  $Z_C$  ( $X_C$ ) with probability  $p_{Z_C}$  ( $p_{X_C}$ ) and measure the coin system  $C$  in the selected basis.

Then, by following the steps from Eq. (S219) to (S234), we obtain

$$N_{Z_C=0}^{\text{err}} \lesssim N_{Z_C=0}^{\text{det}} G_+ \left( \frac{N_{Z_C=1}^{\text{err}}}{N_{Z_C=1}^{\text{det}}}, 1 - \frac{2p_{Z_C} N_{X_C=1}}{p_{X_C} N_{Z_C}^{\text{det}}} \right). \quad (\text{S236})$$

## SE2. OBTAINING A BOUND ON THE COIN IMBALANCE PARAMETER $\Delta$

In this Section, we show how to obtain a bound on the coin imbalance parameter  $\Delta := 1 - \text{Re} \langle \Psi_{\text{Ref}} | \Psi_{\text{Tar}} \rangle_{DAB}$ , which incorporates the effect of the side channels in our security proof. For concreteness, we focus on the three-state protocol considered in Section SM1 B and on the coherent-light-based MDI protocol considered in Section SM4 A. However, the methods introduced here can be easily adapted to other P&M and MDI-type protocols.

### A. Three-state protocol

Here, we first explain how to obtain  $\Delta$  in Eq. (S41) by using SDP techniques and then, we show that when the emitted states in Eq. (S2) satisfy the extra assumption  $\langle \phi_i | \phi_j^\perp \rangle_B = 0$  for all  $i, j \in \{0_Z, 1_Z, 0_X\}$  such that  $i \neq j$ , which is reasonable for some source imperfections,  $\Delta$  can be derived analytically. Finally, we compare the secret-key rate obtainable in the general case with that obtainable under the extra assumption on the emitted states for different parameter regimes.

For this, it is useful to first rewrite the states  $|\Psi_{\text{Tar}}\rangle_{DAB}$  and  $|\Psi_{\text{Ref}}\rangle_{DAB}$  in Eqs. (S21) and (S22), respectively, as

$$\begin{aligned} |\Psi_{\text{Tar}}\rangle_{DAB} &= \frac{1}{\sqrt{1 + c_2 q_{\text{vir1}}^\phi}} \left[ \sqrt{q_{\text{vir0}}^\psi} |0\rangle_D |0\rangle_A |\psi_{\text{vir0}}\rangle_B + |1\rangle_D |0\rangle_A \left( a \sqrt{c_2 q_{\text{vir1}}^\phi} |\psi_{0_X}\rangle_B + b \sqrt{q_{\text{vir1}}^\psi} |\psi_{\text{vir1}}\rangle_B \right) \right. \\ &\quad \left. + |1\rangle_D |1\rangle_A \left( b \sqrt{c_2 q_{\text{vir1}}^\phi} |\psi_{0_X}\rangle_B - a \sqrt{q_{\text{vir1}}^\psi} |\psi_{\text{vir1}}\rangle_B \right) \right], \\ |\Psi_{\text{Ref}}\rangle_{DAB} &= \frac{1}{\sqrt{1 + c_2 q_{\text{vir1}}^\phi}} \left[ \sqrt{q_{\text{vir0}}^\phi} |0\rangle_D |0\rangle_A |\psi_{0_X}\rangle_B + \sqrt{c_1 q_{\text{vir1}}^\phi} |1\rangle_D |0\rangle_A |\psi_{0_Z}\rangle_B + \sqrt{c_1 q_{\text{vir1}}^\phi} |1\rangle_D |1\rangle_A |\psi_{1_Z}\rangle_B \right], \end{aligned} \quad (\text{S237})$$

$$(\text{S238})$$

with  $a = b = 1/\sqrt{2}$ . Then,  $\text{Re} \langle \Psi_{\text{Tar}} | \Psi_{\text{Ref}} \rangle_{DAB}$  can be calculated as follows

$$\begin{aligned} \text{Re} \langle \Psi_{\text{Tar}} | \Psi_{\text{Ref}} \rangle_{DAB} &= \frac{1}{1 + c_2 q_{\text{vir1}}^\phi} \left[ \sqrt{q_{\text{vir0}}^\phi q_{\text{vir0}}^\psi} \text{Re} \langle \psi_{\text{vir0}} | \psi_{0_X} \rangle_B + \sqrt{c_1 q_{\text{vir1}}^\phi} \left( a \sqrt{c_2 q_{\text{vir1}}^\phi} \text{Re} \langle \psi_{0_X} | \psi_{0_Z} \rangle_B \right. \right. \\ &\quad \left. \left. + b \sqrt{q_{\text{vir1}}^\psi} \text{Re} \langle \psi_{\text{vir1}} | \psi_{0_Z} \rangle_B \right) + \sqrt{c_1 q_{\text{vir1}}^\phi} \left( b \sqrt{c_2 q_{\text{vir1}}^\phi} \text{Re} \langle \psi_{0_X} | \psi_{1_Z} \rangle_B - a \sqrt{q_{\text{vir1}}^\psi} \text{Re} \langle \psi_{\text{vir1}} | \psi_{1_Z} \rangle_B \right) \right] \\ &= \frac{1}{1 + c_2 q_{\text{vir1}}^\phi} \left[ \left( \frac{\sqrt{q_{\text{vir0}}^\phi}}{2} + a \sqrt{c_1 c_2 q_{\text{vir1}}^\phi} \right) \text{Re} \langle \psi_{0_Z} | \psi_{0_X} \rangle_B + \left( \frac{\sqrt{q_{\text{vir0}}^\phi}}{2} + b \sqrt{c_1 c_2 q_{\text{vir1}}^\phi} \right) \text{Re} \langle \psi_{1_Z} | \psi_{0_X} \rangle_B \right. \\ &\quad \left. + (a + b) \frac{\sqrt{c_1 q_{\text{vir1}}^\phi}}{2} (1 - \text{Re} \langle \psi_{0_Z} | \psi_{1_Z} \rangle_B) \right], \end{aligned} \quad (\text{S239})$$

where in the last equality we have used the definitions of the virtual states in Eq. (S9) such that  $\text{Re} \langle \psi_{\text{vir0}} | \psi_{0_X} \rangle_B = (\text{Re} \langle \psi_{0_Z} | \psi_{0_X} \rangle_B + \text{Re} \langle \psi_{1_Z} | \psi_{0_X} \rangle_B) / (2\sqrt{q_{\text{vir0}}^\psi})$  and  $\text{Re} \langle \psi_{\text{vir1}} | \psi_{\alpha_Z} \rangle_B = (-1)^\alpha (1 - \text{Re} \langle \psi_{0_Z} | \psi_{1_Z} \rangle_B) / (2\sqrt{q_{\text{vir1}}^\psi})$  for  $\alpha \in \{0, 1\}$ , with

$$\text{Re} \langle \psi_i | \psi_j \rangle_B = \text{Re} \left[ (1 - \epsilon) \langle \phi_i | \phi_j \rangle_B + \sqrt{(1 - \epsilon)\epsilon} \langle \phi_i | \phi_j^\perp \rangle_B + \sqrt{\epsilon(1 - \epsilon)} \langle \phi_i^\perp | \phi_j \rangle_B + \epsilon \langle \phi_i^\perp | \phi_j^\perp \rangle_B \right]. \quad (\text{S240})$$

#### 1. Numerical bound using SDP techniques

To construct the SDP, let us redefine the tuple  $\{0_Z, 1_Z, 0_X\}$  as  $\{1, 2, 3\}$  and rename the states  $|\psi_j\rangle_B$ ,  $|\phi_j\rangle_B$  and  $|\phi_j^\perp\rangle_B$  accordingly. Moreover, let us define  $G$  as the Gram matrix of the vector set  $\{|\phi_1\rangle_B, |\phi_2\rangle_B, |\phi_3\rangle_B, |\phi_1^\perp\rangle_B, |\phi_2^\perp\rangle_B, |\phi_3^\perp\rangle_B\}$  such that, for example,  $G[1, 1] = \langle \phi_1 | \phi_1 \rangle_B$  and  $G[1, 5] = \langle \phi_1 | \phi_2^\perp \rangle_B$ . That is,  $G[i, j] \equiv \langle i | G | j \rangle$  denotes the coefficient in the  $i$ -th column and  $j$ -th row of  $G$ . Using this redefinition, we can rewrite Eq. (S239) as

$$\begin{aligned} \text{Re} \langle \Psi_{\text{Tar}} | \Psi_{\text{Ref}} \rangle_{DAB} &= \frac{1}{1 + c_2 q_{\text{vir1}}^\phi} \left[ \left( \frac{\sqrt{q_{\text{vir0}}^\phi}}{2} + a \sqrt{c_1 c_2 q_{\text{vir1}}^\phi} \right) \text{Re} \langle \psi_1 | \psi_3 \rangle_B + \left( \frac{\sqrt{q_{\text{vir0}}^\phi}}{2} + b \sqrt{c_1 c_2 q_{\text{vir1}}^\phi} \right) \text{Re} \langle \psi_2 | \psi_3 \rangle_B \right. \\ &\quad \left. + (a + b) \frac{\sqrt{c_1 q_{\text{vir1}}^\phi}}{2} (1 - \text{Re} \langle \psi_1 | \psi_2 \rangle_B) \right], \end{aligned} \quad (\text{S241})$$

which is the objective function of the SDP. Note that, as required, it is guaranteed to be real and it can be expressed as a linear function of elements of  $G$ , since

$$\begin{aligned} \text{Re} \langle \psi_i | \psi_j \rangle_B &= \text{Re} \left[ (1 - \epsilon) G[i, j] + \sqrt{(1 - \epsilon)\epsilon} G[i, j + 3] + \sqrt{\epsilon(1 - \epsilon)} G[i + 3, j] + \epsilon G[i + 3, j + 3] \right] \\ &= (1 - \epsilon) \text{Re} G[i, j] + \sqrt{(1 - \epsilon)\epsilon} \text{Re} G[i, j + 3] + \sqrt{\epsilon(1 - \epsilon)} \text{Re} G[i + 3, j] + \epsilon \text{Re} G[i + 3, j + 3], \end{aligned} \quad (\text{S242})$$

and  $\text{Re } G[i, j] = (G[i, j] + G[j, i])/2$ . The constraints of the SDP can then be listed as follows

$$\begin{aligned}
G &\geq 0; \\
G[j, j] &= \langle \phi_j | \phi_j \rangle_B = 1, & \forall j \in \{1, 2, 3\}; \\
G[j+3, j+3] &= \langle \phi_j^\perp | \phi_j^\perp \rangle_B = 1, & \forall j \in \{1, 2, 3\}; \\
G[j, j+3] &= \langle \phi_j | \phi_j^\perp \rangle_B = 0, & \forall j \in \{1, 2, 3\}; \\
G[1, 2] &= \langle \phi_1 | \phi_2 \rangle_B = \cos(\kappa\pi/2); \\
G[1, 3] &= \langle \phi_1 | \phi_3 \rangle_B = \cos(\kappa\pi/4); \\
G[2, 3] &= \langle \phi_2 | \phi_3 \rangle_B = \cos(\kappa\pi/4);
\end{aligned} \tag{S243}$$

where we have used Eqs. (S12) and (S13) to calculate the inner products  $\langle \phi_i | \phi_j \rangle_B$ . Note that the first inequality in Eq. (S243) is the standard positive semidefinite constraint, which holds because  $G$  is a Gram matrix, and that the others are valid SDP constraints since they can be written as a linear function of elements of  $G$ . Using the SDP we can obtain a lower bound on  $\text{Re} \langle \Psi_{\text{Tar}} | \Psi_{\text{Ref}} \rangle_{DAB}$ , and then directly use Eq. (S41) to define  $\Delta$ .

Note that, for concreteness, we have considered the scenario in which one has knowledge on the fidelity between the actual states  $\{|\psi_j\rangle_B\}_j$  and the characterized qubit states  $\{|\phi_j\rangle_B\}_j$ . However, as explained in the subsection ‘‘A more general form of Eq. (1)’’ under Methods, the approach presented here is also valid when one has knowledge between the actual states  $\{|\psi_j\rangle_B\}_j$  and *any* characterized states  $\{|\tilde{\phi}_j\rangle_B\}_j$ , not necessarily qubits. In this case, one only needs to trivially substitute  $|\phi_j\rangle_B \rightarrow |\tilde{\phi}_j\rangle_B$  and  $|\phi_j^\perp\rangle_B \rightarrow |\tilde{\phi}_j^\perp\rangle_B$  in the SDP above, and then modify the constraints based on the knowledge of the inner products  $\langle \tilde{\phi}_{j'} | \tilde{\phi}_j \rangle_B \forall j, j'$ .

## 2. Analytical bound with an additional assumption

If the emitted states in Eq. (S2) satisfy  $\langle \phi_i | \phi_j^\perp \rangle_B = 0$  for all  $i, j \in \{0_Z, 1_Z, 0_X\}$  such that  $i \neq j$ , it is straightforward to obtain  $\Delta$  by analytically deriving a lower bound on  $\text{Re} \langle \Psi_{\text{Tar}} | \Psi_{\text{Ref}} \rangle_{DAB}$ . First, using Eqs. (S12) and (S13) we can directly calculate the inner products  $\langle \phi_i | \phi_j \rangle_B$  in Eq. (S240) to be  $\langle \phi_{0_Z} | \phi_{1_Z} \rangle_B = \cos(\kappa\pi/2)$  and  $\langle \phi_{0_Z} | \phi_{0_X} \rangle_B = \langle \phi_{1_Z} | \phi_{0_X} \rangle_B = \cos(\kappa\pi/4)$ . Then, even though the side-channel states  $|\phi_j^\perp\rangle_B$  are uncharacterized, it must be that  $-1 \leq \text{Re} \langle \phi_i^\perp | \phi_j^\perp \rangle_B \leq 1$  since  $\text{Re} \langle \phi_i^\perp | \phi_j^\perp \rangle_B$  is the real part of an inner product between two normalized states. Therefore, Eq. (S239) can be lower bounded by

$$\begin{aligned}
\text{Re} \langle \Psi_{\text{Tar}} | \Psi_{\text{Ref}} \rangle_{DAB} &\geq \frac{1}{1 + c_2 q_{\text{vir1}}^\phi} \left( \left[ \sqrt{q_{\text{vir0}}^\phi} + (a+b) \sqrt{c_1 c_2 q_{\text{vir1}}^\phi} \right] [(1-\epsilon) \cos(\kappa\pi/4) - \epsilon] \right. \\
&\quad \left. + (a+b) \frac{\sqrt{c_1 q_{\text{vir1}}^\phi}}{2} [1 - (1-\epsilon) \cos(\kappa\pi/2) - \epsilon] \right).
\end{aligned} \tag{S244}$$

## 3. Comparison between the numerical and analytical bounds

For the comparison between the numerical and analytical bounds, we evaluate the secret-key rate obtainable when employing our analysis with the SDP techniques described above, which does not assume  $\langle \phi_i | \phi_j^\perp \rangle_B = 0 \forall i, j$  when  $i \neq j$ , and with Eq. (S244). In the simulations, we take  $\delta = 0.063$  [S32, S33] and  $\epsilon \in \{10^{-6}, 10^{-3}\}$ . All the other experimental parameters are the same as in the Main Text.

The results are presented in Fig. S12, where the solid and dashed lines correspond to using the numerical and analytical bounds, respectively. This figure shows that these bounds provide very similar secret-key rates. In fact, when  $\epsilon = 10^{-3}$ , the two curves are indistinguishable to the naked eye. This suggests that, while the extra assumption helps to simplify the analysis, it does not actually result in an appreciable key-rate improvement.

## B. Coherent-light-based MDI protocol

Here, we explain how to construct an SDP to find an upper bound on the coin imbalance parameter  $\Delta := 1 - \text{Re} \langle \Psi_{\text{Tar}} | \Psi_{\text{Ref}} \rangle_{DAB}$  for the coherent-light-based MDI protocol analyzed in Section SM4 A. Using Eq. (S173) and

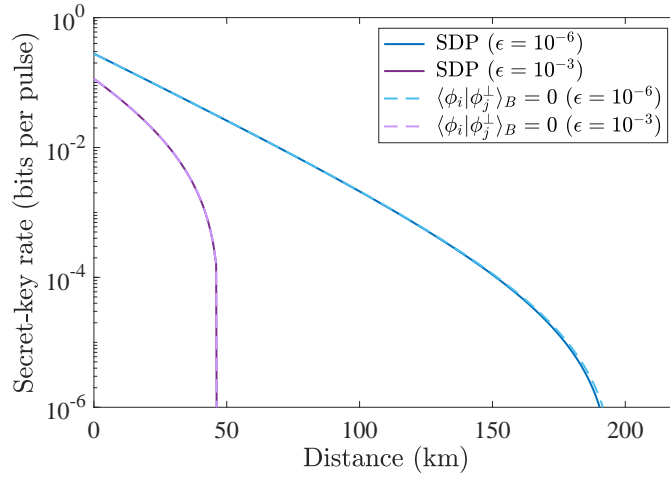

Figure S12. Secret-key rate per pulse as a function of the distance (km) for  $\delta = 0.063$  and different values of  $\epsilon$  when using our numerical bound based on SDP and our analytical bound that assumes  $\langle \phi_i | \phi_j^\perp \rangle_B = 0$ .

Eq. (S2), we can express the states emitted by Alice and Bob as

$$|\psi_j\rangle_{B_u} = \sqrt{1-\epsilon} |\tilde{\phi}_j\rangle_{B_u} + \sqrt{\epsilon} |\tilde{\phi}_j^\perp\rangle_{B_u}, \quad (\text{S245})$$

where  $j \in \{0_Z, 1_Z, 0_X\}$ ,  $u \in \{a, b\}$ ,  $|\tilde{\phi}_{0_Z}\rangle_{B_u} = |\sqrt{\mu}\rangle_{B_u}$ ,  $|\tilde{\phi}_{1_Z}\rangle_{B_u} = |-\sqrt{\mu}\rangle_{B_u}$ ,  $|\tilde{\phi}_{0_X}\rangle_{B_u} = |\text{vac}\rangle_{B_u}$ , and  $\langle \tilde{\phi}_j^\perp | \tilde{\phi}_j \rangle_{B_u} = 0$ <sup>8</sup>. Taking the tensor product of Eq. (S245) for  $u = a$  and  $u = b$ , we obtain the following expression for Alice and Bob's joint states,

$$|\psi_{ij}\rangle_B := |\psi_i\rangle_{B_a} \otimes |\psi_j\rangle_{B_b} = \sqrt{1-\xi} |\tilde{\phi}_{ij}\rangle_B + \sqrt{\xi} |\tilde{\phi}_{ij}^\perp\rangle_B, \quad (\text{S246})$$

where we have defined  $\xi := 1 - (1 - \epsilon)^2$ ,  $|\tilde{\phi}_{ij}\rangle_B := |\tilde{\phi}_i\rangle_{B_a} \otimes |\tilde{\phi}_j\rangle_{B_b}$ , and  $|\tilde{\phi}_{ij}^\perp\rangle_B$  is a normalized state that can be easily shown to satisfy  $\langle \tilde{\phi}_{ij}^\perp | \tilde{\phi}_{ij} \rangle_B = 0$ . Now, let us define an ordering for Alice and Bob's joint setting choices  $ij \in \{0_Z 0_Z, 0_Z 1_Z, 0_Z 0_X, 1_Z 0_Z, 1_Z 1_Z, 1_Z 0_X, 0_X 0_Z, 0_X 1_Z, 0_X 0_X\}$  using the index  $k \in \{1, 2, 3, 4, 5, 6, 7, 8, 9\}$ , and let us define  $G$  as the Gram matrix of the union of vector sets  $\{|\tilde{\phi}_{ij}\rangle_B\}_{ij}$  and  $\{|\tilde{\phi}_{ij}^\perp\rangle_B\}_{ij}$ , with the latter being indexed by  $k \in \{10, 11, 12, 13, 14, 15, 16, 17, 18\}$ . From the ordering we have defined, we have that the elements of  $G$  are, e.g.,  $G[1, 6] = \langle \tilde{\phi}_{0_Z 0_Z} | \tilde{\phi}_{1_Z 0_X} \rangle_B$ ,  $G[10, 6] = \langle \tilde{\phi}_{0_Z 0_Z} | \tilde{\phi}_{1_Z 0_X}^\perp \rangle_B$ ,  $G[3, 5] = \langle \tilde{\phi}_{0_Z 0_X} | \tilde{\phi}_{1_Z 1_Z} \rangle_B$ ,  $G[3, 14] = \langle \tilde{\phi}_{0_Z 0_X} | \tilde{\phi}_{1_Z 1_Z}^\perp \rangle_B$ , and so on. Now, let us define

$$G_\star(k, k') := (1 - \xi) \text{Re } G[k, k'] + \sqrt{(1 - \xi)\xi} (\text{Re } G[k + 9, k'] + \text{Re } G[k, k' + 9]) + \xi \text{Re } G[k + 9, k' + 9], \quad (\text{S247})$$

where  $\text{Re } G[k, k'] = (G[k, k'] + G[k', k])/2$  since  $G$  is Hermitian. Note that we have, e.g.,  $G_\star(1, 6) = \text{Re } \langle \psi_{0_Z 0_Z} | \psi_{1_Z 0_X} \rangle_B$ ,  $G_\star(3, 5) = \text{Re } \langle \psi_{0_Z 0_X} | \psi_{1_Z 1_Z} \rangle_B$ , and so on. Using the definition of  $\langle \Psi_{\text{Tar}} | \Psi_{\text{Ref}} \rangle_{DAB}$  in Eq. (S196) and our definition

<sup>8</sup> Note that the set of states  $\{|\tilde{\phi}_{0_Z}\rangle_{B_u}, |\tilde{\phi}_{1_Z}\rangle_{B_u}, |\tilde{\phi}_{0_X}\rangle_{B_u}\}$  defined here is different from the set of states  $\{|\phi_{0_Z}\rangle_{B_u}, |\phi_{1_Z}\rangle_{B_u}, |\phi_{0_X}\rangle_{B_u}\}$  defined in Section SM4 A. In particular, while  $|\phi_{0_Z}\rangle_{B_u} = |\tilde{\phi}_{0_Z}\rangle_{B_u} = |\sqrt{\mu}\rangle_{B_u}$  and  $|\phi_{1_Z}\rangle_{B_u} = |\tilde{\phi}_{1_Z}\rangle_{B_u} = |-\sqrt{\mu}\rangle_{B_u}$ ,  $|\phi_{0_X}\rangle_{B_u} \neq |\tilde{\phi}_{0_X}\rangle_{B_u} = |\text{vac}\rangle_{B_u}$ , since  $|\phi_{0_X}\rangle_{B_u}$  was defined as the projection of  $|\text{vac}\rangle_{B_u}$  onto the qubit subspace spanned by  $\{|\sqrt{\mu}\rangle_{B_u}, |-\sqrt{\mu}\rangle_{B_u}\}$ . The reason is that  $\{|\phi_{0_Z}\rangle_{B_u}, |\phi_{1_Z}\rangle_{B_u}, |\phi_{0_X}\rangle_{B_u}\}$  needed to be qubit states, in order to derive the LT formulas in Eq. (S179), which are then used as a blueprint to define the reference and target states. However, here, while  $\{|\tilde{\phi}_{0_Z}\rangle_{B_u}, |\tilde{\phi}_{1_Z}\rangle_{B_u}, |\tilde{\phi}_{0_X}\rangle_{B_u}\}$  need to be known states, they do not need to be qubit states. The reason is that we can employ any state expansion of the actual states to calculate an upper bound on  $\Delta$ , and using the definition  $|\tilde{\phi}_{0_X}\rangle_{B_u} = |\text{vac}\rangle_{B_u}$  results in a better bound.

in Eq. (S247), we can write our objective function as

$$\begin{aligned} \text{Re} \langle \Psi_{\text{Tar}} | \Psi_{\text{Ref}} \rangle_{DAB} = & \frac{q_{\text{vir}0}^{\phi}}{4C} (G_{\star}(9, 1) + G_{\star}(9, 2) + G_{\star}(9, 4) + G_{\star}(9, 5)) + \frac{\sqrt{2c_1 q_{\text{vir}01}^{\phi}}}{2C} \left( \frac{1}{4} (G_{\star}(3, 1) - G_{\star}(3, 2) + G_{\star}(3, 4) \right. \\ & - G_{\star}(3, 5) - G_{\star}(8, 1) + G_{\star}(8, 2) - G_{\star}(8, 4) + G_{\star}(8, 5) + G_{\star}(1, 7) + G_{\star}(2, 7) - G_{\star}(4, 7) - G_{\star}(5, 7) - G_{\star}(6, 1) - G_{\star}(6, 2) \\ & + G_{\star}(6, 4) + G_{\star}(6, 5)) + \sqrt{c_2 q_{\text{vir}01}^{\phi}} (G_{\star}(3, 9) + G_{\star}(8, 9) + G_{\star}(7, 9) + G_{\star}(6, 9)) \Big) + \frac{c_1 q_{\text{vir}1}^{\phi}}{4C} (2 - G_{\star}(2, 1) - G_{\star}(4, 1) \\ & + G_{\star}(5, 1) + G_{\star}(4, 2) - G_{\star}(5, 2) - G_{\star}(5, 4)) + \frac{q_{\text{vir}11}^{\phi} \sqrt{c_1 c_2}}{2\sqrt{2}C} \left( c_1 (G_{\star}(1, 7) - G_{\star}(4, 7) + 2G_{\star}(1, 3) + G_{\star}(2, 7) - G_{\star}(5, 7) \right. \\ & + 2G_{\star}(2, 8) - G_{\star}(4, 7) + G_{\star}(4, 6) + 2G_{\star}(4, 3) - G_{\star}(5, 7) + G_{\star}(5, 6) + 2G_{\star}(5, 8)) + 2c_2 (G_{\star}(9, 7) + G_{\star}(9, 6)) \Big), \end{aligned} \quad (\text{S248})$$

which is a linear function of elements of  $G$ , and therefore a valid SDP objective function. Here,  $q_{\text{vir}\alpha\beta}^{\phi} := q_{\text{vir}\alpha}^{\phi} q_{\text{vir}\beta}^{\phi}$  for  $\alpha, \beta \in \{0, 1\}$ , where  $q_{\text{vir}\alpha}^{\phi}$  and  $q_{\text{vir}\beta}^{\phi}$  are defined in Eq. (S177),  $c_1$  and  $c_2$  are defined in Eq. (S180), and  $C$  is defined in Eq. (S191). Also, using the fact that  $\langle \tilde{\phi}_{ij} | \tilde{\phi}_{ij} \rangle_B = 1$ ,  $\langle \tilde{\phi}_{ij}^{\perp} | \tilde{\phi}_{ij}^{\perp} \rangle_B = 1$  and  $\langle \tilde{\phi}_{ij}^{\perp} | \tilde{\phi}_{ij} \rangle_B = 0$  for all  $i, j$ , and our knowledge of the states  $\{|\tilde{\phi}_{ij}\rangle_B\}_{ij}$  (and thus our knowledge of the inner product between any two states in this set), we obtain the constraints

$$\begin{aligned} G &\geq 0; \\ G[k, k] &= 1, & \forall k \in \{1, \dots, 9\}; \\ G[k + 9, k] &= 0, & \forall k \in \{1, \dots, 9\}; \\ G[k + 9, k + 9] &= 1, & \forall k \in \{1, \dots, 9\}; \\ G[1, 2] = G[1, 4] = G[2, 5] = G[3, 6] = G[4, 5] = G[7, 8] &= \langle \sqrt{\mu} | -\sqrt{\mu} \rangle = \exp(-2\mu); \\ G[1, 3] = G[1, 7] = G[2, 8] = G[3, 9] = G[4, 6] = G[7, 9] &= \langle \sqrt{\mu} | \text{vac} \rangle = \exp(-\mu/2); \\ G[1, 5] = G[2, 4] &= (\langle \sqrt{\mu} | -\sqrt{\mu} \rangle)^2 = \exp(-4\mu); \\ G[1, 6] = G[1, 8] = G[2, 7] = G[3, 4] &= \langle \sqrt{\mu} | -\sqrt{\mu} \rangle \langle \sqrt{\mu} | \text{vac} \rangle = \exp(-5\mu/2); \\ G[1, 9] = G[3, 7] &= (\langle \sqrt{\mu} | \text{vac} \rangle)^2 = \exp(-\mu); \\ G[2, 3] = G[4, 7] = G[5, 6] = G[5, 8] = G[6, 9] = G[8, 9] &= \langle -\sqrt{\mu} | \text{vac} \rangle = \exp(-\mu/2); \\ G[2, 6] = G[3, 5] = G[4, 8] = G[5, 7] &= \langle \sqrt{\mu} | -\sqrt{\mu} \rangle \langle -\sqrt{\mu} | \text{vac} \rangle = \exp(-5\mu/2); \\ G[5, 9] = G[6, 8] &= (\langle -\sqrt{\mu} | \text{vac} \rangle)^2 = \exp(-\mu); \\ G[2, 9] = G[3, 8] = G[4, 9] = G[6, 7] &= \langle \sqrt{\mu} | \text{vac} \rangle \langle -\sqrt{\mu} | \text{vac} \rangle = \exp(-\mu); \end{aligned} \quad (\text{S249})$$

all of which are valid SDP constraints. Our SDP is defined then as the optimization problem of finding the minimum of Eq. (S248) given the constraints in Eq. (S249) and the standard SDP constraint  $G \geq 0$  (which holds since a Gram matrix is always positive semidefinite). By solving the dual problem of this SDP, one can obtain a rigorous lower bound on  $\text{Re} \langle \Psi_{\text{Tar}} | \Psi_{\text{Ref}} \rangle_{DAB}$ , and thus a rigorous upper bound on  $\Delta := 1 - \text{Re} \langle \Psi_{\text{Tar}} | \Psi_{\text{Ref}} \rangle_{DAB}$ .

### SE3. CHANNEL MODEL

#### A. Prepare-and-measure protocol

For the simulations, we consider, as examples, the three-state and the BB84 protocols with a phase encoding scheme. In the presence of qubit flaws, Alice's prepared qubit states can be expressed as

$$\frac{1}{\sqrt{2}} \left( |1\rangle_r |0\rangle_s + e^{i(\varphi_j + \delta\varphi_j/\pi)} |0\rangle_r |1\rangle_s \right), \quad (\text{S250})$$

where 0 and 1 denote the photon number, the subscript  $r$  ( $s$ ) stands for reference (signal) pulse, and  $\delta$  quantifies the deviation of the phase modulation from the desired phases  $\varphi_j$  for  $j \in \{0_Z, 1_Z, 0_X, 1_X\}$ . For simplicity, we assume that these phases take the values:  $\varphi_{0_Z} = 0$ ,  $\varphi_{1_Z} = \pi$ ,  $\varphi_{0_X} = \pi/2$  and  $\varphi_{1_X} = 3\pi/2$ . Note that if we define  $|1\rangle_r |0\rangle_s =: |0_Y\rangle_B$  and  $|0\rangle_r |1\rangle_s =: |1_Y\rangle_B$ , and then use the fact that  $|\alpha_Y\rangle_B = (|0_Z\rangle_B + (-1)^\alpha i |1_Z\rangle_B)/\sqrt{2}$  with  $\alpha \in \{0, 1\}$ , it is

straightforward to obtain the states in Eq. (S12) with  $\theta_j = \varphi_j \kappa/2$ , after a change of global phase. The non-qubit imperfections are not considered in the calculations below because  $\epsilon$  is small, and thus it does not significantly affect the estimated experimental observables.

The overall transmission efficiency of the system is defined as  $\eta = \eta_c \eta_d$ , where  $\eta_c = 10^{-0.02l}$  is the channel transmission rate, with  $l$  denoting the length of the channel in km, and  $\eta_d$  is the detector efficiency. We assume, for simplicity, that there is no misalignment in the channel and that the detector dark count probability  $p_d$  is independent of Bob's basis selection. On the receiving unit, a phase  $\varphi_B = 0$  ( $\varphi_B = -\pi/2$ ) corresponds to selecting the  $Z$  ( $X$ ) measurement basis, but due to an imperfect phase modulator this phase is shifted by  $-\delta\varphi_B/\pi$ . By neglecting the terms with  $p_d^2$  we can then express the yields as

$$Y_j^{0x} \approx \left(1 - \frac{\eta}{2}\right) p_d + \frac{\eta}{4} \left[1 + \sin\left(\varphi_j + \frac{\delta\varphi_j}{\pi} + \frac{\delta}{2}\right)\right] \left(1 - \frac{p_d}{2}\right) + \frac{\eta}{4} \left[1 - \sin\left(\varphi_j + \frac{\delta\varphi_j}{\pi} + \frac{\delta}{2}\right)\right] \frac{p_d}{2}, \quad (\text{S251})$$

$$Y_j^{1x} \approx \left(1 - \frac{\eta}{2}\right) p_d + \frac{\eta}{4} \left[1 + \sin\left(\varphi_j + \frac{\delta\varphi_j}{\pi} + \frac{\delta}{2}\right)\right] \frac{p_d}{2} + \frac{\eta}{4} \left[1 - \sin\left(\varphi_j + \frac{\delta\varphi_j}{\pi} + \frac{\delta}{2}\right)\right] \left(1 - \frac{p_d}{2}\right), \quad (\text{S252})$$

$$Y_j^{0z} \approx \left(1 - \frac{\eta}{2}\right) p_d + \frac{\eta}{4} \left[1 + \cos\left(\varphi_j + \frac{\delta\varphi_j}{\pi}\right)\right] \left(1 - \frac{p_d}{2}\right) + \frac{\eta}{4} \left[1 - \cos\left(\varphi_j + \frac{\delta\varphi_j}{\pi}\right)\right] \frac{p_d}{2}, \quad (\text{S253})$$

$$Y_j^{1z} \approx \left(1 - \frac{\eta}{2}\right) p_d + \frac{\eta}{4} \left[1 + \cos\left(\varphi_j + \frac{\delta\varphi_j}{\pi}\right)\right] \frac{p_d}{2} + \frac{\eta}{4} \left[1 - \cos\left(\varphi_j + \frac{\delta\varphi_j}{\pi}\right)\right] \left(1 - \frac{p_d}{2}\right), \quad (\text{S254})$$

where the superscript denotes Bob's outcome. Using Eqs. (S253) and (S254), we can directly calculate the rate at which Bob obtains a detection event conditioned on Alice and Bob choosing the  $Z$  basis

$$Y_Z = \frac{1}{2} (Y_{0z}^{0z} + Y_{1z}^{0z} + Y_{0z}^{1z} + Y_{1z}^{1z}) = \frac{1}{2} \left[4 \left(1 - \frac{\eta}{2}\right) p_d + \eta\right], \quad (\text{S255})$$

and the bit-error rate

$$e_Z = \frac{Y_{1z}^{0z} + Y_{0z}^{1z}}{Y_{0z}^{0z} + Y_{1z}^{0z} + Y_{0z}^{1z} + Y_{1z}^{1z}} = \frac{2(1 - \frac{\eta}{2})p_d + \frac{\eta}{4}(1 + p_d) + \frac{\eta}{4}(p_d - 1)\cos\delta}{4 \left(1 - \frac{\eta}{2}\right) p_d + \eta}. \quad (\text{S256})$$

## B. Coherent-light-based MDI protocol

Here, we present the channel model used for the simulations in Section SM4A, which is the same as that of Ref. [S34]. We model the loss from Alice and Bob to Charlie with a beamsplitter of transmittance  $\sqrt{\eta}$  and assume that there is no misalignment in the channel. Moreover, for simplicity, we assume that Charlie's detectors have the same dark count probability  $p_d$ . The conditional probability that Charlie observes a click on detector  $D_c$  and no click on detector  $D_d$  (corresponding to the announcement  $k_c = 1, k_d = 0$ ), given that Alice and Bob have sent the states  $|\psi_i\rangle_{B_a}$  and  $|\psi_j\rangle_{B_b}$ , respectively, is given by

$$Y_{i,j}^{k_c=1, k_d=0} = (1 - p_d)^2 \exp \left[ -\sqrt{\eta} \left( \frac{|\gamma_i|^2 + |\gamma_j|^2}{2} - |\gamma_i||\gamma_j| \cos(\phi_i - \phi_j) \right) \right] \\ \times \left\{ 1 - \exp \left[ -\sqrt{\eta} \left( \frac{|\gamma_i|^2 + |\gamma_j|^2}{2} + |\gamma_i||\gamma_j| \cos(\phi_i - \phi_j) \right) \right] \right\} + p_d(1 - p_d), \quad (\text{S257})$$

where  $i, j \in \{0_Z, 1_Z, 0_X\}$ ,  $\gamma_{0z} = \sqrt{\mu}$ ,  $\gamma_{1z} = -\sqrt{\mu}$ ,  $\gamma_{0x} = 0$ ,  $\phi_i = \arg(\gamma_i)$  and  $\phi_j = \arg(\gamma_j)$ . Similarly, the probability that he observes a click on detector  $D_d$  and no click on detector  $D_c$  (corresponding to the announcement  $k_c = 0, k_d = 1$ ) is given by

$$Y_{i,j}^{k_c=0, k_d=1} = (1 - p_d)^2 \exp \left[ -\sqrt{\eta} \left( \frac{|\gamma_i|^2 + |\gamma_j|^2}{2} - |\gamma_i||\gamma_j| \cos(\phi_i - \phi_j + \pi) \right) \right] \\ \times \left\{ 1 - \exp \left[ -\sqrt{\eta} \left( \frac{|\gamma_i|^2 + |\gamma_j|^2}{2} + |\gamma_i||\gamma_j| \cos(\phi_i - \phi_j + \pi) \right) \right] \right\} + p_d(1 - p_d). \quad (\text{S258})$$

Therefore, the probability that Charlie obtains a detection is given by

$$Y_{i,j}^{\text{det}} := Y_{i,j}^{k_c=1, k_d=0} + Y_{i,j}^{k_c=0, k_d=1}. \quad (\text{S259})$$

Also, the bit-error rate can be calculated to be

$$e_Z = \frac{p_d}{2p_d + \exp(2\mu\sqrt{\eta}) - 1}. \quad (\text{S260})$$

## SE4. HIGH-LEVEL DESCRIPTION OF THE CODE

In this Section, we provide a high-level description of the code written to perform the simulations. We note that our SDP optimization (see Section SE2) was performed using MATLAB, in conjunction with the YALMIP toolbox and the MOSEK solver. Nonetheless, alternative programming languages, toolboxes, and solvers could also be employed to attain equivalent results. For ease of discussion, we consider the asymptotic regime and the particular three-state protocol introduced in Section SM1 B to explain the code. However, it is rather straightforward to generalize it to the finite-key regime and to other P&M or MDI-type protocols.

### 1. Definition of the protocol parameters

- Define the value of  $\epsilon$  and  $\delta$ .
- Define the coefficients  $c_1$  and  $c_2$  in Eq. (S16) and the probabilities  $q_{\text{vir}\alpha}^\phi$  in Eq. (S18).
- Define  $\Delta = 1 - \text{Re} \langle \Psi_{\text{Ref}} | \Psi_{\text{Tar}} \rangle_{DAB}$ : if  $\epsilon = 0$ , set  $\Delta = 0$ ; otherwise, use the SDP techniques explained in Section SE2 A 1 to obtain an upper bound on  $\Delta$ .

### 2. Definition of the channel model

- Define the probabilities  $P_{Z_A}$ ,  $P_{X_A}$ ,  $P_{Z_B}$  and  $P_{X_B}$ . To generate Fig. 1 in the Main Text we have used  $P_{Z_A} = P_{Z_B} = 0.9$  and  $P_{X_A} = P_{X_B} = 0.1$ .
- Define the parameters  $f$ ,  $p_d$ ,  $\eta_d$  and the repetition rate of the protocol. The values used to generate all figures in this work are stated in the Main Text.
- Define the yields  $Y_j^{0x}$  and  $Y_j^{1x}$  for  $j \in \{0_Z, 1_Z, 0_X\}$  and  $Y_Z$ . To generate Fig. 1, we have used Eq. (S251), Eq. (S252), and Eq. (S255), respectively.
- Define the bit-error rate  $e_Z$ . To generate Fig. 1, we have used Eq. (S256).

### 3. Calculation of $e_{\text{ph}}^U$

- Define the conditions to apply the function  $G_+(y, z)$  with

$$y = \frac{q_{\text{vir}0}^\phi Y_{0_X}^{1x} + c_1 q_{\text{vir}1}^\phi (Y_{0_Z}^{0x} + Y_{1_Z}^{0x})}{q_{\text{vir}0}^\phi Y_{0_X} + c_1 q_{\text{vir}1}^\phi Y_Z},$$

$$z = 1 - \frac{2\Delta(1 + c_1 q_{\text{vir}1}^\phi)}{Y_Z + q_{\text{vir}0}^\phi Y_{0_X} + q_{\text{vir}1}^\phi (c_1 Y_{0_Z} + c_2 Y_{1_Z} + c_3 Y_{1_X})}. \quad (\text{S261})$$

Namely, if  $y < z^2$ ,  $G_+(y, z) = g_+(y, z)$ , where  $g_+(y, z)$  is defined in Eq. (S230); otherwise,  $G_+(y, z) = 1$ .

- Substitute the value of  $G_+(y, z)$  in Eq. (S46) and use it to calculate  $e_{\text{ph}}^U$ .

### 4. Calculation of the secret-key rate $R$

- Calculate  $R$  using Eq. (S47) for each km.
- Plot  $R$  as a function of distance. To plot  $R$  in bits per second, multiply  $R$  by the repetition rate.

## Supplementary Tables

Table S1. List of random variables by order of appearance in the Supplementary Information.

| Variable                         | Protocol                      | Definition                                                                                                                                                                                                            |
|----------------------------------|-------------------------------|-----------------------------------------------------------------------------------------------------------------------------------------------------------------------------------------------------------------------|
| $N$                              | All                           | Total number of transmitted rounds                                                                                                                                                                                    |
| $N_{\text{key}}^{\text{det}}$    | Actual and Virtual            | Length of the sifted key                                                                                                                                                                                              |
| $N_j^{\beta X}$                  | Actual                        | Number of events in which Alice selects the setting $j$ and Bob obtains the $X$ -basis measurement outcome $\beta$ with $\beta \in \{0, 1\}$                                                                          |
| $e_{\text{ph}}$                  | Virtual                       | Phase-error rate                                                                                                                                                                                                      |
| $N_{\text{ph}}$                  | Virtual                       | Number of phase errors                                                                                                                                                                                                |
| $N_{\text{vir}\alpha}^{\beta X}$ | Virtual                       | Number of events in which Alice emits the state $ \psi_{\text{vir}\alpha}\rangle_B$ and Bob obtains the $X$ -basis measurement outcome $\beta$ with $\alpha, \beta \in \{0, 1\}$                                      |
| $N_{Z_C=z}^{\text{err}}$         | Coin                          | Number of events in which Alice chooses the $Z$ basis to measure the coin system $C$ , obtains the result $Z_C = z$ with $z \in \{0, 1\}$ , and Alice and Bob obtain the outcome associated to $\hat{m}_{\text{err}}$ |
| $N_{X_C=z}$                      | Coin                          | Number of events in which Alice obtains the outcome $X_C = z$ with $z \in \{0, 1\}$ in her $X$ -basis measurement of the coin system $C$                                                                              |
| $N_l^{\beta X}$                  | Virtual                       | Number of events $l$ in which Bob obtains the $X$ -basis measurement outcome $\beta$ with $\beta \in \{0, 1\}$                                                                                                        |
| $N_{l,t,Z_C}^{\beta X}$          | Virtual (with tag assignment) | Number of events $l$ with tag $t$ marked as $Z_C$ in which Bob obtains the $X$ -basis measurement outcome $\beta$ with $\beta \in \{0, 1\}$                                                                           |
| $N_l^{\text{det}}$               | Virtual                       | Number of detected events $l$                                                                                                                                                                                         |
| $N_{l,t,Z_C}^{\text{det}}$       | Virtual (with tag assignment) | Number of detected events $l$ with tag $t$ marked as $Z_C$                                                                                                                                                            |
| $N_{Z_C=z}^{\text{det}}$         | Coin                          | Number of detected events in which Alice chooses $Z_C$ and obtains the outcome $Z_C = z$ with $z \in \{0, 1\}$                                                                                                        |
| $N_{Z_C=z,D=d,A=a}^{\beta X}$    | Coin                          | Number of events in which Alice obtains $Z_C = z$ , $D = d$ , $A = a$ and Bob obtains the $X$ -basis measurement outcome $\beta$ with $z, d, a, \beta \in \{0, 1\}$                                                   |
| $N^{\text{det}}$                 | All                           | Number of detected rounds                                                                                                                                                                                             |
| $N_{ij}$                         | Actual                        | Number of events in which Alice (Bob) selects the setting $i(j)$                                                                                                                                                      |
| $N_{X_C=z}^{\text{det}}$         | Coin                          | Number of detected events in which Alice obtains the outcome $X_C = z$ with $z \in \{0, 1\}$ in her $X$ -basis measurement of the coin system $C$                                                                     |

Table S2. List of probabilities by order of appearance in the Supplementary Information.

| Variable                         | Protocol                      | Definition                                                                                                                                     |
|----------------------------------|-------------------------------|------------------------------------------------------------------------------------------------------------------------------------------------|
| $p_{\gamma_A}$                   | Actual                        | Probability that Alice selects the $\gamma$ -basis with $\gamma \in \{Z, X\}$                                                                  |
| $p_{\gamma_B}$                   | Actual                        | Probability that Bob measures in the $\gamma$ -basis with $\gamma \in \{Z, X\}$                                                                |
| $q_{\text{vir}_\alpha}^\psi$     | Virtual                       | Probability that Alice emits the virtual state $ \psi_{\text{vir}_\alpha}\rangle_B$ with $\alpha \in \{0, 1\}$                                 |
| $q_{\text{vir}_\alpha}^\phi$     | Virtual                       | Probability that Alice emits the virtual state $ \phi_{\text{vir}_\alpha}\rangle_B$ with $\alpha \in \{0, 1\}$                                 |
| $p_l$                            | Virtual                       | Probability of selecting the state associated to $l$                                                                                           |
| $p_{t l}$                        | Virtual (with tag assignment) | Probability of assigning a tag $t$ given an event $l$                                                                                          |
| $p_{\gamma_C}$                   | Coin                          | Probability that Alice measures the quantum coin system $C$ in the $\gamma_C$ basis with $\gamma \in \{Z, X\}$                                 |
| $p_t$                            | Virtual (with tag assignment) | Probability of assigning a tag $t$                                                                                                             |
| $p_{l t}$                        | Virtual (with tag assignment) | Probability of having selected the state associated to $l$ given a tag $t$                                                                     |
| $p_C$                            | Coin                          | Probability of selecting a coin round                                                                                                          |
| $p_{\text{key} Z}$               | Actual                        | Probability that a round is assigned to “key” given that the users announced the $Z$ basis                                                     |
| $p_{\text{test} Z}$              | Actual                        | Probability that a round is assigned to “test” given that the users announced the $Z$ basis                                                    |
| $q_{\text{vir}_\alpha}^{\psi,u}$ | Virtual                       | Probability that Alice ( $u = a$ )/Bob ( $u = b$ ) emits the virtual state $ \psi_{\text{vir}_\alpha}\rangle_{B_u}$ with $\alpha \in \{0, 1\}$ |
| $q_{\text{vir}_\alpha}^{\phi,u}$ | Virtual                       | Probability that Alice ( $u = a$ )/Bob ( $u = b$ ) emits the virtual state $ \phi_{\text{vir}_\alpha}\rangle_{B_u}$ with $\alpha \in \{0, 1\}$ |
| $p_{t_{\alpha\beta} t}$          | Virtual (with tag assignment) | Probability that a tag $t_{\alpha\beta}$ is assigned given a tag $t$ with $\alpha, \beta \in \{0, 1\}$                                         |
| $p_{\text{vir}_{\alpha\beta} t}$ | Virtual (with tag assignment) | Probability of having selected the state associated to $\text{vir}_{\alpha\beta}$ given a tag $t$ with $\alpha, \beta \in \{0, 1\}$            |

- 
- [S1] M. Pereira, M. Curty, and K. Tamaki, Quantum key distribution with flawed and leaky sources, *npj Quantum Inf* **5**, 62 (2019).
- [S2] M. Pereira, G. Kato, A. Mizutani, M. Curty, and K. Tamaki, Quantum key distribution with correlated sources, *Sci. Adv.* **6**, eaaz4487 (2020).
- [S3] L. Lydersen, C. Wiechers, C. Wittmann, D. Elser, J. Skaar, and V. Makarov, Hacking commercial quantum cryptography systems by tailored bright illumination, *Nature Photon* **4**, 686 (2010).
- [S4] I. Gerhardt, Q. Liu, A. Lamas-Linares, J. Skaar, C. Kurtsiefer, and V. Makarov, Full-field implementation of a perfect eavesdropper on a quantum cryptography system, *Nat Commun* **2**, 349 (2011).
- [S5] V. Makarov, Controlling passively quenched single photon detectors by bright light, *New J. Phys.* **11**, 065003 (2009).
- [S6] C. Wiechers, L. Lydersen, C. Wittmann, D. Elser, J. Skaar, C. Marquardt, V. Makarov, and G. Leuchs, After-gate attack on a quantum cryptosystem, *New J. Phys.* **13**, 013043 (2011).
- [S7] H.-K. Lo, M. Curty, and B. Qi, Measurement-Device-Independent Quantum Key Distribution, *Phys. Rev. Lett.* **108**, 130503 (2012).
- [S8] R. Renner, *Security of Quantum Key Distribution*, Ph.D. thesis, ETH Zurich (2005).
- [S9] M. Tomamichel and R. Renner, Uncertainty Relation for Smooth Entropies, *Phys. Rev. Lett.* **106**, 110506 (2011).
- [S10] M. Tomamichel, C. C. W. Lim, N. Gisin, and R. Renner, Tight finite-key analysis for quantum cryptography, *Nat Commun* **3**, 634 (2012).
- [S11] D. Mayers, Quantum key distribution and string oblivious transfer in noisy channels, in *Adv. Cryptol. — CRYPTO 96*, edited by N. Kobitz (Springer Berlin Heidelberg, Berlin, Heidelberg, 1996) pp. 343–357.
- [S12] P. W. Shor and J. Preskill, Simple Proof of Security of the BB84 Quantum Key Distribution Protocol, *Phys. Rev. Lett.* **85**, 441 (2000).
- [S13] M. Koashi, Simple security proof of quantum key distribution based on complementarity, *New J. Phys.* **11**, 045018 (2009).
- [S14] K. Tamaki, M. Curty, G. Kato, H.-K. Lo, and K. Azuma, Loss-tolerant quantum cryptography with imperfect sources, *Phys. Rev. A* **90**, 052314 (2014).
- [S15] G. Currás-Lorenzo, Á. Navarrete, M. Pereira, and K. Tamaki, Finite-key analysis of loss-tolerant quantum key distribution based on random sampling theory, *Phys. Rev. A* **104**, 012406 (2021).
- [S16] H. Chernoff, A Measure of Asymptotic Efficiency for Tests of a Hypothesis Based on the sum of Observations, *Ann. Math. Stat.* **23**, 493 (1952).
- [S17] K. Tamaki, M. Curty, and M. Lucamarini, Decoy-state quantum key distribution with a leaky source, *New J. Phys.* **18**, 065008 (2016).
- [S18] W. Wang, K. Tamaki, and M. Curty, Finite-key security analysis for quantum key distribution with leaky sources, *New J. Phys.* **20**, 083027 (2018).
- [S19] W. Wang, K. Tamaki, and M. Curty, Measurement-device-independent quantum key distribution with leaky sources, *Sci Rep* **11**, 1678 (2021).
- [S20] M. Pereira, G. Currás-Lorenzo, Á. Navarrete, A. Mizutani, G. Kato, M. Curty, and K. Tamaki, Modified BB84 quantum key distribution protocol robust to source imperfections, *Phys. Rev. Res.* **5**, 023065 (2023).
- [S21] I. D. Ivanovic, How to differentiate between non-orthogonal states, *Physics Letters A* **123**, 257 (1987).
- [S22] H.-K. Lo and J. Preskill, Security of quantum key distribution using weak coherent states with nonrandom phases, *Quantum Inf. Comput.* **7**, 431 (2007).
- [S23] W. Hoeffding, Probability inequalities for sums of bounded random variables, *J. Am. Stat. Assoc.* **58**, 13 (1963).
- [S24] K. Azuma, Weighted sums of certain dependent random variables, *Tohoku Math. J.* **19**, 357 (1967).
- [S25] G. Kato, Concentration inequality using unconfirmed knowledge (2020), [arxiv:2002.04357 \[quant-ph\]](https://arxiv.org/abs/2002.04357).
- [S26] M. Hayashi and T. Tsurumaru, Concise and tight security analysis of the Bennett–Brassard 1984 protocol with finite key lengths, *New J. Phys.* **14**, 093014 (2012).
- [S27] G. Currás-Lorenzo, Á. Navarrete, K. Azuma, G. Kato, M. Curty, and M. Razavi, Tight finite-key security for twin-field quantum key distribution, *npj Quantum Inf* **7**, 22 (2021).
- [S28] D. Tupkary, S. Nahar, P. Sinha, and N. Lütkenhaus, Phase error rate estimation with basis-efficiency mismatch for decoy-state BB84 (2024), [arXiv:2408.17349 \[quant-ph\]](https://arxiv.org/abs/2408.17349).
- [S29] F. Xu, X. Ma, Q. Zhang, H.-K. Lo, and J.-W. Pan, Secure quantum key distribution with realistic devices, *Rev. Mod. Phys.* **92**, 025002 (2020).
- [S30] M. Pittaluga, M. Minder, M. Lucamarini, M. Sanzaro, R. I. Woodward, M.-J. Li, Z. Yuan, and A. J. Shields, 600-km repeater-like quantum communications with dual-band stabilization, *Nat. Photon.* **15**, 530 (2021).
- [S31] Á. Navarrete and M. Curty, Improved finite-key security analysis of quantum key distribution against Trojan-horse attacks, *Quantum Sci. Technol.* **7**, 035021 (2022).
- [S32] T. Honjo, K. Inoue, and H. Takahashi, Differential-phase-shift quantum key distribution experiment with a planar light-wave circuit Mach–Zehnder interferometer, *Opt. Lett.* **29**, 2797 (2004).
- [S33] F. Xu, K. Wei, S. Sajeed, S. Kaiser, S. Sun, Z. Tang, L. Qian, V. Makarov, and H.-K. Lo, Experimental quantum key distribution with source flaws, *Phys. Rev. A* **92**, 032305 (2015).
- [S34] Á. Navarrete, M. Pereira, M. Curty, and K. Tamaki, Practical Quantum Key Distribution That is Secure Against Side Channels, *Phys. Rev. Applied* **15**, 034072 (2021).
- [S35] D. Gottesman, H.-K. Lo, N. Lütkenhaus, and J. Preskill, Security of quantum key distribution with imperfect devices,

Quantum Inf. Comput. **4**, 325 (2004).

- [S36] A. Mizutani, G. Kato, K. Azuma, M. Curty, R. Ikuta, T. Yamamoto, N. Imoto, H.-K. Lo, and K. Tamaki, Quantum key distribution with setting-choice-independently correlated light sources, *Npj Quantum Inf.* **5**, 8 (2019).
- [S37] A. Mizutani and G. Kato, Security of round-robin differential-phase-shift quantum-key-distribution protocol with correlated light sources, *Phys. Rev. A* **104**, 062611 (2021).
- [S38] K.-i. Yoshino, M. Fujiwara, K. Nakata, T. Sumiya, T. Sasaki, M. Takeoka, M. Sasaki, A. Tajima, M. Koashi, and A. Tomita, Quantum key distribution with an efficient countermeasure against correlated intensity fluctuations in optical pulses, *npj Quantum Inf.* **4**, 1 (2018).
- [S39] M. Pereira, G. Currás-Lorenzo, A. Mizutani, D. Rusca, M. Curty, and K. Tamaki, Quantum key distribution with unbounded pulse correlations (2024), [arxiv:2402.08028 \[quant-ph\]](#).
- [S40] F. Grünenfelder, A. Boaron, D. Rusca, A. Martin, and H. Zbinden, Performance and security of 5 GHz repetition rate polarization-based quantum key distribution, *Appl. Phys. Lett.* **117**, 144003 (2020).
- [S41] W.-Y. Hwang, Quantum key distribution with high loss: Toward global secure communication, *Phys. Rev. Lett.* **91**, 057901 (2003).
- [S42] H.-K. Lo, X. Ma, and K. Chen, Decoy State Quantum Key Distribution, *Phys. Rev. Lett.* **94**, 230504 (2005).
- [S43] X.-B. Wang, Beating the Photon-Number-Splitting Attack in Practical Quantum Cryptography, *Phys. Rev. Lett.* **94**, 230503 (2005).
- [S44] M. Curty, F. Xu, W. Cui, C. C. W. Lim, K. Tamaki, and H.-K. Lo, Finite-key analysis for measurement-device-independent quantum key distribution, *Nat Commun* **5**, 3732 (2014).
- [S45] C. C. W. Lim, M. Curty, N. Walenta, F. Xu, and H. Zbinden, Concise security bounds for practical decoy-state quantum key distribution, *Phys. Rev. A* **89**, 022307 (2014).
- [S46] V. Zapatero, Á. Navarrete, K. Tamaki, and M. Curty, Security of quantum key distribution with intensity correlations, *Quantum* **5**, 602 (2021).
- [S47] X. Sixto, V. Zapatero, and M. Curty, Security of Decoy-State Quantum Key Distribution with Correlated Intensity Fluctuations, *Phys. Rev. Applied* **18**, 044069 (2022).
- [S48] S. Nahar, T. Upadhyaya, and N. Lütkenhaus, Imperfect Phase-Randomisation and Generalised Decoy-State Quantum Key Distribution (2023), [arxiv:2304.09401 \[quant-ph\]](#).
- [S49] X. Sixto, G. Currás-Lorenzo, K. Tamaki, and M. Curty, Secret key rate bounds for quantum key distribution with faulty active phase randomization, *EPJ Quantum Technol.* **10**, 1 (2023).
- [S50] G. Currás-Lorenzo, S. Nahar, N. Lütkenhaus, K. Tamaki, and M. Curty, Security of quantum key distribution with imperfect phase randomisation, *Quantum Sci. Technol.* **9**, 015025 (2023).
- [S51] M. Sandfuchs, M. Haberland, V. Vilasini, and R. Wolf, Security of differential phase shift QKD from relativistic principles (2023), [arxiv:2301.11340 \[quant-ph\]](#).
